# Supplementary material for: ManiFlow: Implicitly Representing Manifolds with Normalizing Flows
Source: arXiv:2208.08932 source file (2022-08-18)
Supplement: Supplementary file 1 [file supplement.tex]

% Content of the supplement:
% \begin{itemize}
%     \item \ding{51} Code submission
%     \item \ding{51} More qualitative examples of PCs
%     \item \ding{51} Ablation of hyperparameters
%     \item \ding{51} Qualitative examples of created mesh
%     \item \ding{51} Additional toy example regarding importance of small $\sigma$ and regularization term
%     \item \ding{51} Experimental details
%     \item \ding{51} Optional: Proof that gradient is perpendicular to surface and surface equals the region of maximum likelihood under our assumptions
% \end{itemize}

\begin{figure*}[t!]
\begin{center}

    \renewcommand{\figsize}{0.16}
    
    \begin{tabular}{ c c c c c }
    
        \centering 
    
        GT & GT + Noise & NF & LLM, $\lambda=0.0$ & LLM, $\lambda=0.2$ \\
        
      \includegraphics[width=\figsize\linewidth]{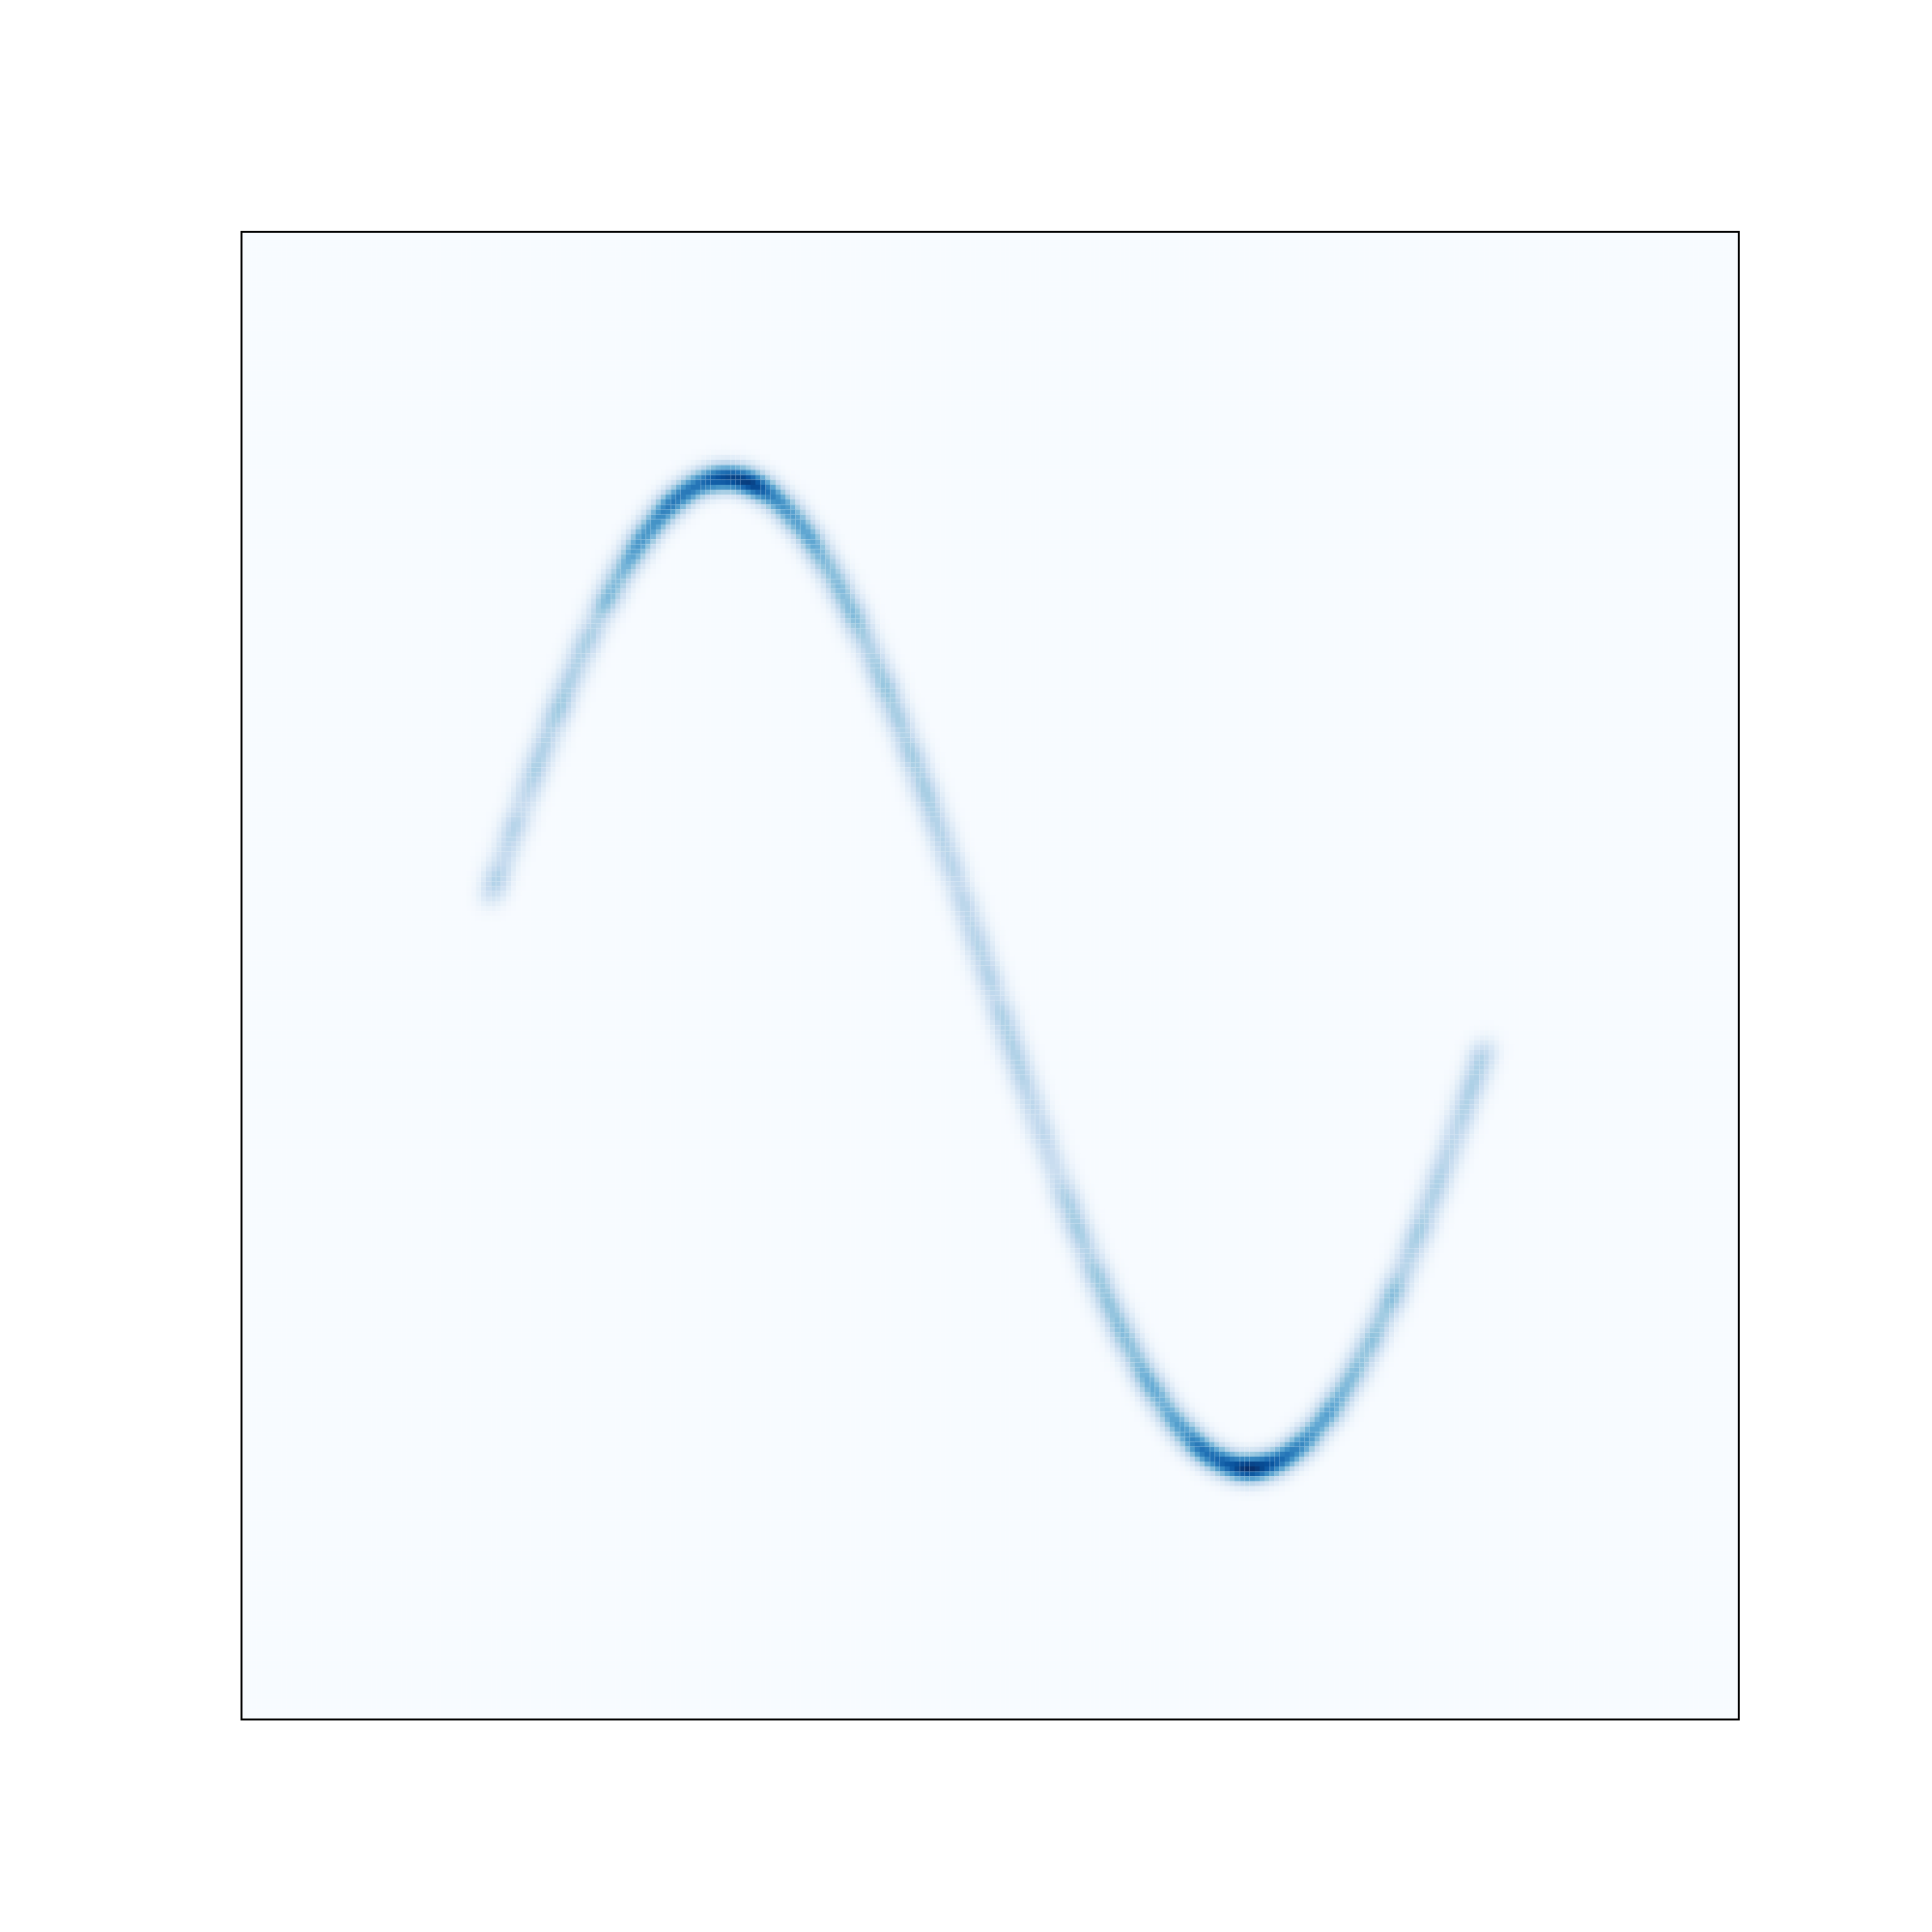} &
      \includegraphics[width=\figsize\linewidth]{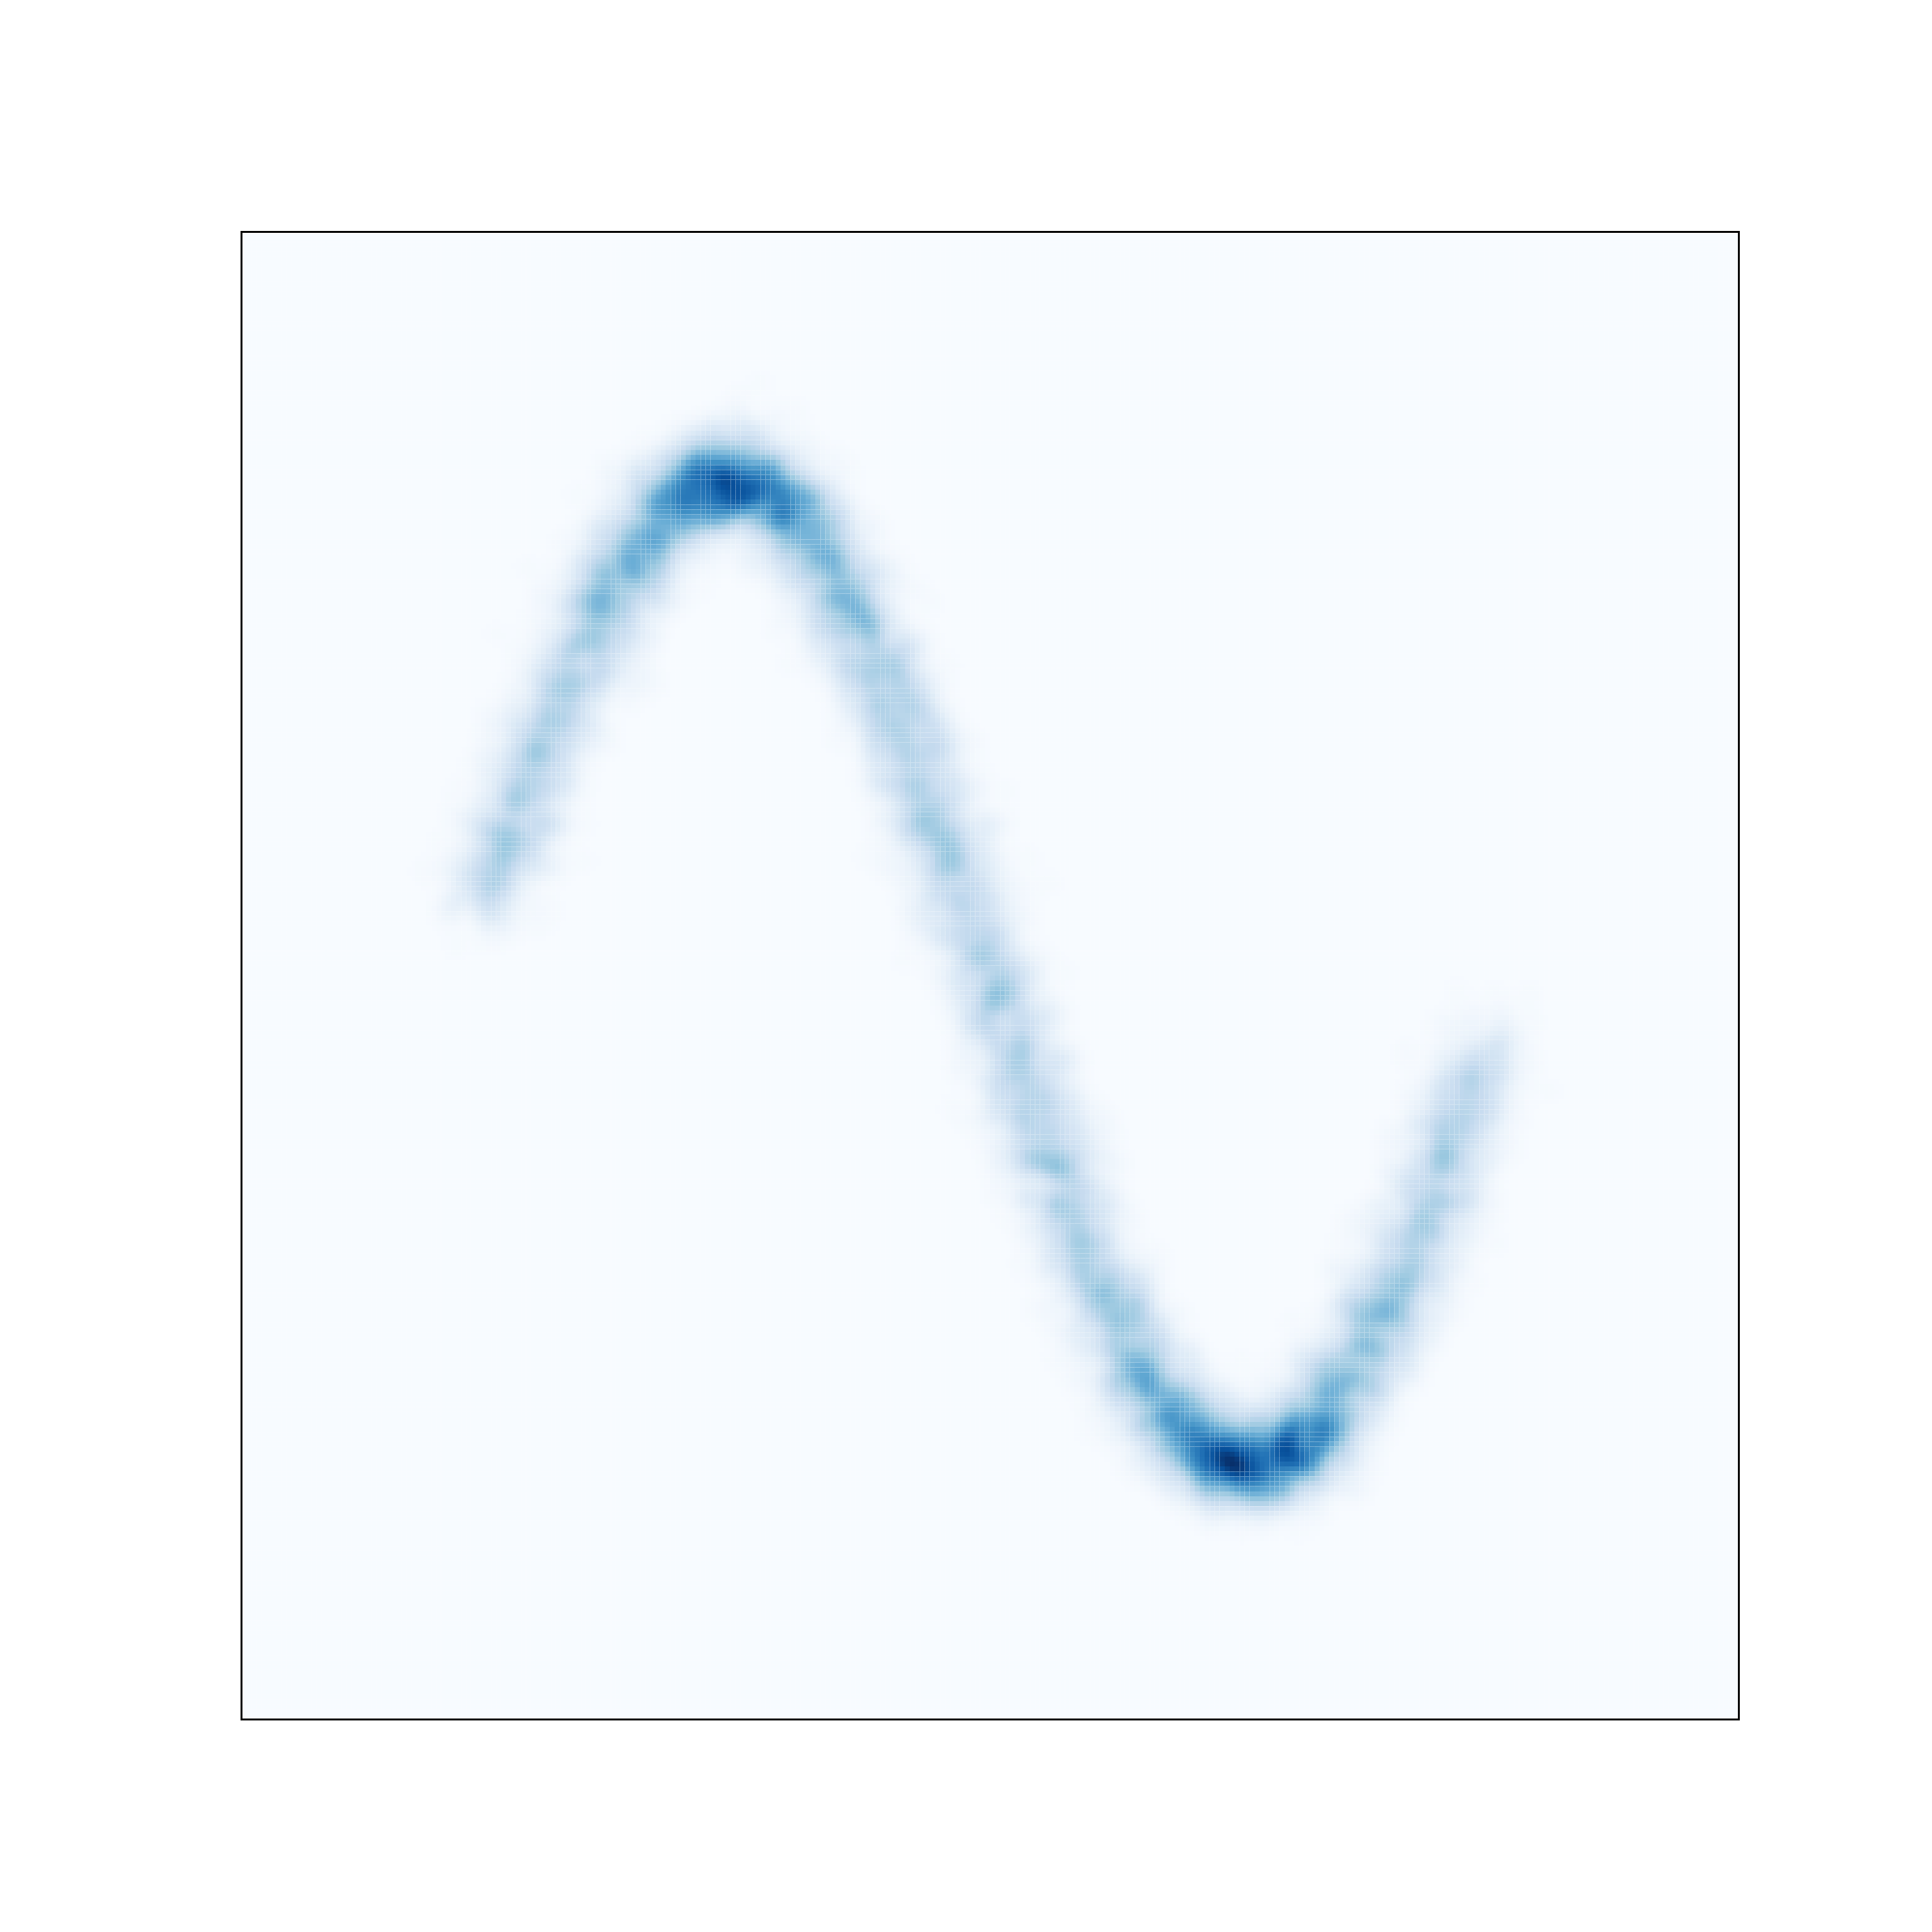} &
      \includegraphics[width=\figsize\linewidth]{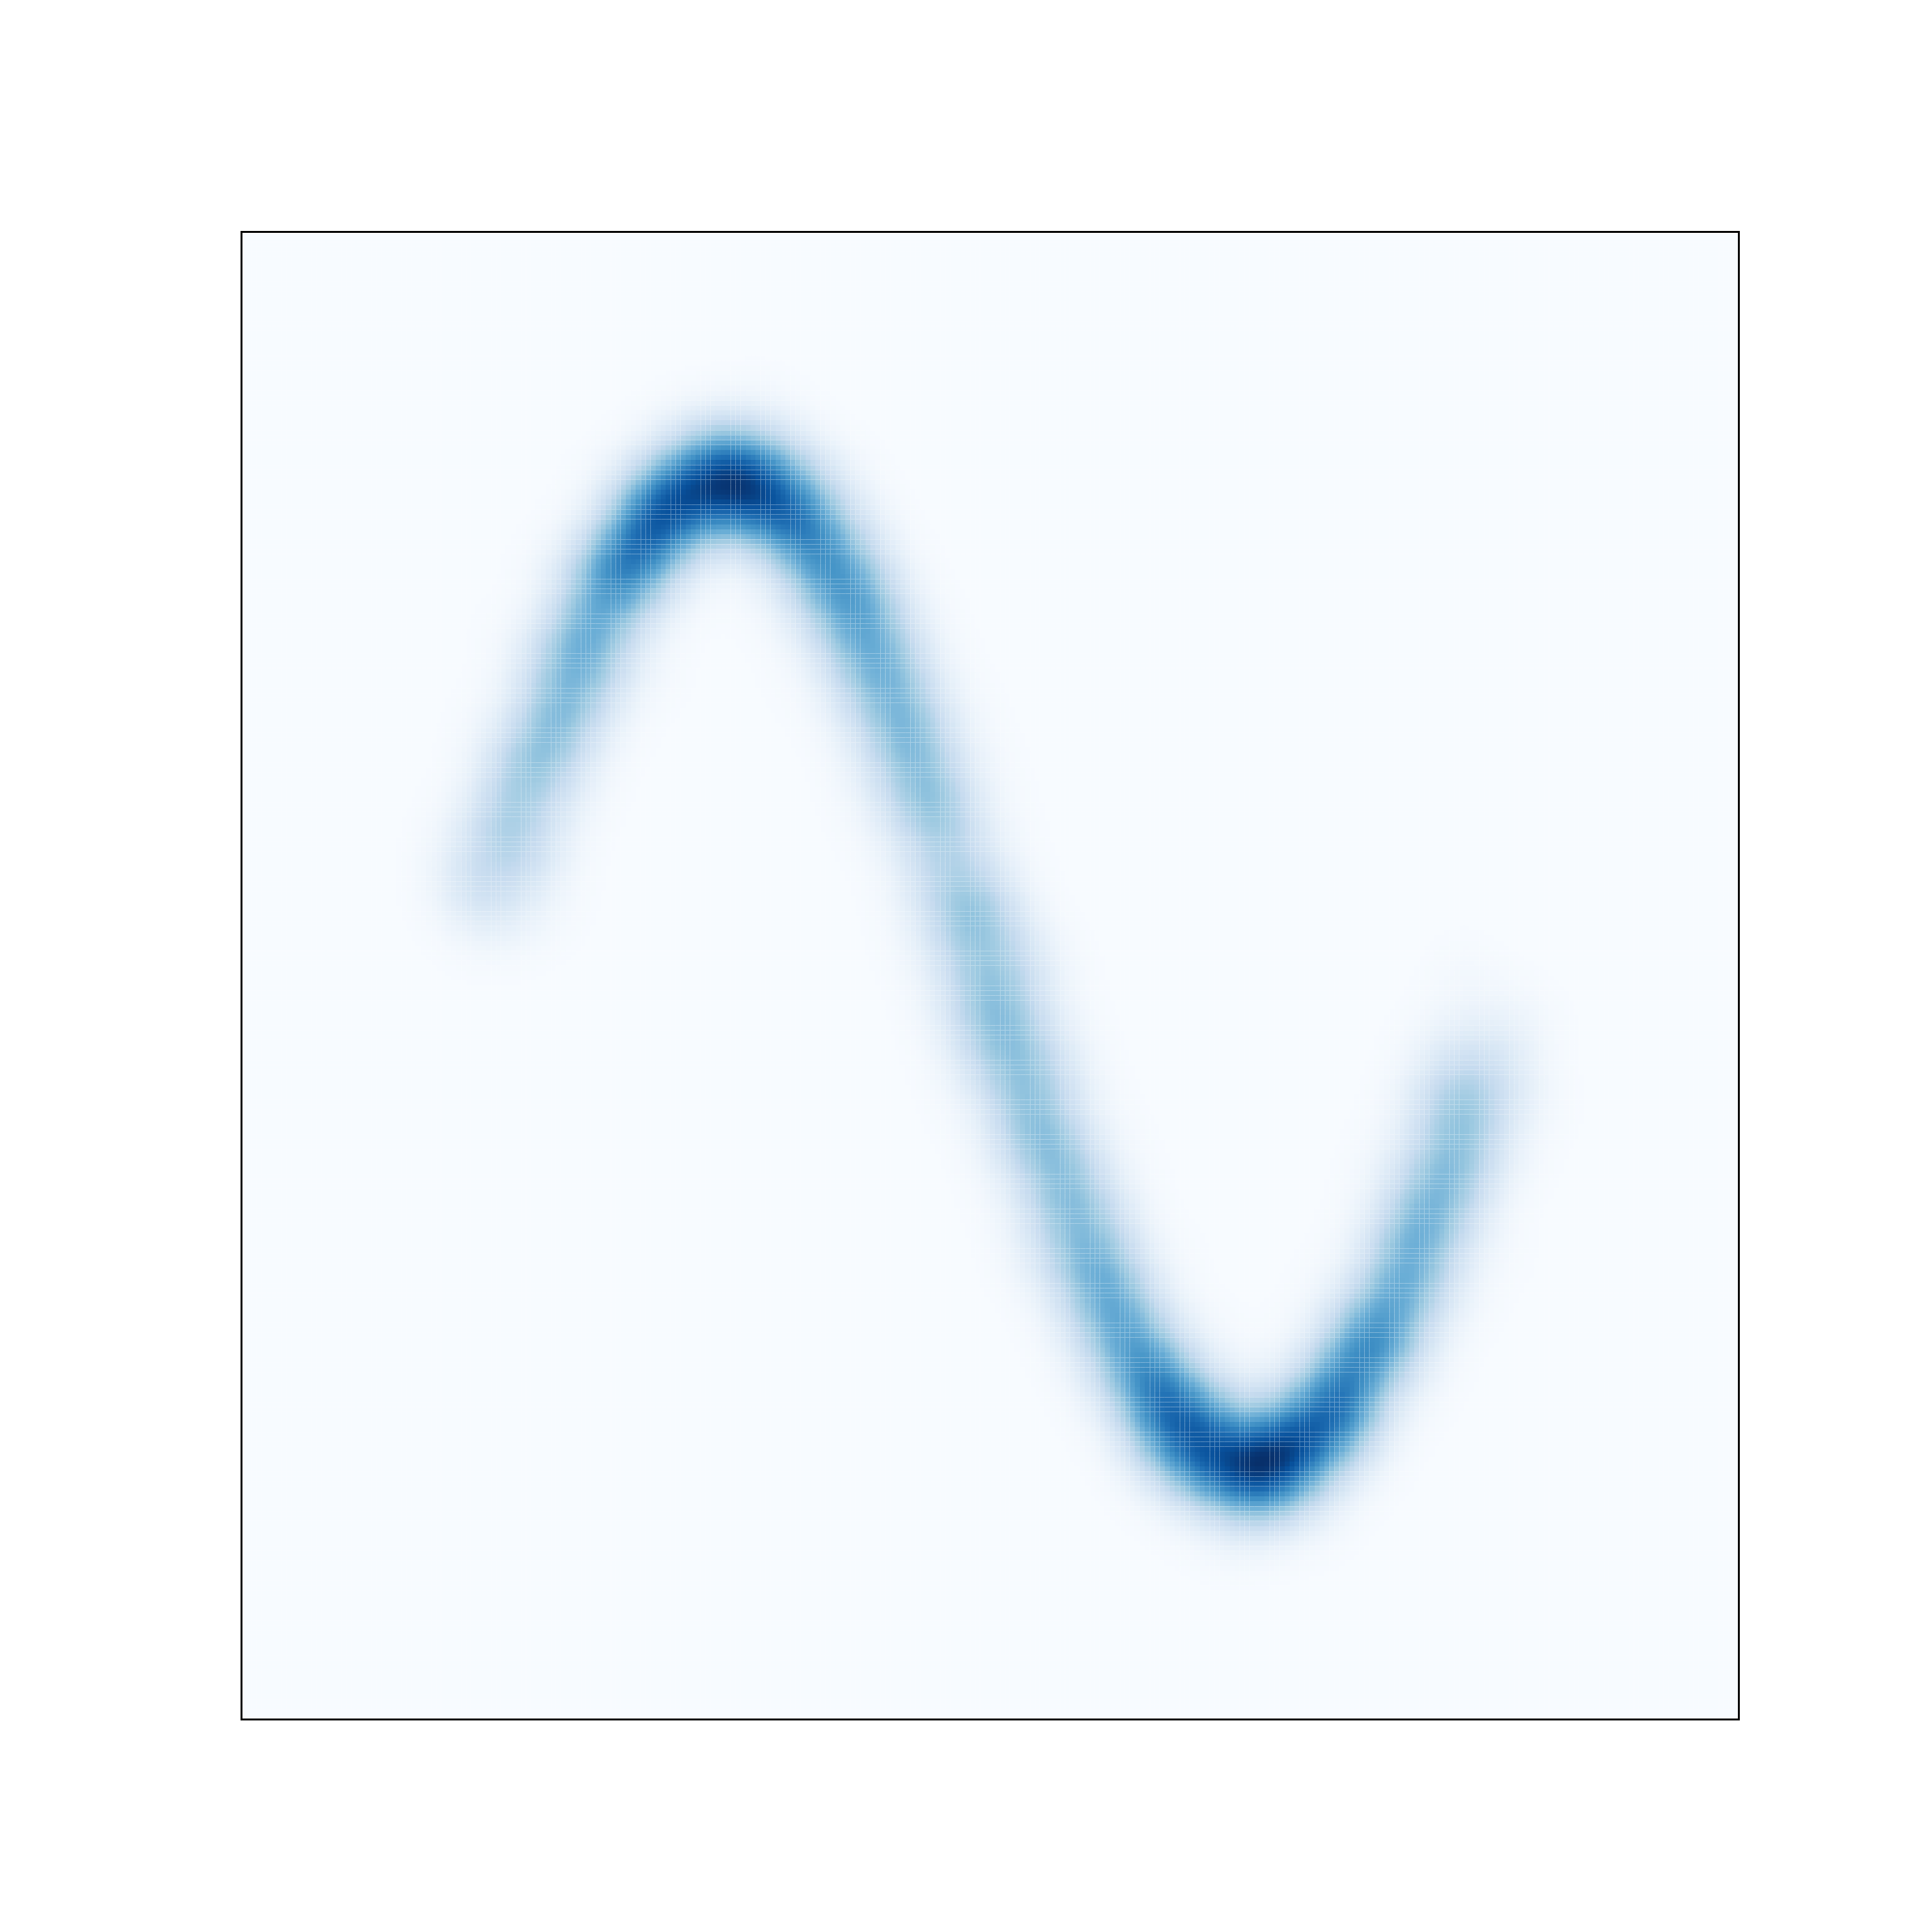} &
      \includegraphics[width=\figsize\linewidth]{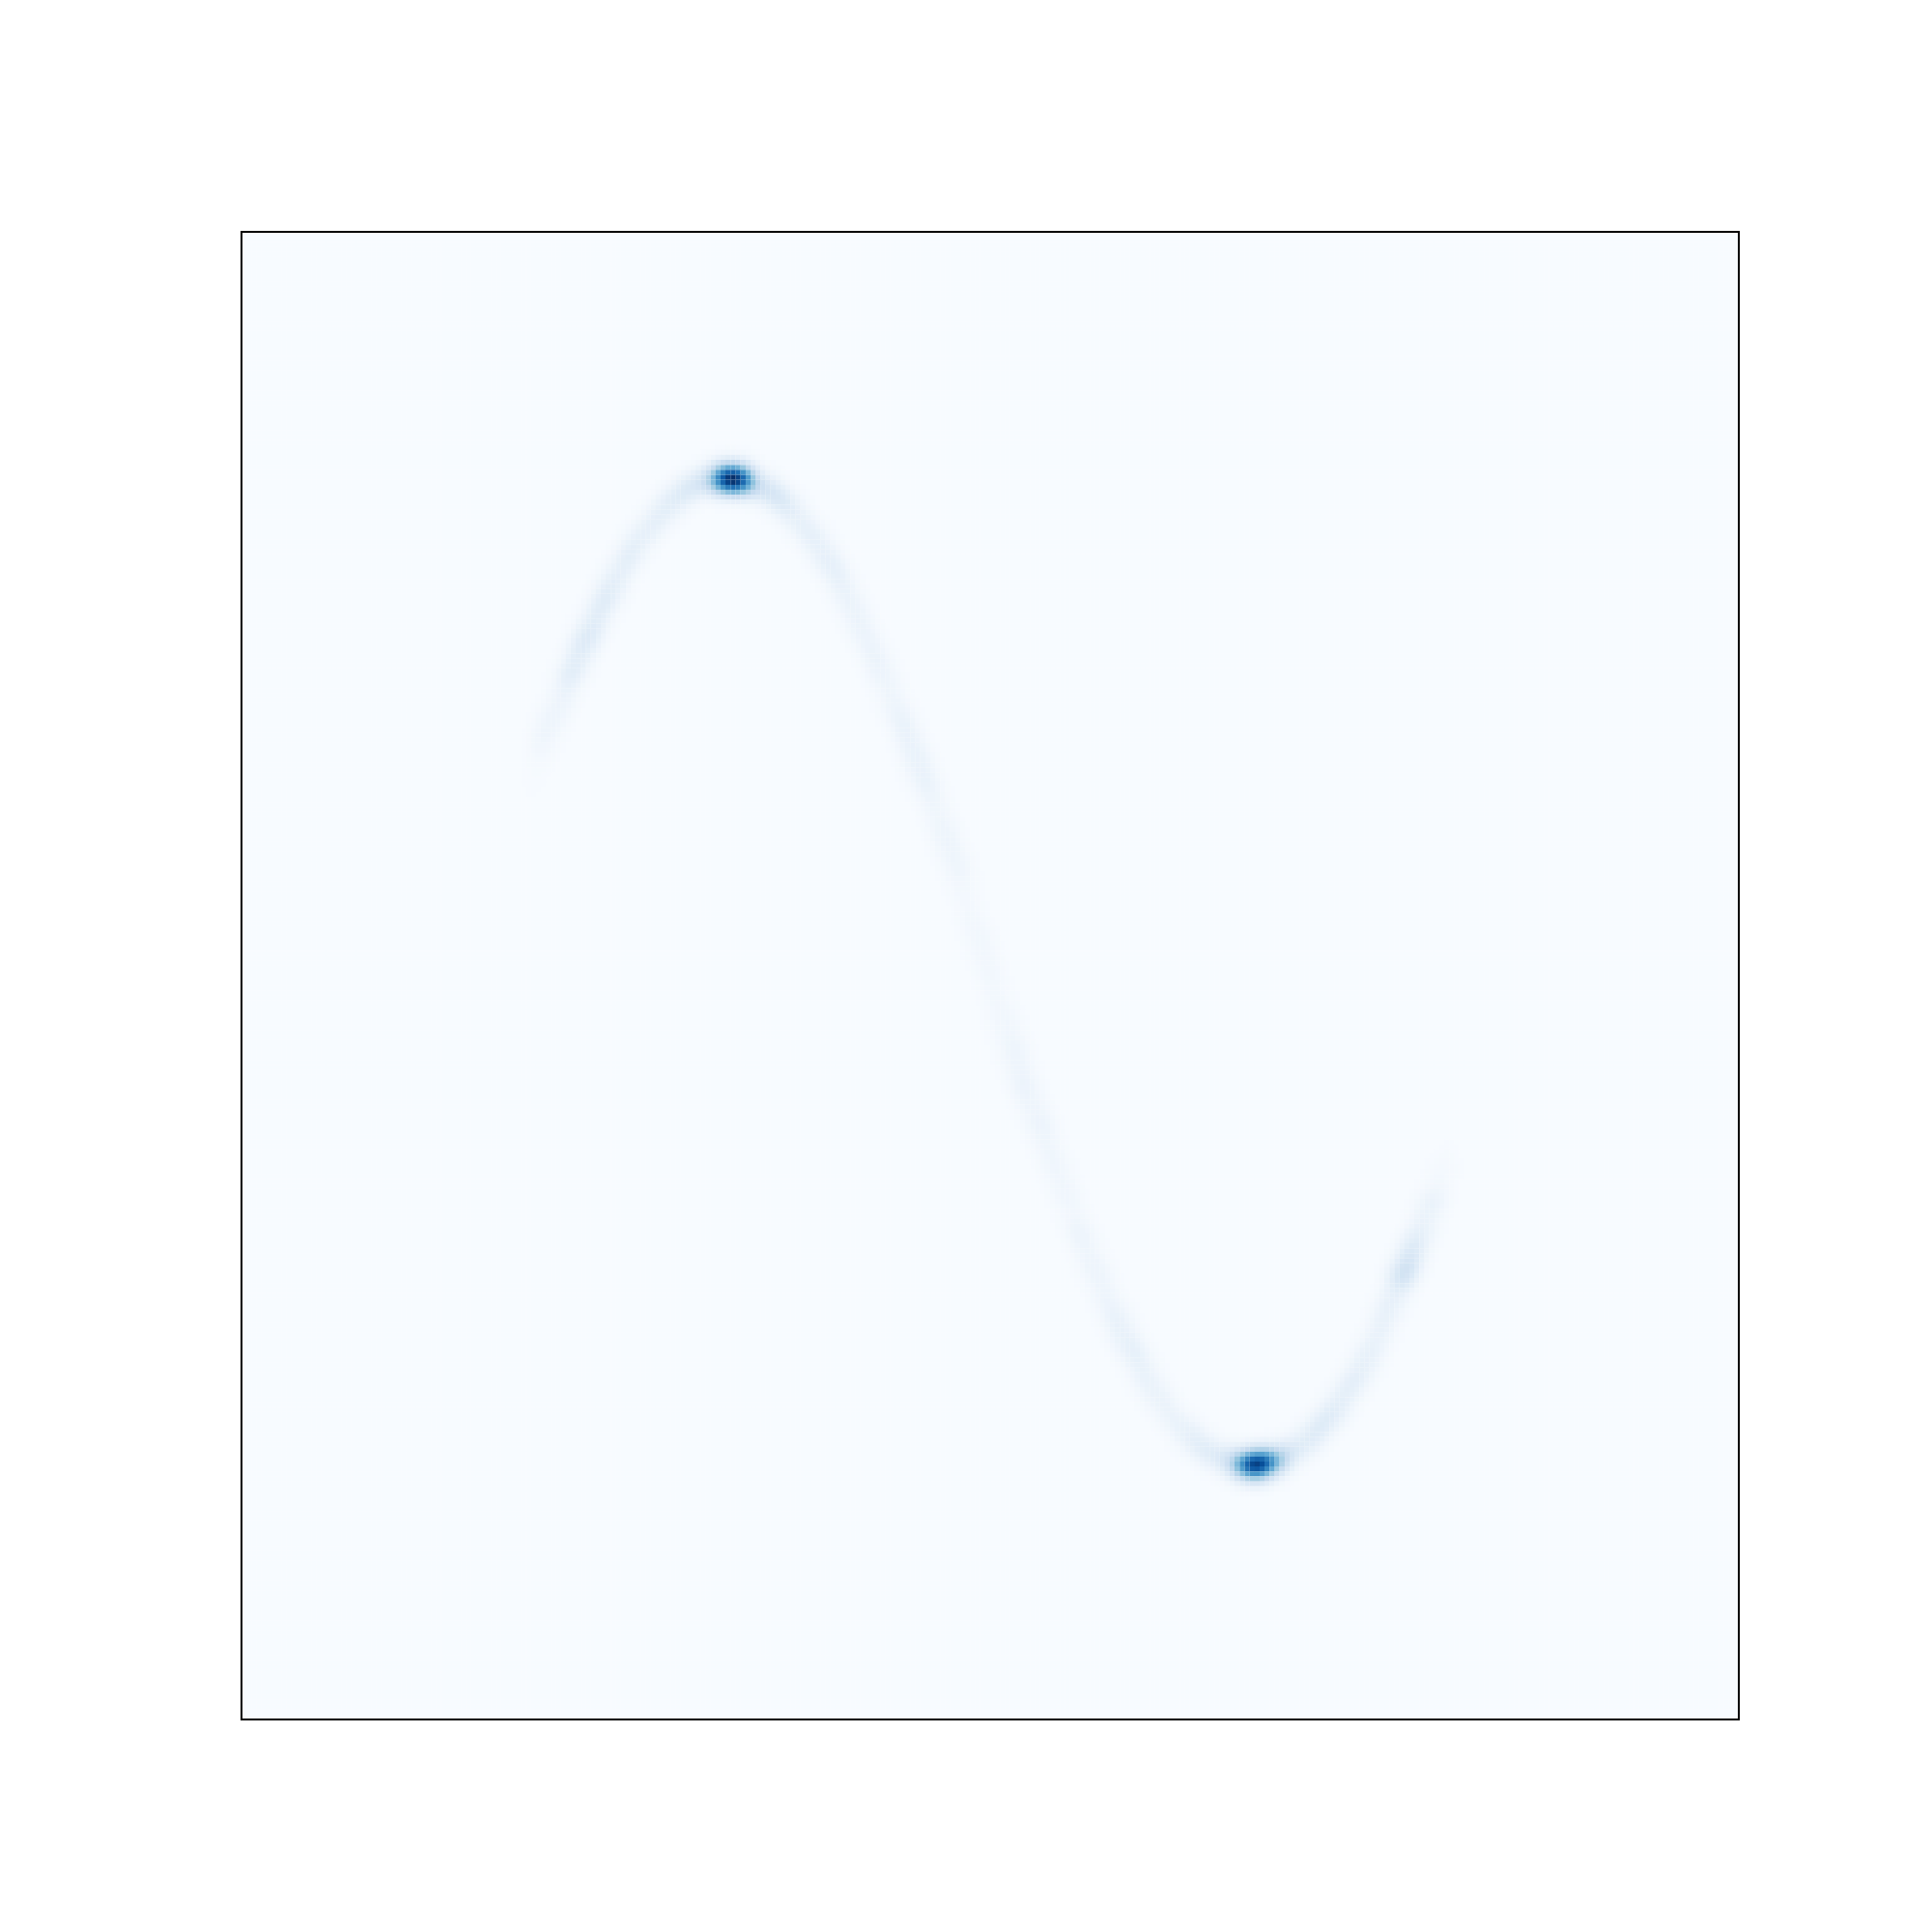} &
      \includegraphics[width=\figsize\linewidth]{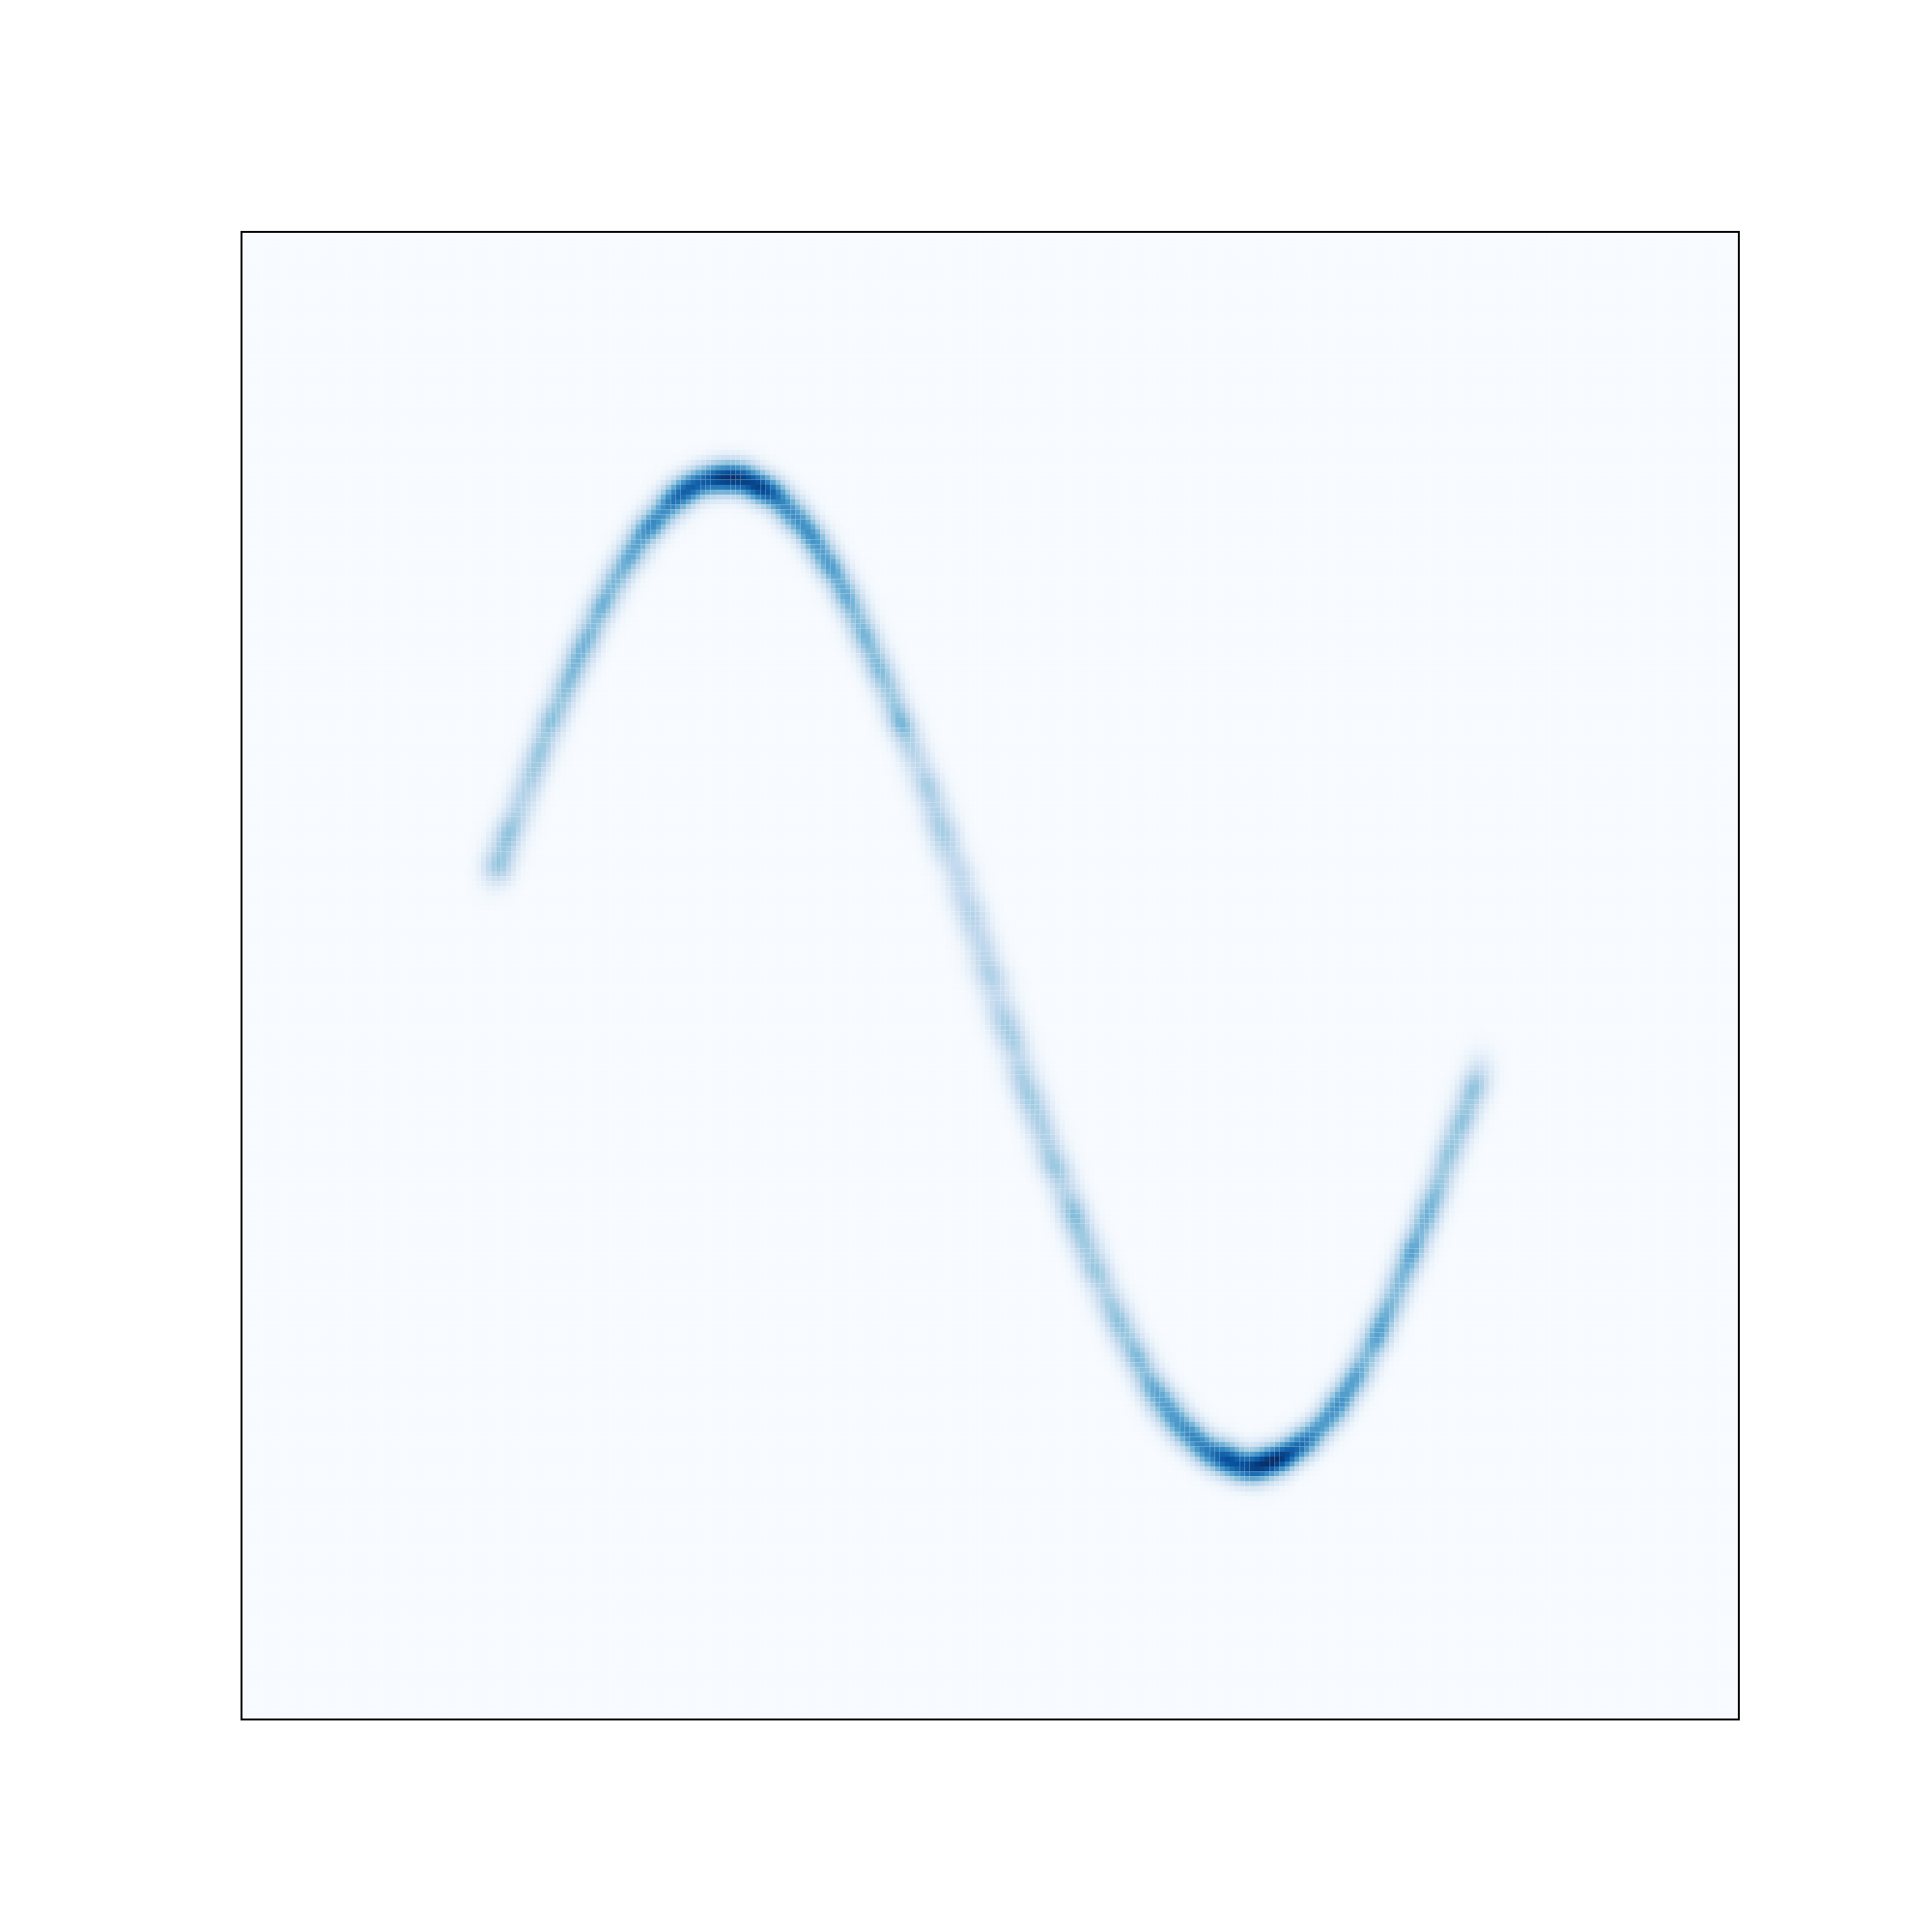} \\

    \end{tabular}
    
\end{center}
\caption{In this experiment, we learn a non-uniform distribution (GT, GT + Noise) that exists on a 1D sine curve in 2D using a \ac{nf}. We demonstrate the importance of the regularization parameter $\lambda$. In absence of regularization ($\lambda =0$) LLM is not able to recover the correct distribution on the sine curve. However, using $\lambda = 0.2$ recovers the correct distribution.}\label{fig:toy_example_regularization}
\end{figure*}

We conduct an additional experiment on artificial data to provide intuition about ManiFlow in \secref{suppl_sec:toy_examples}. Then, we analyse the impact of hyperparameters used by ManiFlow - LLM/LL-Poisson in \secref{suppl_sec:ablation}. In \secref{suppl_sec:vis_pcs}, \secref{suppl_sec:vis_meshes} and \secref{suppl_sec:gen_imgs}, we depict additional qualitative examples of reconstructed point clouds, visualize the meshes obtained using LL-Poisson and show qualitative examples of generated image. Finally, we show properties assumed about the log-likelihood of \acp{nf} in \secref{subsection:sampling_manifold} in \secref{suppl_sec:proof} and provide additional details about the architecture and optimization procedure used in the experiments in \secref{suppl_sec:exp_details}.

\subsection{Additional Experiments of Artifical Data}\label{suppl_sec:toy_examples}

We provide an additional experiment on artificial data showing the importance of setting $\lambda>0$ in \eref{eq:optimization_criterion}. To this end, we train a \ac{nf} on a non-uniform distribution on a 1D sine curve embedded in 2D space. After training, we recover the manifold using ManiFlow - LLM using $\lambda=0.0$ and $\lambda=0.2$. The results are in \figref{fig:toy_example_regularization}. We observe that $\lambda=0.0$ fails to recover the true distribution on the manifold since generated points collapse towards global peaks of the distribution parameterized by the \ac{nf}.

\subsection{Impact of Hyperparameters}\label{suppl_sec:ablation}

We analyse the sensitivity of LLM/LL-Poisson to its hyperparameters. We perform this anaysis on the task of point cloud autoencoding and use the RealNVP trained on the airplane category in \secref{subsection:pc_autoencoding}. For LLM we plot the F1-score against the number of epochs used to optimize \eref{eq:optimization_criterion} and the logarithm of the magnitude of the weight $\lambda$. For LL-Poisson we plot the F1-score against the depth used for Poisson surface reconstruction and the logarithm of the number of points K\textsubscript{1} sampled prior to surface reconstruction. \figref{fig:llm_ablation} and \figref{fig:llpoisson_ablation} depict the results. While there exists an optimal $\lambda$, we find that the other hyperparameters typically lead to saturating performance given a sufficient magnitude.

\begin{figure}[t!]
\centering
\begin{subfigure}{.49\textwidth}
  \centering
  \includegraphics[width=1.0\linewidth]{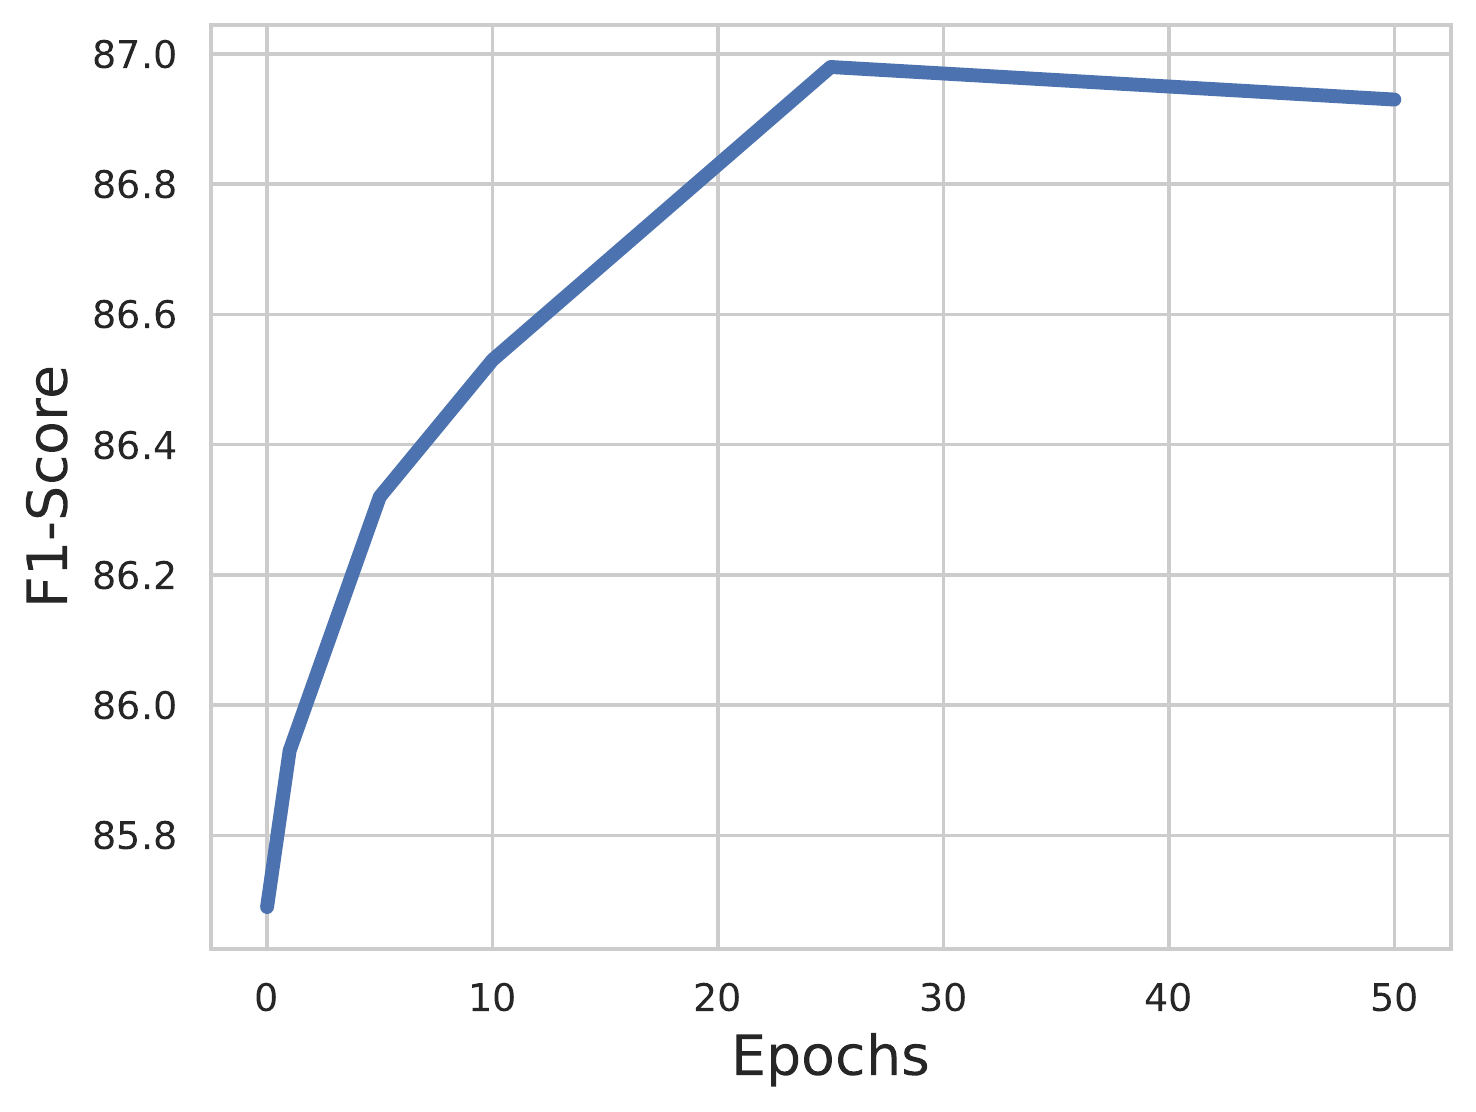}
  \caption{F1-Score depending on the number of epochs used for ManiFlow-LLM.}.
  \label{fig:f1_vs_epochs}
\end{subfigure}%
\\
\begin{subfigure}{.49\textwidth}
  \centering
  \includegraphics[width=1.0\linewidth]{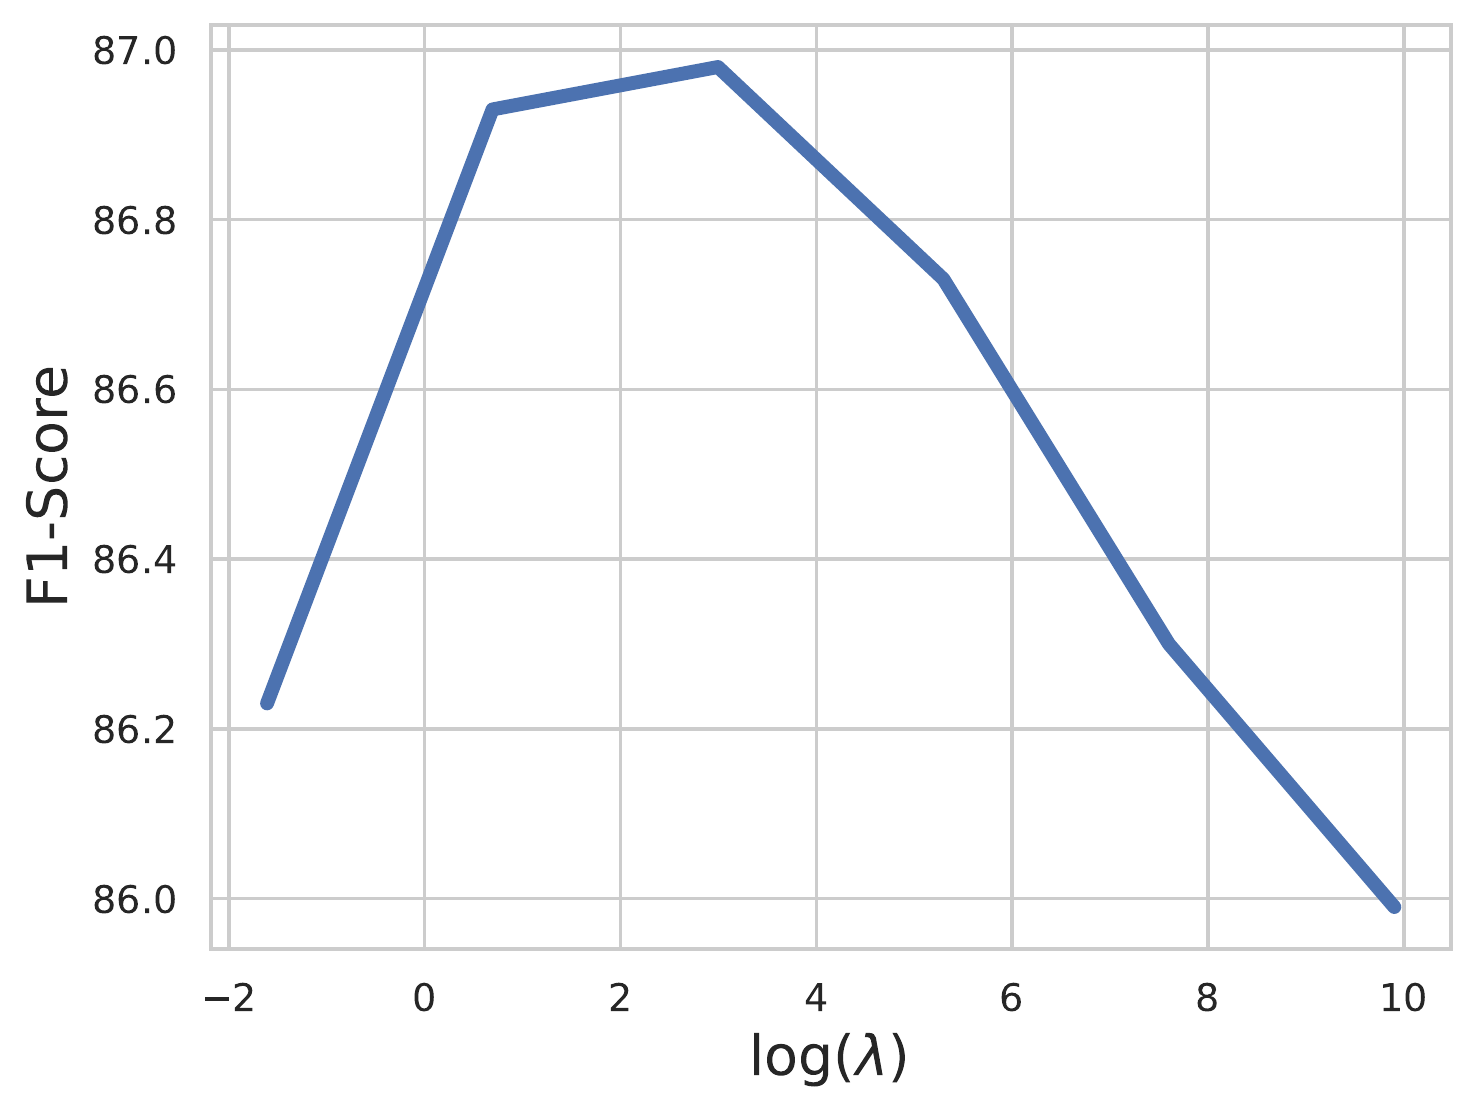}
  \caption{F1-Score depending on the on the logarithm of the weight $\lambda$ used for ManiFlow-LLM.}
  \label{fig:f1_vs_dweight}
\end{subfigure}
\caption{Analysis of the sensitivity of ManiFlow-LLM to the number of epochs (a) and the magnitude of $\lambda$ (b) on the airplane category.}
\label{fig:llm_ablation}
\end{figure}

\begin{figure}
\centering
\begin{subfigure}{.49\textwidth}
  \centering
  \includegraphics[width=1.0\linewidth]{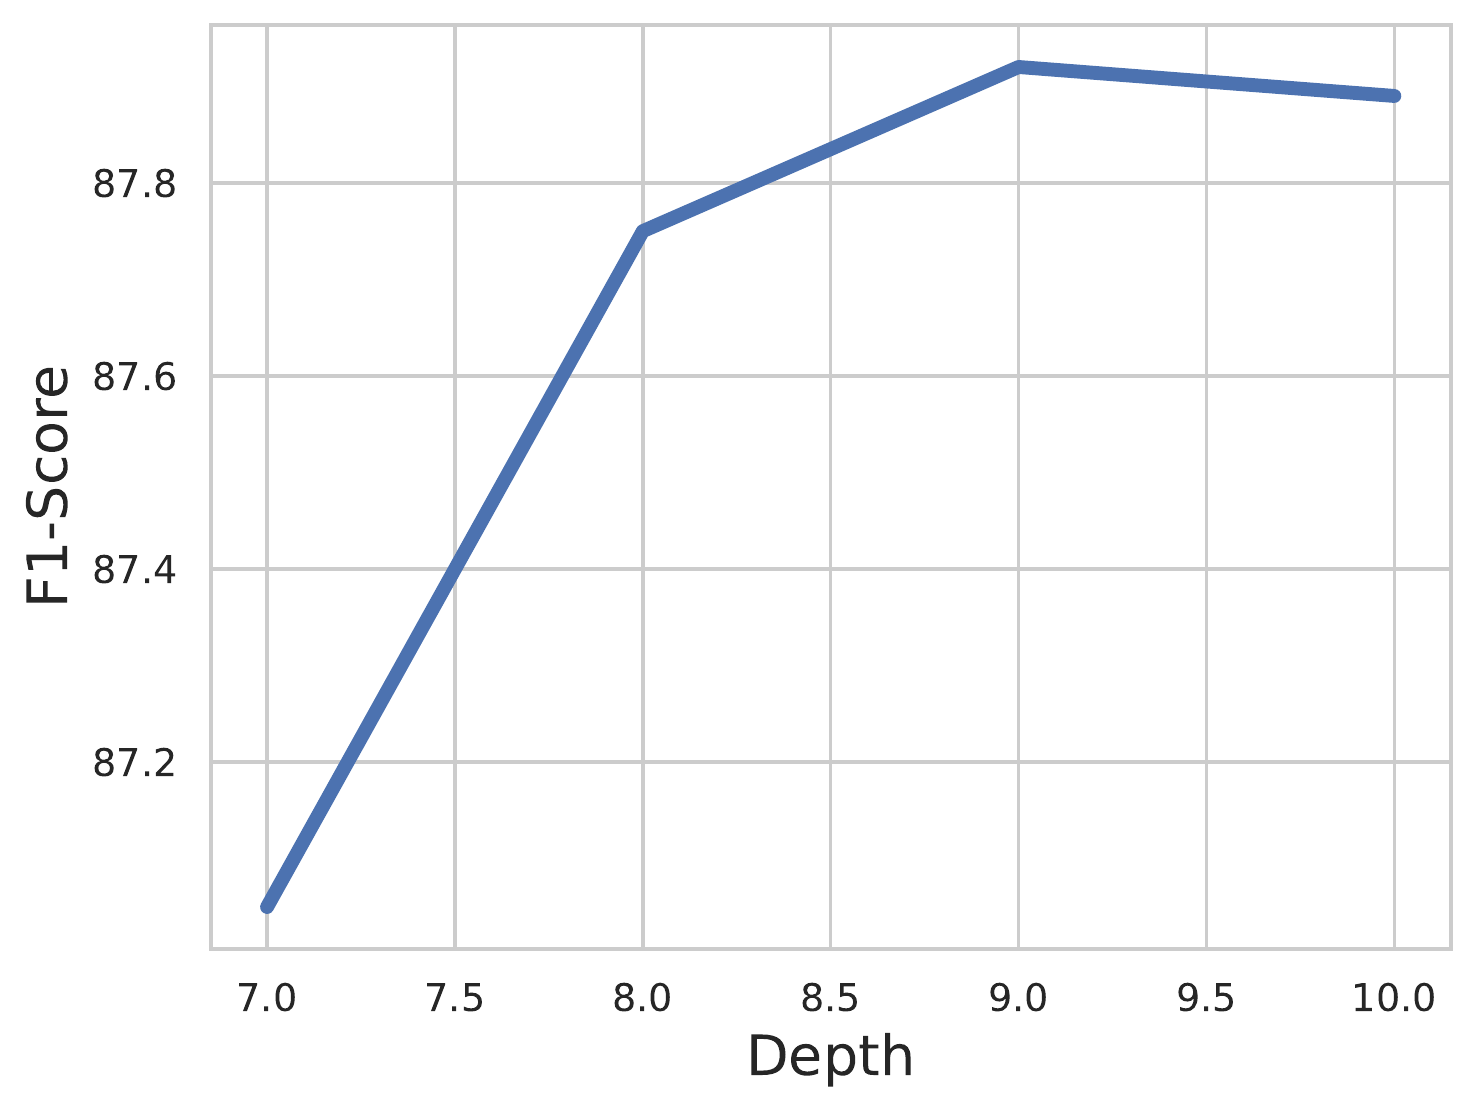}
  \caption{F1-Score depending on the depth used in Poisson surface reconstruction.}.
  \label{fig:f1_vs_dpoisson}
\end{subfigure}%
\\
\begin{subfigure}{.49\textwidth}
  \centering
  \includegraphics[width=1.0\linewidth]{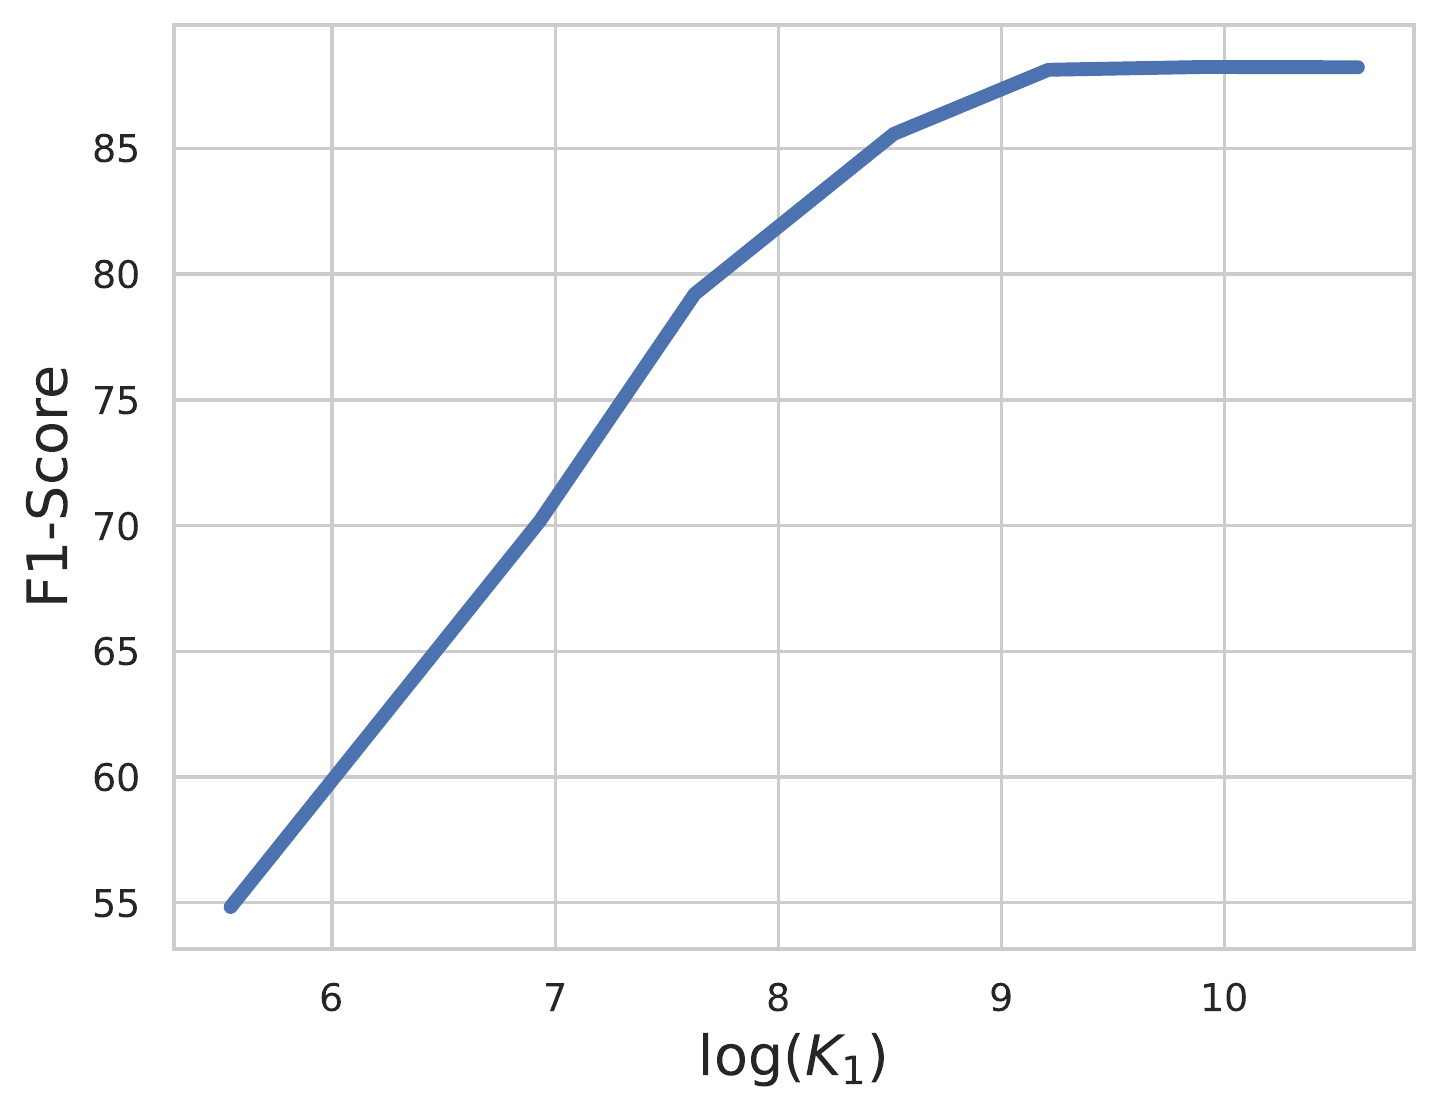}
  \caption{F1-Score depending on the on the logarithm of the number of points K\textsubscript{1}.}
  \label{fig:f1_vs_nr_points}
\end{subfigure}
\caption{Analysis of the sensitivity of ManiFlow-LL-Poisson to the depth used for Poisson surface reconstruction (a) and the number of points K\textsubscript{1} (b) on the airplane category.}
\label{fig:llpoisson_ablation}
\end{figure}

\subsection{Further Visualization of Point Clouds}\label{suppl_sec:vis_pcs}

\begin{figure*}[t]
\begin{center}

    \renewcommand{\figsize}{0.17}
    \newcommand{\planesize}{3.0}
    
    \begin{tabular}{ c c c c c }
    \setlength{\tabcolsep}{0pt} % Default value: 6pt
     % Default value: 1
    
        \centering 
    
      GT  & DPM~\cite{luo2021diffusion} & NF & NF\textsubscript{LLM} & NF\textsubscript{LL-Poisson} \\
      
      \includegraphics[width=\figsize\linewidth,trim={\planesize cm \planesize cm \planesize cm \planesize cm},clip]{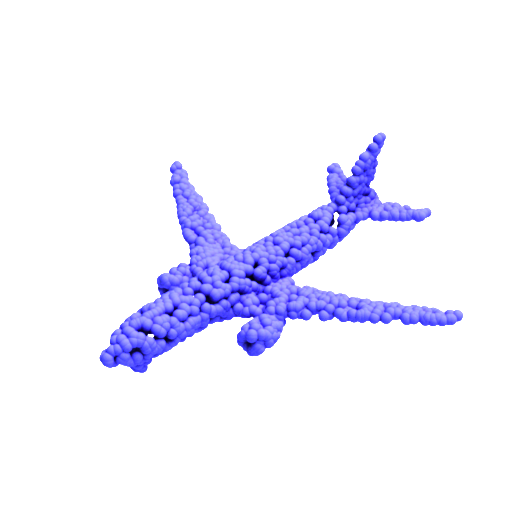} &
      \includegraphics[width=\figsize\linewidth,trim={\planesize cm \planesize cm \planesize cm \planesize cm},clip]{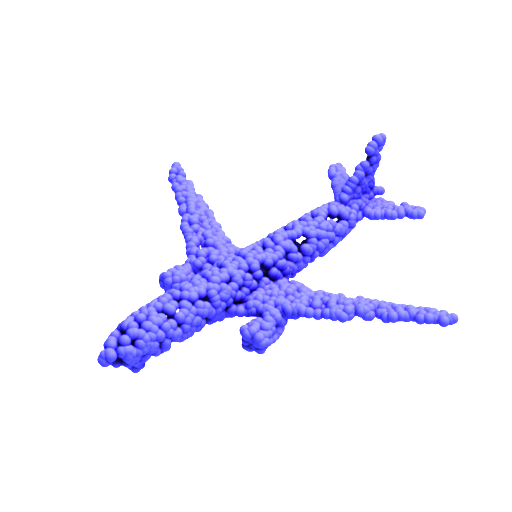} &
      \includegraphics[width=\figsize\linewidth,trim={\planesize cm \planesize cm \planesize cm \planesize cm},clip]{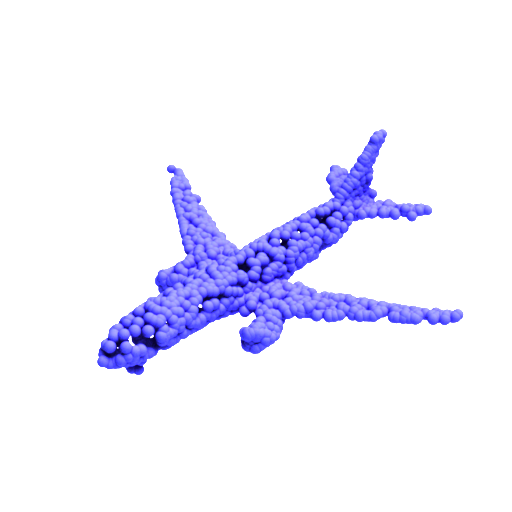} &
      \includegraphics[width=\figsize\linewidth,trim={\planesize cm \planesize cm \planesize cm \planesize cm},clip]{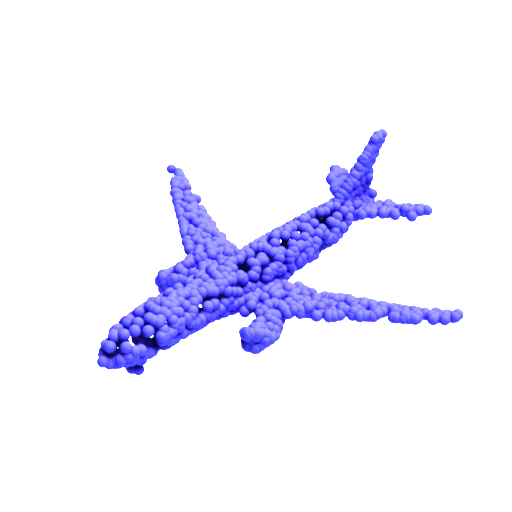} &
      \includegraphics[width=\figsize\linewidth,trim={\planesize cm \planesize cm \planesize cm \planesize cm},clip]{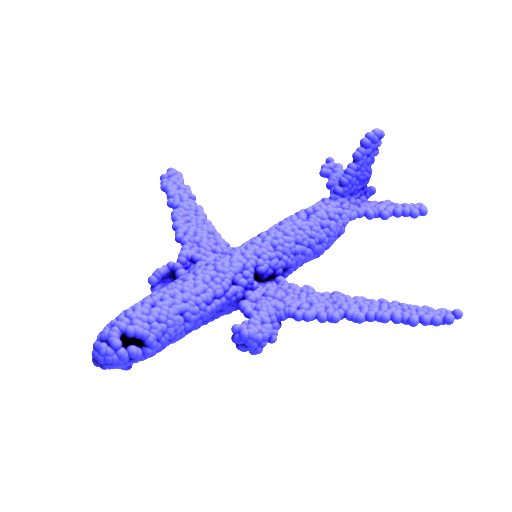} \\
      
      \includegraphics[width=\figsize\linewidth,trim={\planesize cm \planesize cm \planesize cm \planesize cm},clip]{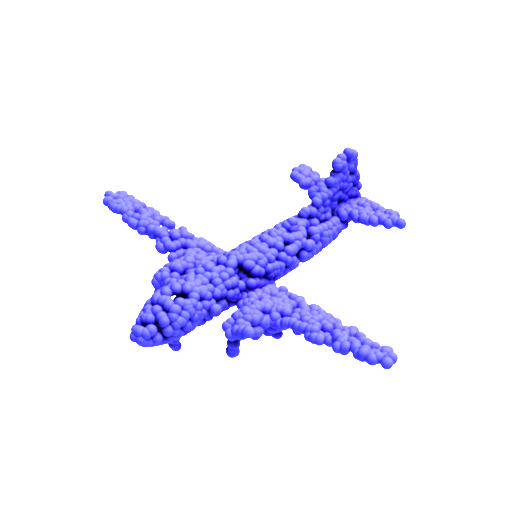} &
      \includegraphics[width=\figsize\linewidth,trim={\planesize cm \planesize cm \planesize cm \planesize cm},clip]{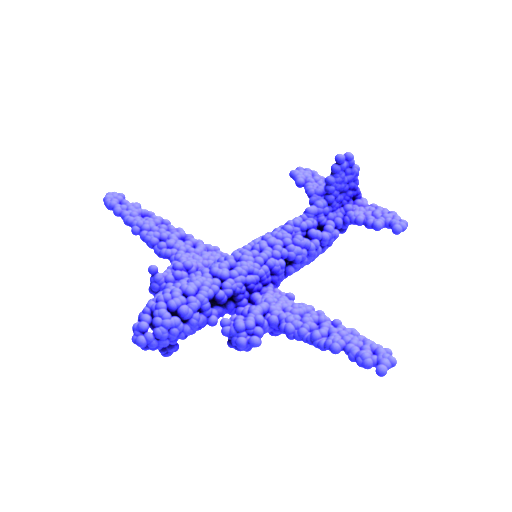} &
      \includegraphics[width=\figsize\linewidth,trim={\planesize cm \planesize cm \planesize cm \planesize cm},clip]{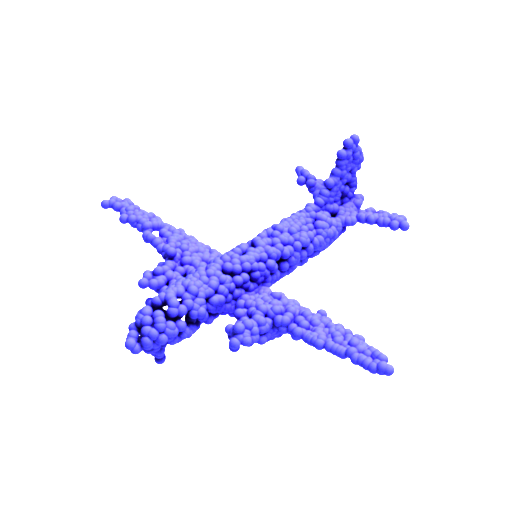} &
      \includegraphics[width=\figsize\linewidth,trim={\planesize cm \planesize cm \planesize cm \planesize cm},clip]{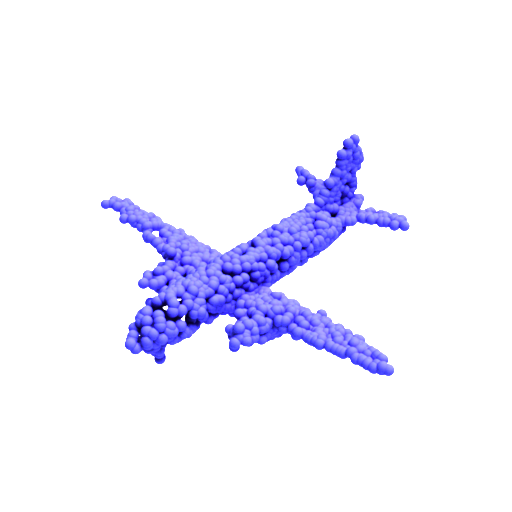} &
      \includegraphics[width=\figsize\linewidth,trim={\planesize cm \planesize cm \planesize cm \planesize cm},clip]{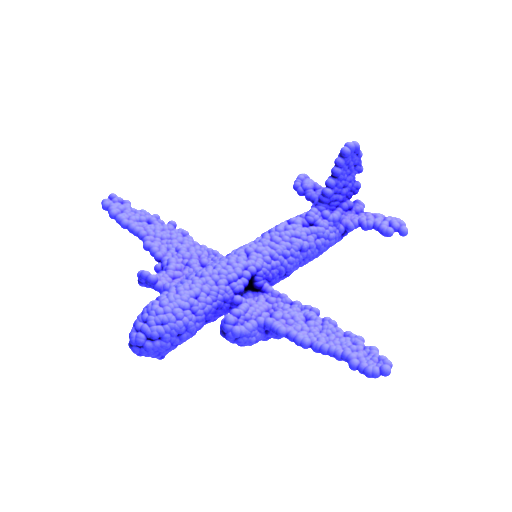} \\
      
      \includegraphics[width=\figsize\linewidth,trim={\planesize cm \planesize cm \planesize cm \planesize cm},clip]{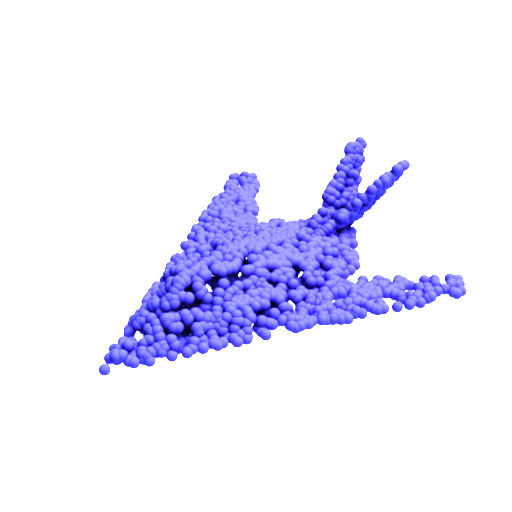} &
      \includegraphics[width=\figsize\linewidth,trim={\planesize cm \planesize cm \planesize cm \planesize cm},clip]{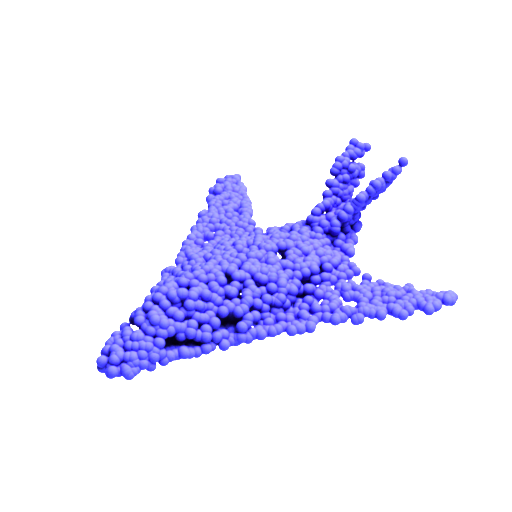} &
      \includegraphics[width=\figsize\linewidth,trim={\planesize cm \planesize cm \planesize cm \planesize cm},clip]{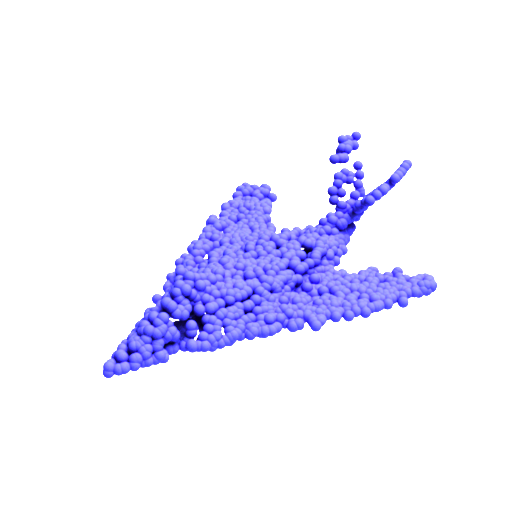} &
      \includegraphics[width=\figsize\linewidth,trim={\planesize cm \planesize cm \planesize cm \planesize cm},clip]{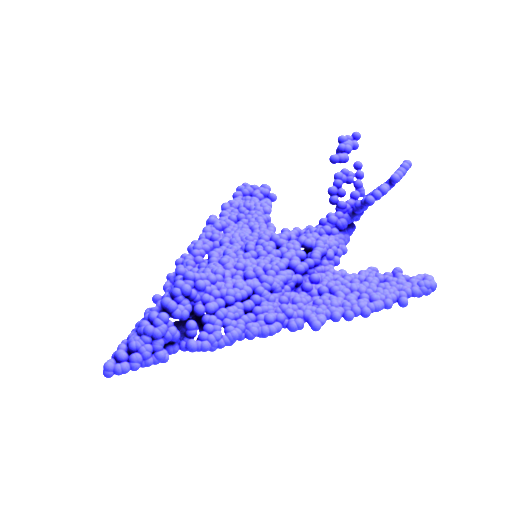} &
      \includegraphics[width=\figsize\linewidth,trim={\planesize cm \planesize cm \planesize cm \planesize cm},clip]{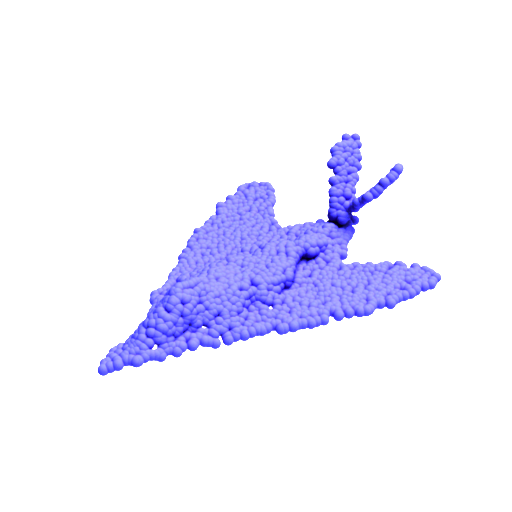} \\
      
    \end{tabular}
    
\end{center}
\caption{Further qualitative results on the airplane category of the ground truth (GT), DPM~\cite{luo2021diffusion}, a RealNVP (NF) and a RealNVP with LLM/LL-Poisson (NF\textsubscript{LLM}/NF\textsubscript{LL-Poisson}).}\label{fig:airplane_supplement}
\end{figure*}

\begin{figure*}[t]
\begin{center}

    \renewcommand{\figsize}{0.15}
    \newcommand{\carsize}{3.5}
    
    \begin{tabular}{ c c c c c }
    \setlength{\tabcolsep}{0pt} % Default value: 6pt
     % Default value: 1
    
        \centering 
    
      GT  & DPM~\cite{luo2021diffusion} & NF & NF\textsubscript{LLM} & NF\textsubscript{LL-Poisson} \\
      
      \includegraphics[width=\figsize\linewidth,trim={\carsize cm \carsize cm \carsize cm \carsize cm},clip]{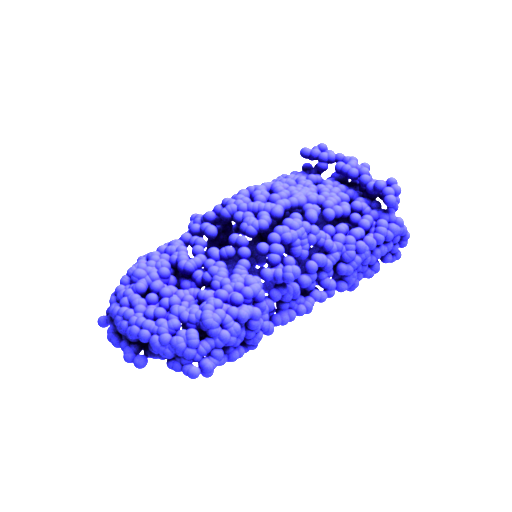} &
      \includegraphics[width=\figsize\linewidth,trim={\carsize cm \carsize cm \carsize cm \carsize cm},clip]{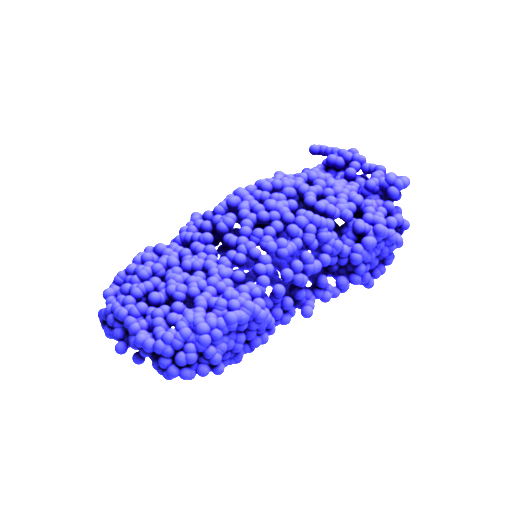} &
      \includegraphics[width=\figsize\linewidth,trim={\carsize cm \carsize cm \carsize cm \carsize cm},clip]{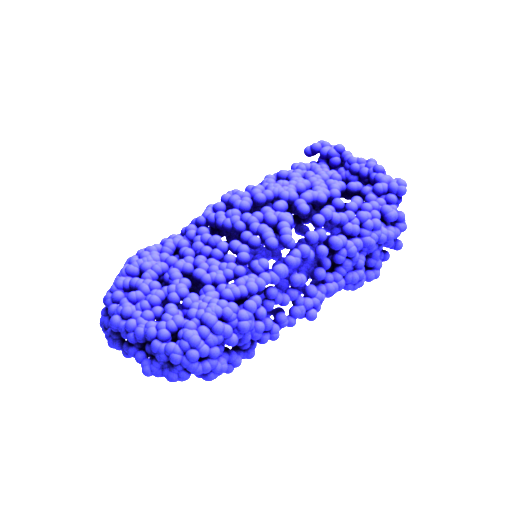} &
      \includegraphics[width=\figsize\linewidth,trim={\carsize cm \carsize cm \carsize cm \carsize cm},clip]{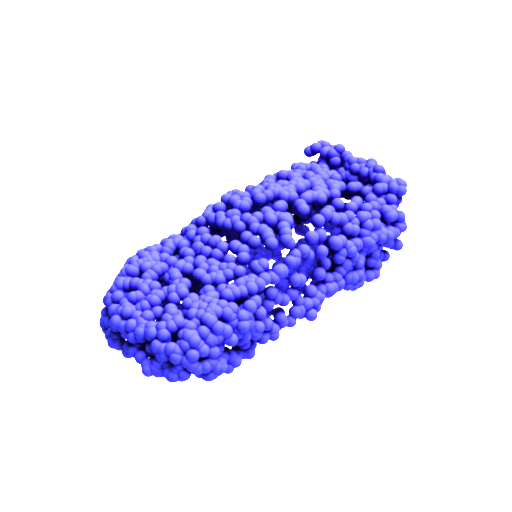} &
      \includegraphics[width=\figsize\linewidth,trim={\carsize cm \carsize cm \carsize cm \carsize cm},clip]{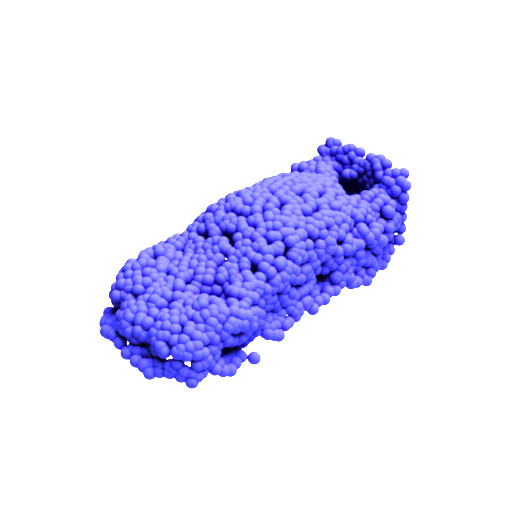} \\
      
      \includegraphics[width=\figsize\linewidth,trim={\carsize cm \carsize cm \carsize cm \carsize cm},clip]{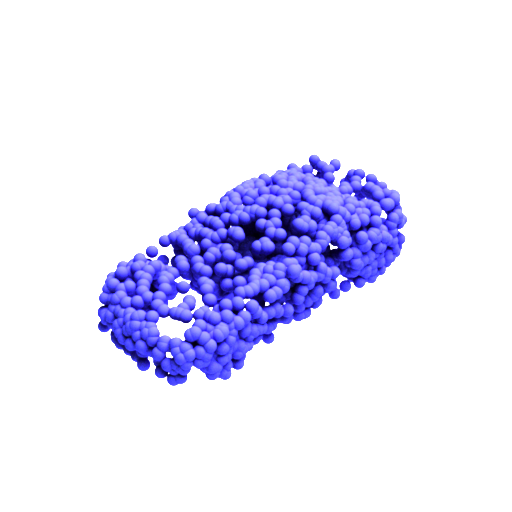} &
      \includegraphics[width=\figsize\linewidth,trim={\carsize cm \carsize cm \carsize cm \carsize cm},clip]{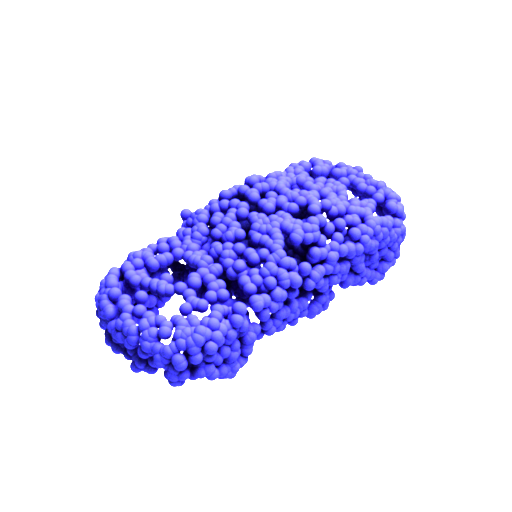} &
      \includegraphics[width=\figsize\linewidth,trim={\carsize cm \carsize cm \carsize cm \carsize cm},clip]{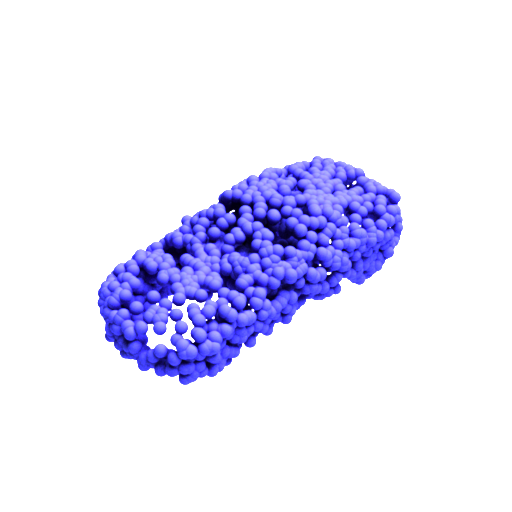} &
      \includegraphics[width=\figsize\linewidth,trim={\carsize cm \carsize cm \carsize cm \carsize cm},clip]{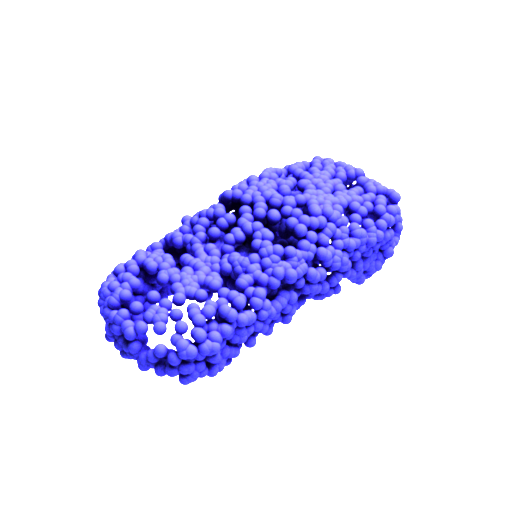} &
      \includegraphics[width=\figsize\linewidth,trim={\carsize cm \carsize cm \carsize cm \carsize cm},clip]{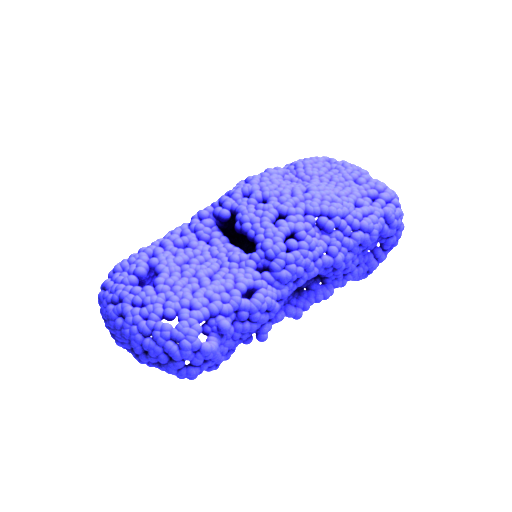} \\
      
      \includegraphics[width=\figsize\linewidth,trim={\carsize cm \carsize cm \carsize cm \carsize cm},clip]{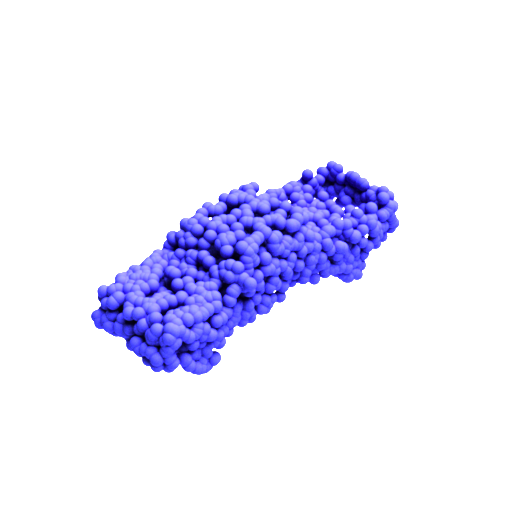} &
      \includegraphics[width=\figsize\linewidth,trim={\carsize cm \carsize cm \carsize cm \carsize cm},clip]{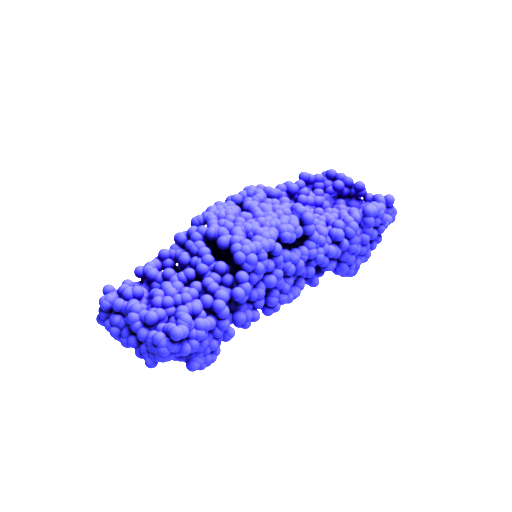} &
      \includegraphics[width=\figsize\linewidth,trim={\carsize cm \carsize cm \carsize cm \carsize cm},clip]{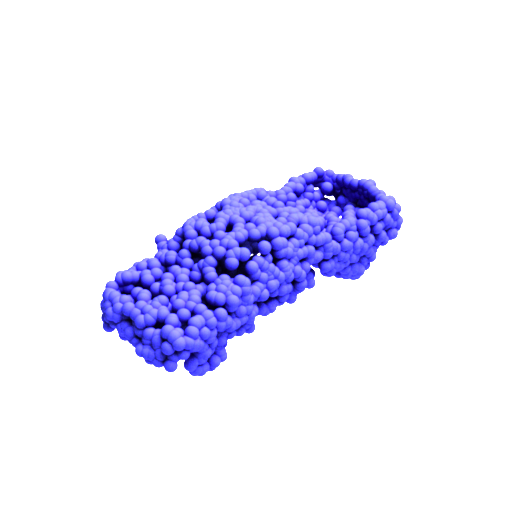} &
      \includegraphics[width=\figsize\linewidth,trim={\carsize cm \carsize cm \carsize cm \carsize cm},clip]{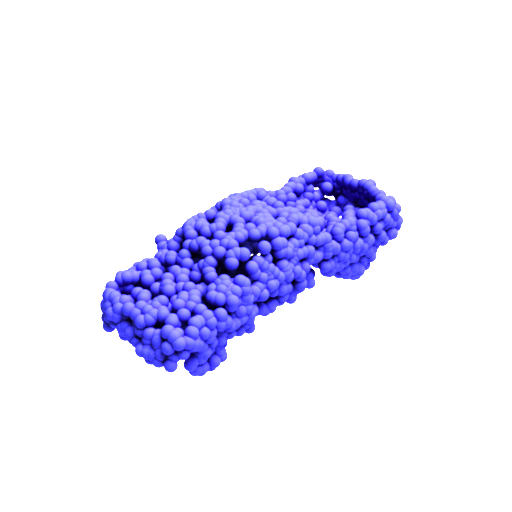} &
      \includegraphics[width=\figsize\linewidth,trim={\carsize cm \carsize cm \carsize cm \carsize cm},clip]{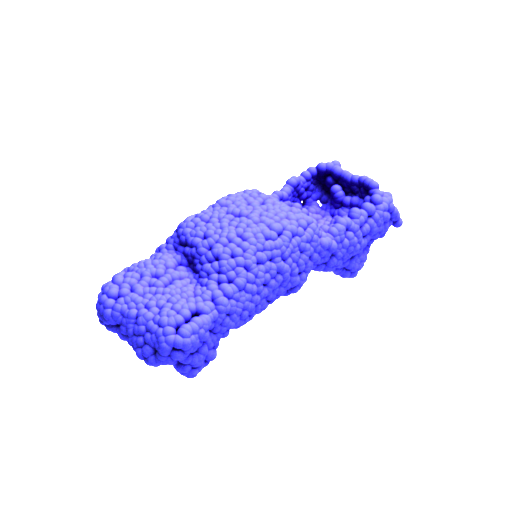} \\
      
    \end{tabular}
    
\end{center}
\caption{Further qualitative results on the car category of the ground truth (GT), DPM~\cite{luo2021diffusion}, a RealNVP (NF) and a RealNVP with LLM/LL-Poisson (NF\textsubscript{LLM}/NF\textsubscript{LL-Poisson}).}\label{fig:car_supplement}
\end{figure*}

\begin{figure*}[t]
\begin{center}

    \renewcommand{\figsize}{0.15}
    \newcommand{\chairsize}{1.0}
    
    \begin{tabular}{ c c c c c }
    \setlength{\tabcolsep}{0pt} % Default value: 6pt
     % Default value: 1
    
        \centering 
    
      GT  & DPM~\cite{luo2021diffusion} & NF & NF\textsubscript{LLM} & NF\textsubscript{LL-Poisson} \\
      
      \includegraphics[width=\figsize\linewidth,trim={\chairsize cm \chairsize cm \chairsize cm \chairsize cm},clip]{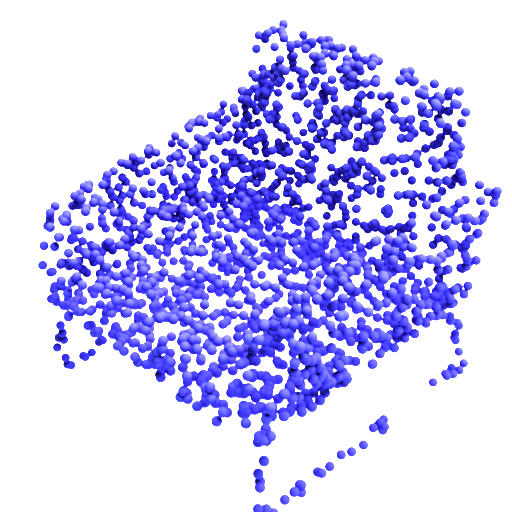}&
      \includegraphics[width=\figsize\linewidth,trim={\chairsize cm \chairsize cm \chairsize cm \chairsize cm},clip]{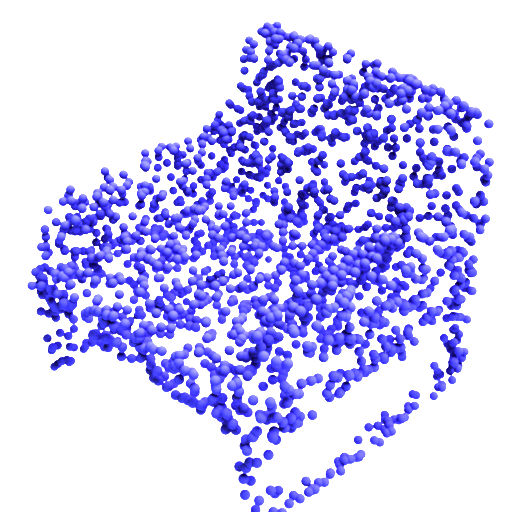} &
      \includegraphics[width=\figsize\linewidth,trim={\chairsize cm \chairsize cm \chairsize cm \chairsize cm},clip]{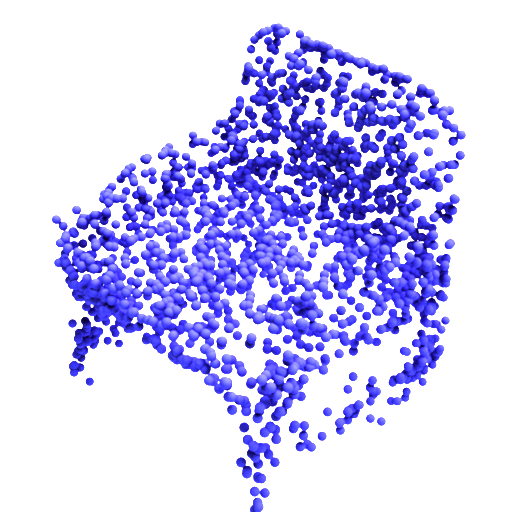} &
      \includegraphics[width=\figsize\linewidth,trim={\chairsize cm \chairsize cm \chairsize cm \chairsize cm},clip]{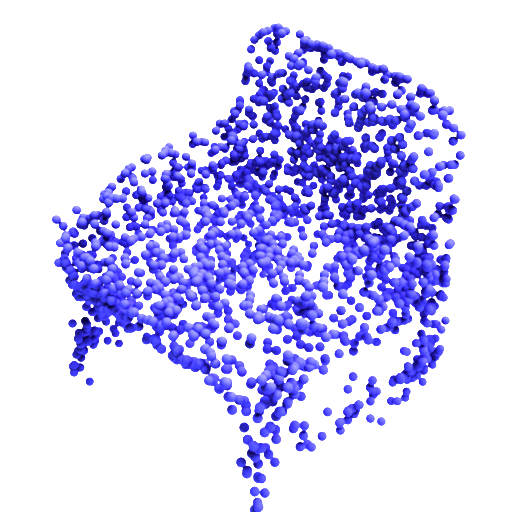} &
      \includegraphics[width=\figsize\linewidth,trim={\chairsize cm \chairsize cm \chairsize cm \chairsize cm},clip]{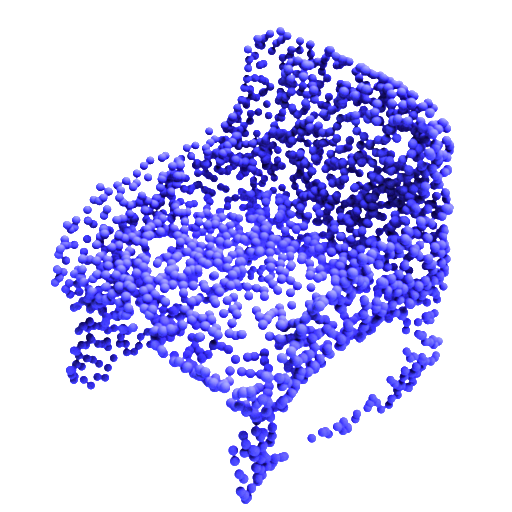} \\
      
      \includegraphics[width=\figsize\linewidth,trim={\chairsize cm \chairsize cm \chairsize cm \chairsize cm},clip]{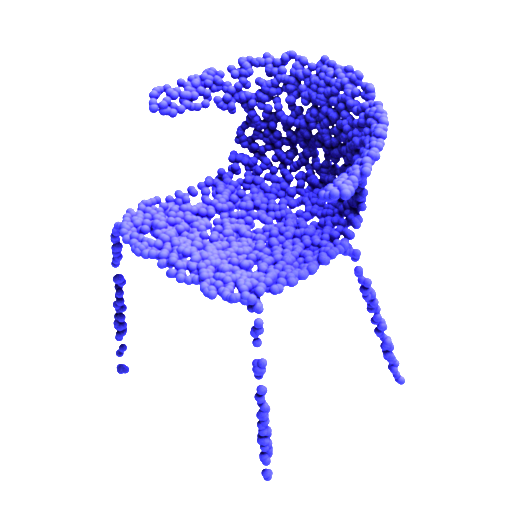}&
      \includegraphics[width=\figsize\linewidth,trim={\chairsize cm \chairsize cm \chairsize cm \chairsize cm},clip]{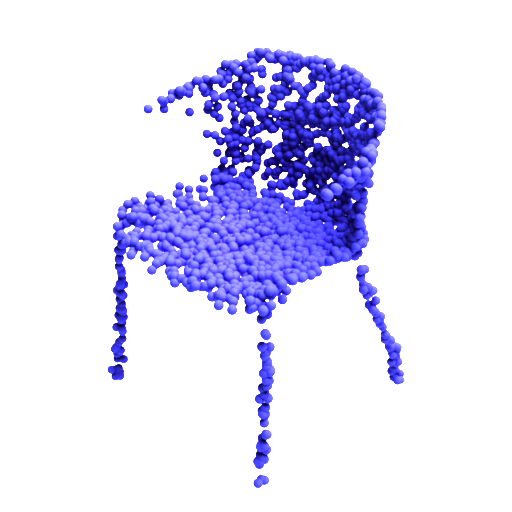} &
      \includegraphics[width=\figsize\linewidth,trim={\chairsize cm \chairsize cm \chairsize cm \chairsize cm},clip]{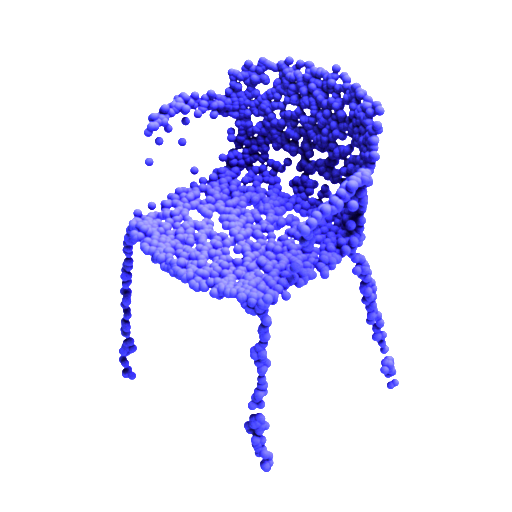} &
      \includegraphics[width=\figsize\linewidth,trim={\chairsize cm \chairsize cm \chairsize cm \chairsize cm},clip]{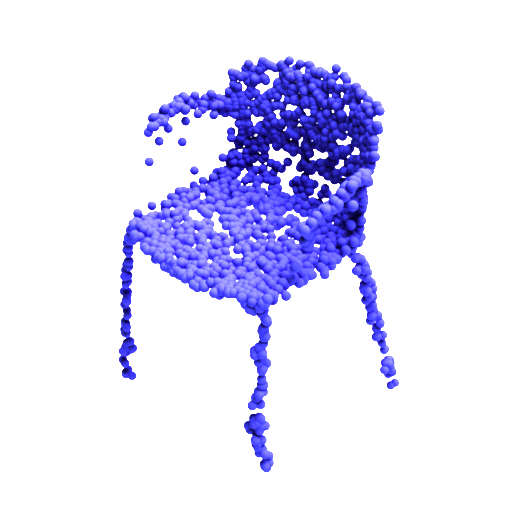} &
      \includegraphics[width=\figsize\linewidth,trim={\chairsize cm \chairsize cm \chairsize cm \chairsize cm},clip]{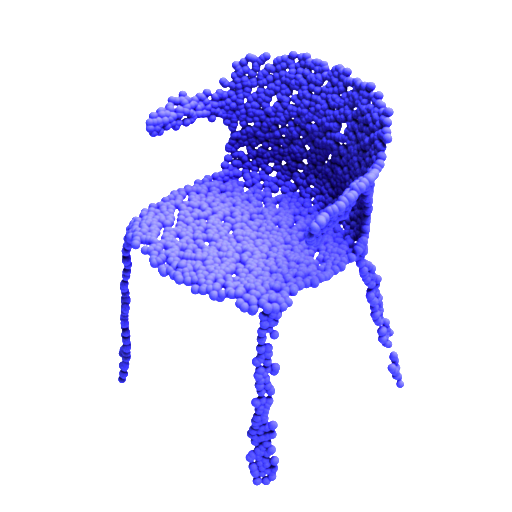} \\
      
      \includegraphics[width=\figsize\linewidth,trim={\chairsize cm \chairsize cm \chairsize cm \chairsize cm},clip]{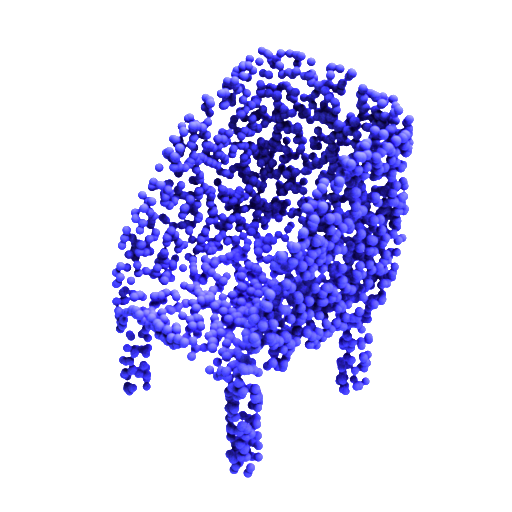}&
      \includegraphics[width=\figsize\linewidth,trim={\chairsize cm \chairsize cm \chairsize cm \chairsize cm},clip]{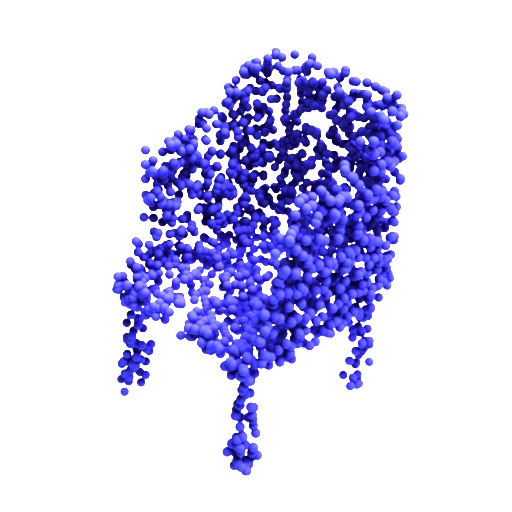} &
      \includegraphics[width=\figsize\linewidth,trim={\chairsize cm \chairsize cm \chairsize cm \chairsize cm},clip]{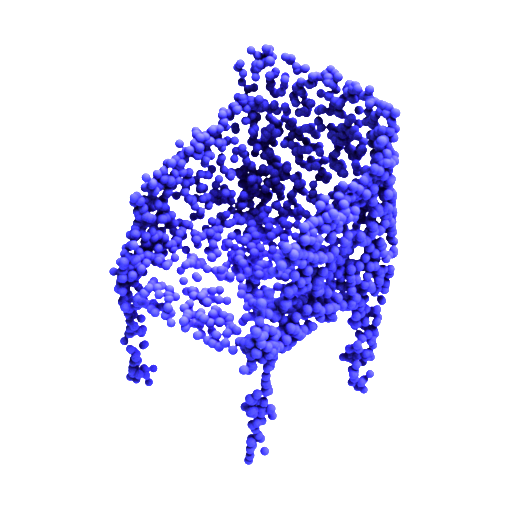} &
      \includegraphics[width=\figsize\linewidth,trim={\chairsize cm \chairsize cm \chairsize cm \chairsize cm},clip]{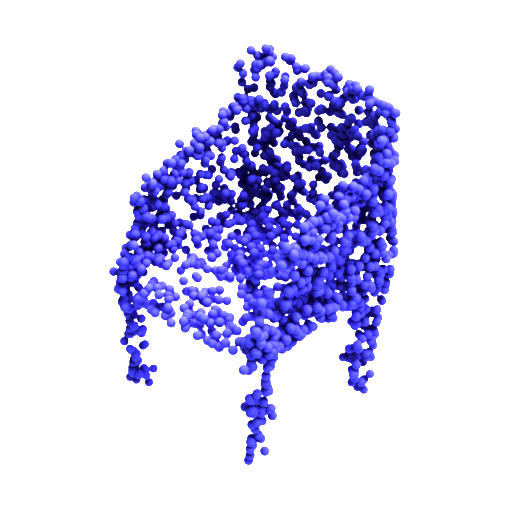} &
      \includegraphics[width=\figsize\linewidth,trim={\chairsize cm \chairsize cm \chairsize cm \chairsize cm},clip]{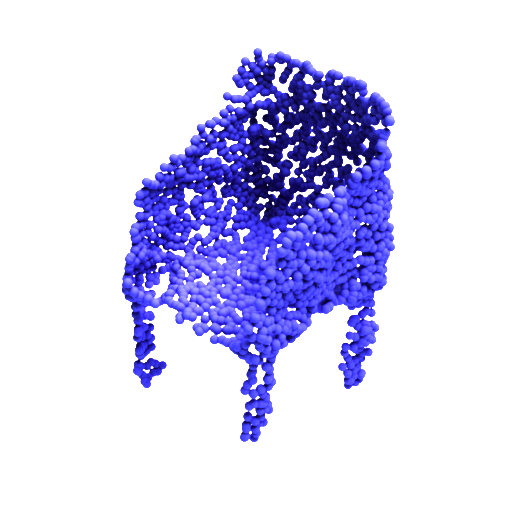} \\
      
    \end{tabular}
    
\end{center}
\caption{Further qualitative results on the chair category of the ground truth (GT), DPM~\cite{luo2021diffusion}, a RealNVP (NF) and a RealNVP with LLM/LL-Poisson (NF\textsubscript{LLM}/NF\textsubscript{LL-Poisson}).}\label{fig:chair_supplement}
\end{figure*}

We provide additional qualitative examples of generated point clouds in \figref{fig:airplane_supplement}, \figref{fig:car_supplement} and \figref{fig:chair_supplement}.

\subsection{Visualization of Meshes}\label{suppl_sec:vis_meshes}

Poisson surface reconstruction in LL-Poisson extracts a mesh of the 3D shape from the \ac{nf}'s log-likelihood. We provide qualitative examples of these meshes in \figref{fig:ll_poisson_meshes}. Note that these meshes correspond to the point clouds visualized in \figref{fig:airplane_supplement}, \figref{fig:car_supplement} and \figref{fig:chair_supplement}.

\begin{figure*}[b]
\begin{center}

    \renewcommand{\figsize}{0.15}
    
    \begin{tabular}{ c c c }
    \setlength{\tabcolsep}{0pt} % Default value: 6pt
     % Default value: 1
    
        \centering 
      
      \includegraphics[width=\figsize\linewidth]{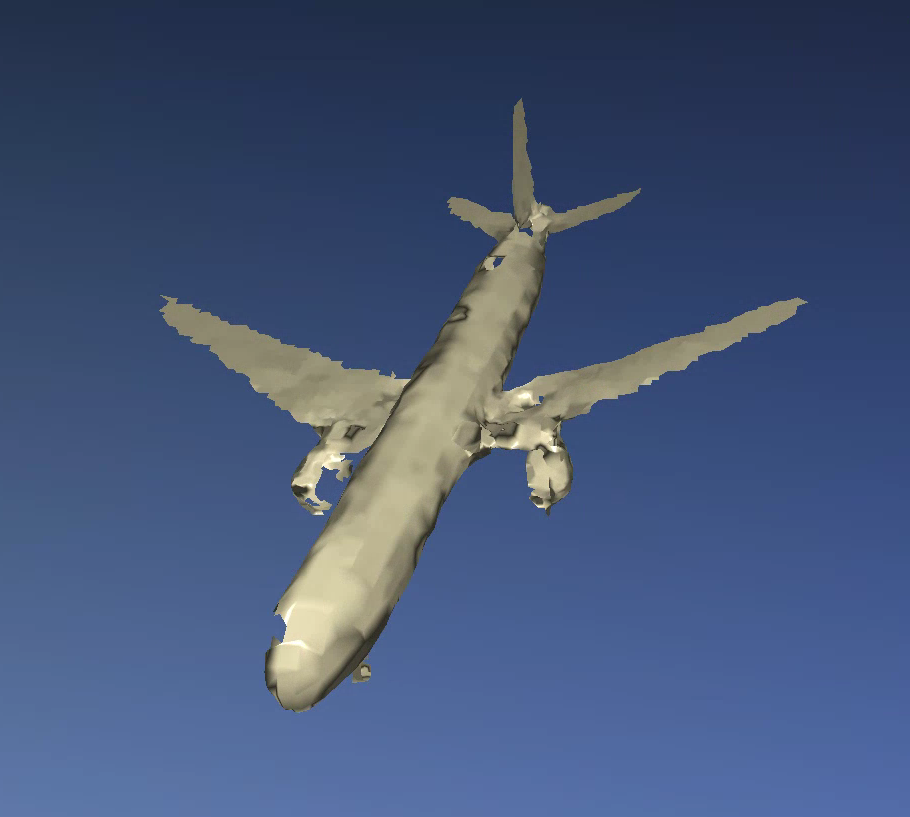} &
      \includegraphics[width=\figsize\linewidth]{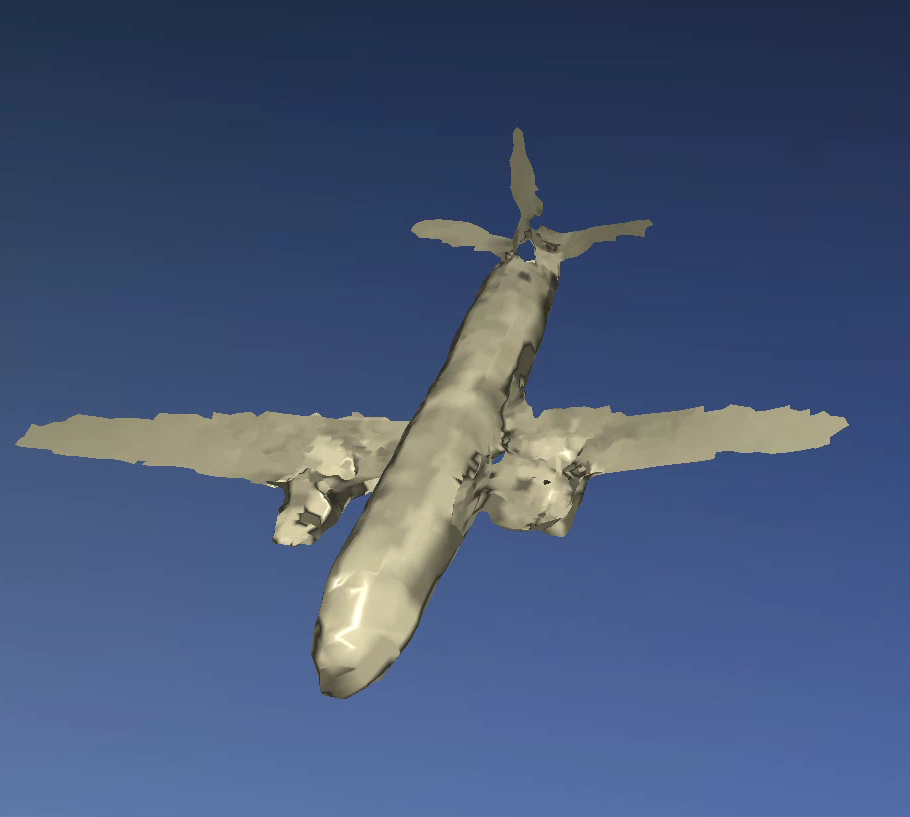} &
      \includegraphics[width=\figsize\linewidth]{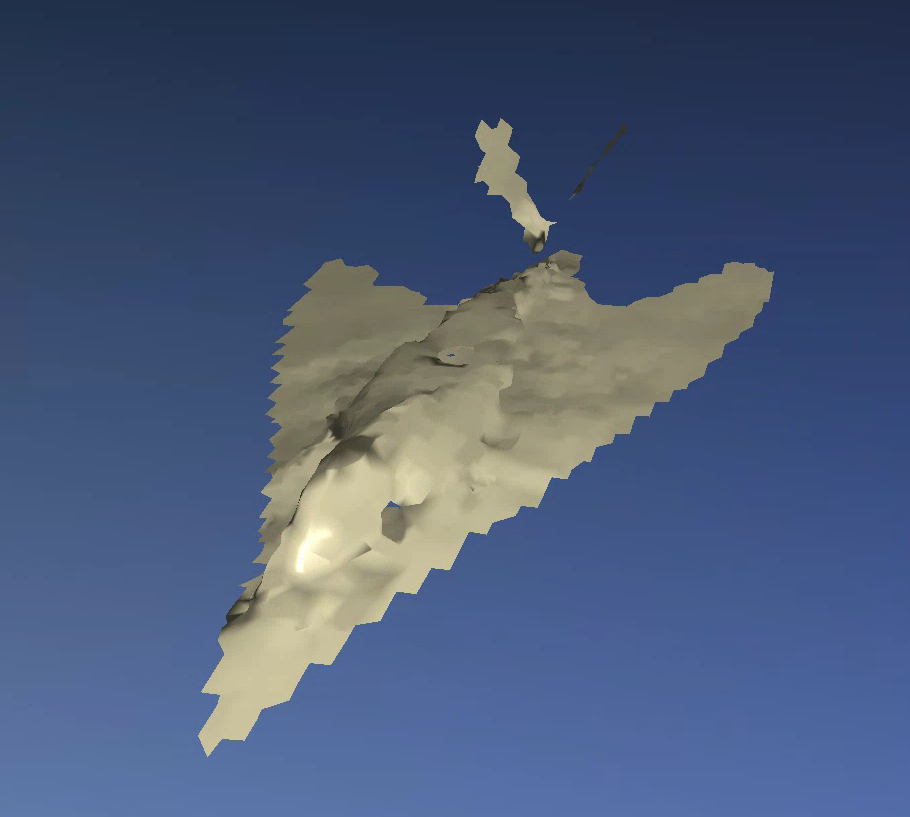} \\
      
      \includegraphics[width=\figsize\linewidth]{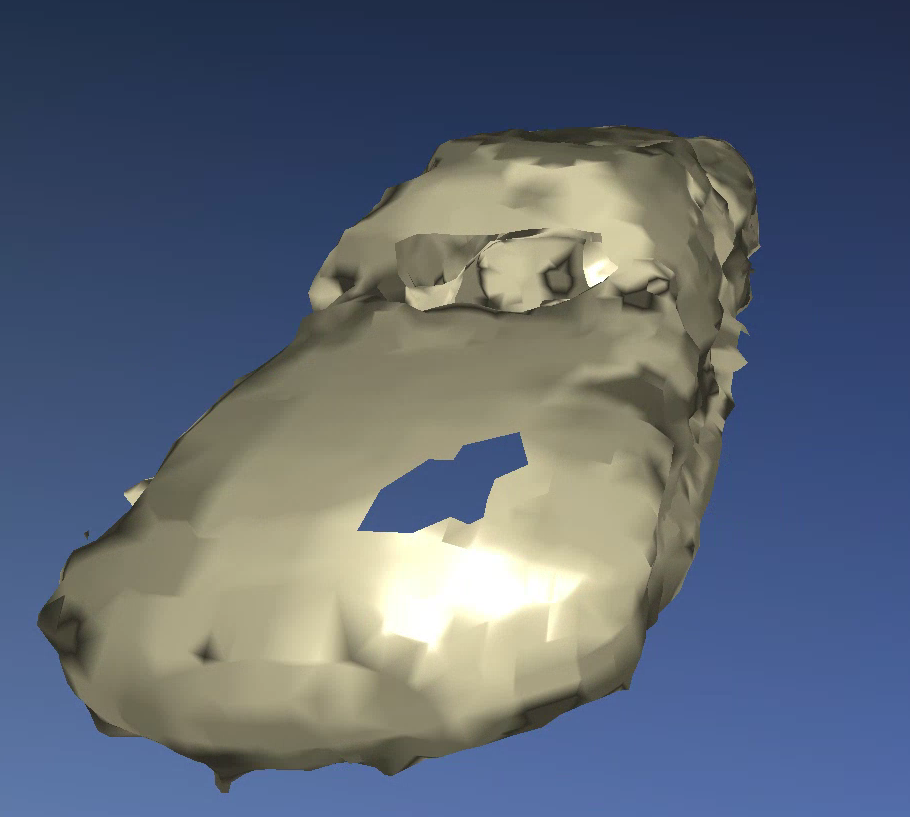} &
      \includegraphics[width=\figsize\linewidth]{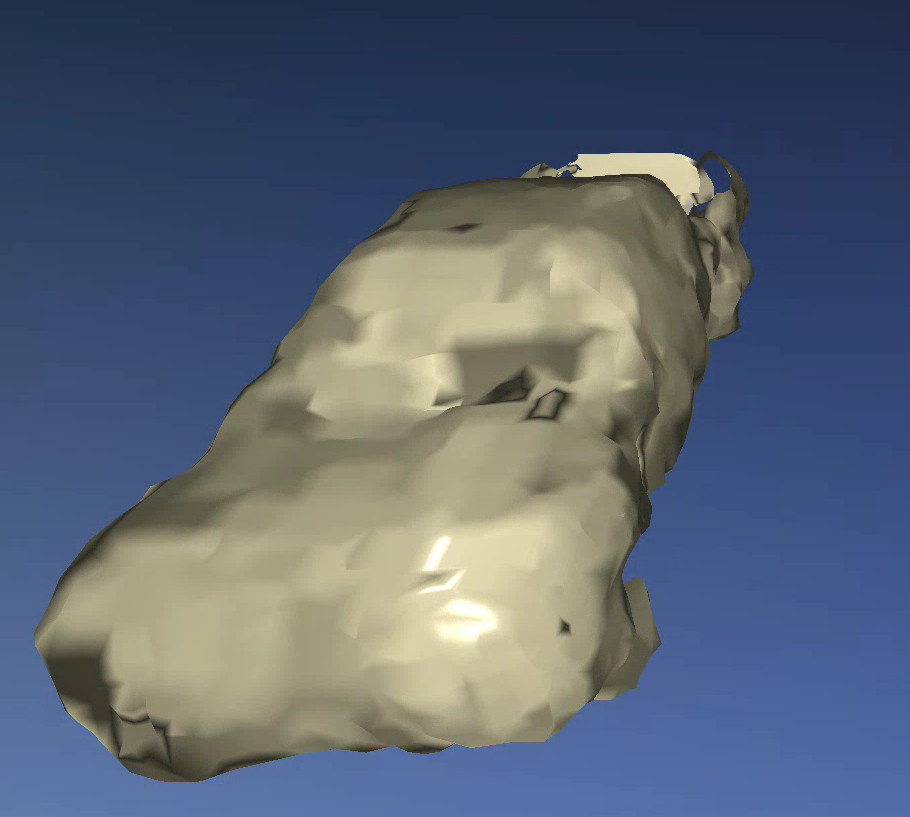} &
      \includegraphics[width=\figsize\linewidth]{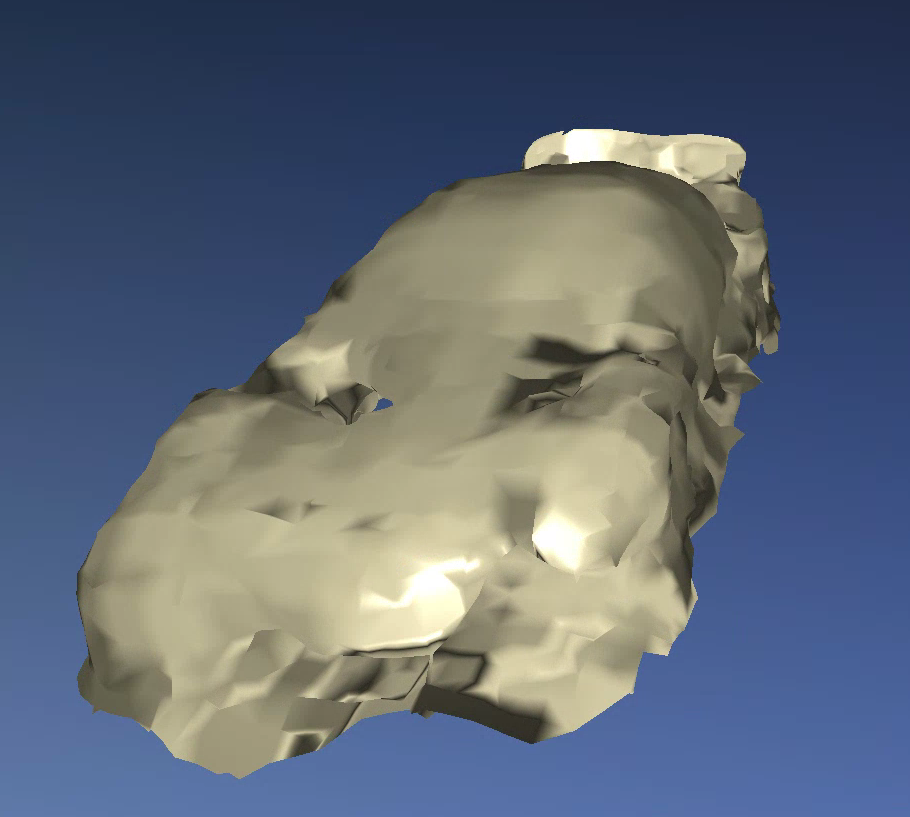} \\
      
      \includegraphics[width=\figsize\linewidth]{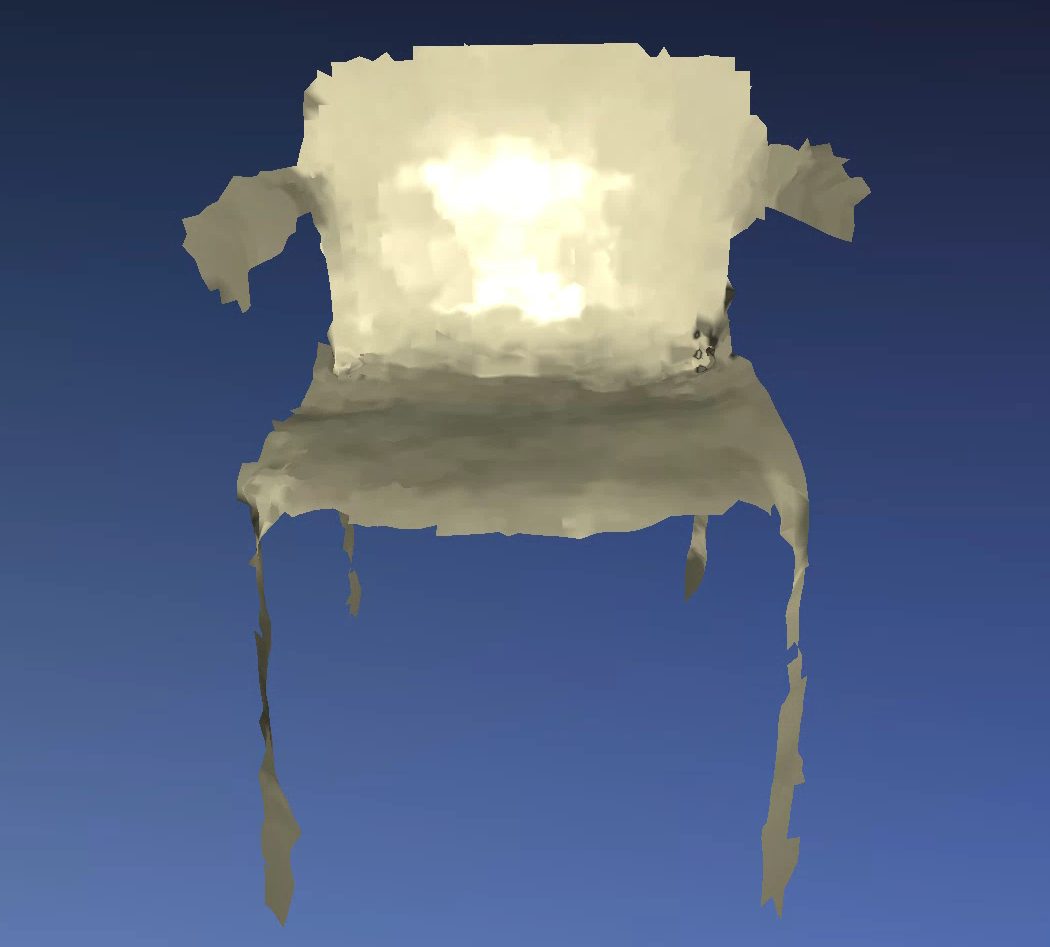} &
      \includegraphics[width=\figsize\linewidth]{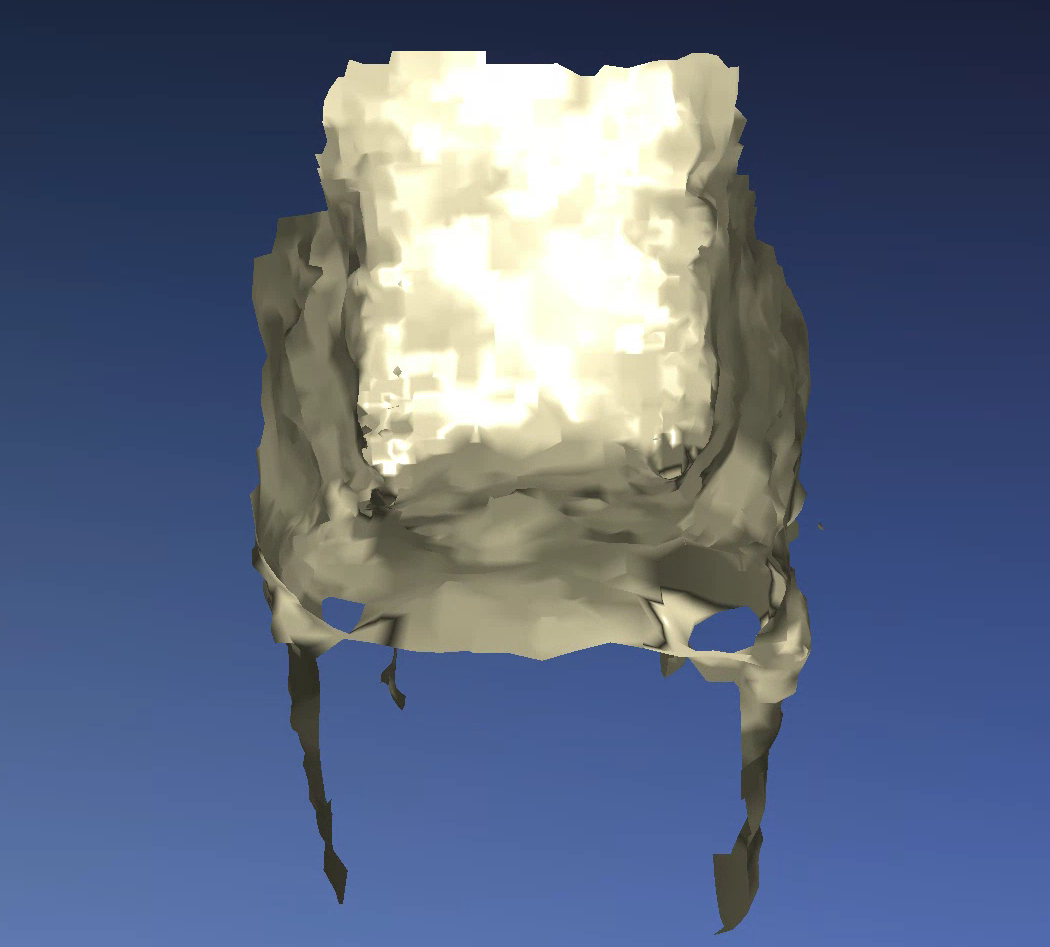} &
      \includegraphics[width=\figsize\linewidth]{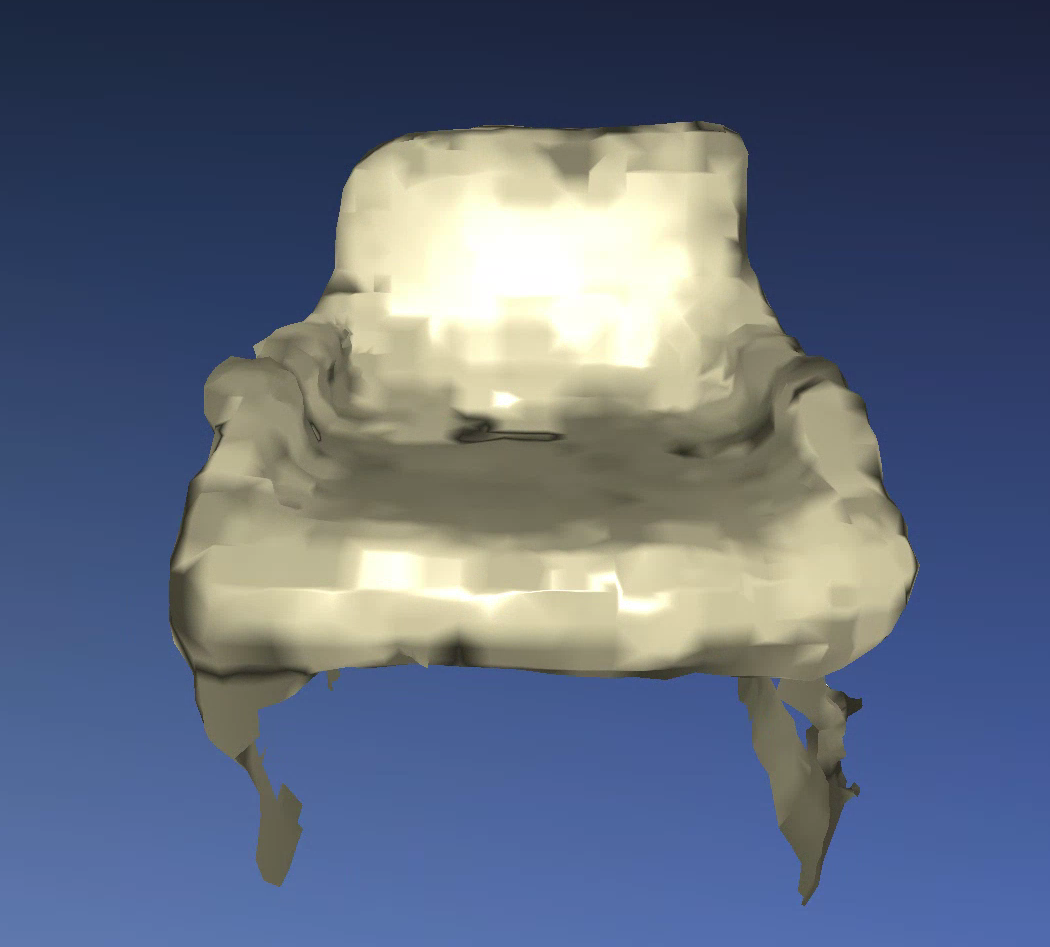} \\
      
    \end{tabular}
    
\end{center}
\caption{Qualitative examples of meshes created with LL-Poisson on the categories airplane, car and chair.}\label{fig:ll_poisson_meshes}
\end{figure*}

\subsection{Visualization of Generated Images}\label{suppl_sec:gen_imgs}

\subsection{Proof of Properties of the Log-Likelihood of Normalizing Flows}\label{suppl_sec:proof}

We now prove assumptions about the log-likelihood of \acp{nf} made in \secref{subsection:sampling_manifold}. 
Let $\Omega$ denote a m-dimensional compact manifold embedded in n-dimensional Euclidean space, $\Omega \in \mathbb{R}^n$ where $m<n$. Let further $X$/$S$ refer to a random variables with their corresponding probability density $P_X$/$P_S$ and $x\sim P_X(x)$, resp. $s\sim P_S(s)$, realizations of these random variables. Moreover, let $S$ exist on the m-dimensional manifold $\Omega$ such that $P_S(x) = 0$ $\forall x \notin \Omega$.
Assuming that $S$ is locally well approximated by a m-dimensional hypersphere with radius $r\gg \sigma$ and that $P_S$ is approximately uniform on this hypersphere, we show that i) the gradient of the log-likelihood $\log(P_X)$ is perpendicular to $S$ and ii) that $P_X$ has a maximum on $S$.  

To this end, we will consider one sample $x\sim P_X$ and approximate $P_S$ in its neighborhood using the aforementioned hypersphere L and multivariate Gaussian noise with a covariance matrix $\Sigma = \sigma^2 I$.
\begin{align}
    P_X(x) &= \int_{\mathbb{R}^n} P_N(x-s)P_S(s) ds \nonumber\\
    &= \int_{\mathbb{R}^n} P_N(x-s)p_0\delta(f_{imp}(s)) ds \\
    &\approx \frac{p_0}{(2\pi \sigma^2)^{\frac{n}{2}}}\int_{L} \exp\left(  \frac{\sum_{i+1}^{n} (x - l)^2}{\sigma^{2n}}\right) dl \nonumber
\end{align}
where we have used $P_S(s) = p_0\delta(f_{imp}(s))$. $p_0$ is the local probability density, $\delta(x)$ the delta function and $f_{imp}(s)$ an implicit representation of $\Omega$ that is zero on $\Omega$. Thus, we are integrating the noise distribution over the hypersphere. Without loss of generality let us assume that L is zero-centered and axis aligned - i.e. n-m basis vectors of the n-dimensional space are perpendicular to L. Now let $M = \{ i_1, \dots, i_k \}$ denote the set of basis vectors that are parallel to L, then we have 
\begin{align}
\begin{split}
    P_X(x) \approx & \frac{p_0}{(2\pi \sigma^2)^{\frac{n}{2}}} \exp\left(  \frac{\sum_{i\not\in M} x_i^2}{\sigma^{2n}}\right) \\ &\int_{L} \exp\left(  \frac{\sum_{i\in M} (x_i - l_i)^2}{\sigma^{2n}}\right) dx_{i_1}\dots dx_{i_k}
\end{split}
\end{align}
Thus, we only integrate over the axis that are aligned with the hypersphere. Given that $r\gg \sigma$ and knowledge about the solution of the Gaussian integral, the integral approximately evaluates to $\int_{L} \exp\left(  \frac{\sum_{i\in M} (x_i - l_i)^2}{\sigma^{2n}}\right) dx_{i_1}\dots dx_{i_k} \approx (2\pi \sigma^2)^{\frac{m}{2}}$ for x close to the origin. Consequently, we can locally approximate $P_X$ with (d-m)-dimensional Gaussian distribution that is invariant to changes along basis vectors in $M$:
\begin{equation}
    P_X(x) \approx \frac{p_0}{(2\pi \sigma^2)^{\frac{n-m}{2}}} \exp\left(  \frac{\sum_{i\not\in M} x_i^2}{\sigma^{2n}}\right)
\end{equation}
From this we can see that $P_X$ approximately fulfills i) and ii).

\subsection{Experimental Details}\label{suppl_sec:exp_details}

\subsubsection{Architecture of Normalizing Flows}

\paragraph{Experiments on Artificial Data.} We train a RealNVP~\cite{dinh2016density} comprised of 5 coupling layers. Each coupling layer is comprised of two linear layers with a relu activation function and 128 hidden dimensions between them. We mask dimensions of the 2D data alternatingly.

\paragraph{Comparison with SoftFlow}~\cite{kim2020softflow} in \secref{subsection:pc_autoencoding}. We apply the architecture proposed in the original work~\cite{kim2020softflow}. The decoder \ac{nf} is comprised of a sequence of 8 identical modules. This module is depicted in \figref{fig:softflow_architecture}. Here, activation normalization (ActNorm) and invertible 1x1 convolutions are implemented according to GLOW~\cite{kingma2018glow}. 1x1 convolutions are enforced to be invertible by parameterizing the kernel using the LU-decomposition~\cite{kingma2018glow}. The invertible autoregressive layer is implemented according to~\cite{kingma2016improved}. In invertible autoregressive layers scaling and translation of each dimension are calculated autoregressively. Each autoregressive step is parameterized by a separate \ac{nn} consisting of of 4 linear layers with tanh activation functions and 256 hidden dimensions. 

\paragraph{General experiments on autoencoding} in \secref{subsection:pc_autoencoding}. Here the decoder model is implemented as a ReaLNVP~\cite{dinh2016density} consisting of 63 coupling layers. Such coupling layers are schematically depicted in \figref{fig:dpf_architecture}. A coupling layer splits the dimensions into two sets and applies the identity mapping to one set of dimensions. Further, the set of dimensions, which is mapped by the identity, is used to compute scaling and translation factors for the other set of dimensions. The computation of scaling and translation is parameterized by a \ac{nn} which consists of 2 linear layers with an intermediate Swish activation function and 64 hidden dimensions. The conditioning on the latent shape representation z is implemented by FiLM conditioning~\cite{perez2018film}.

\begin{figure*}
\centering
\begin{subfigure}{.9\textwidth}
  \centering
  \includegraphics[width=1.0\linewidth]{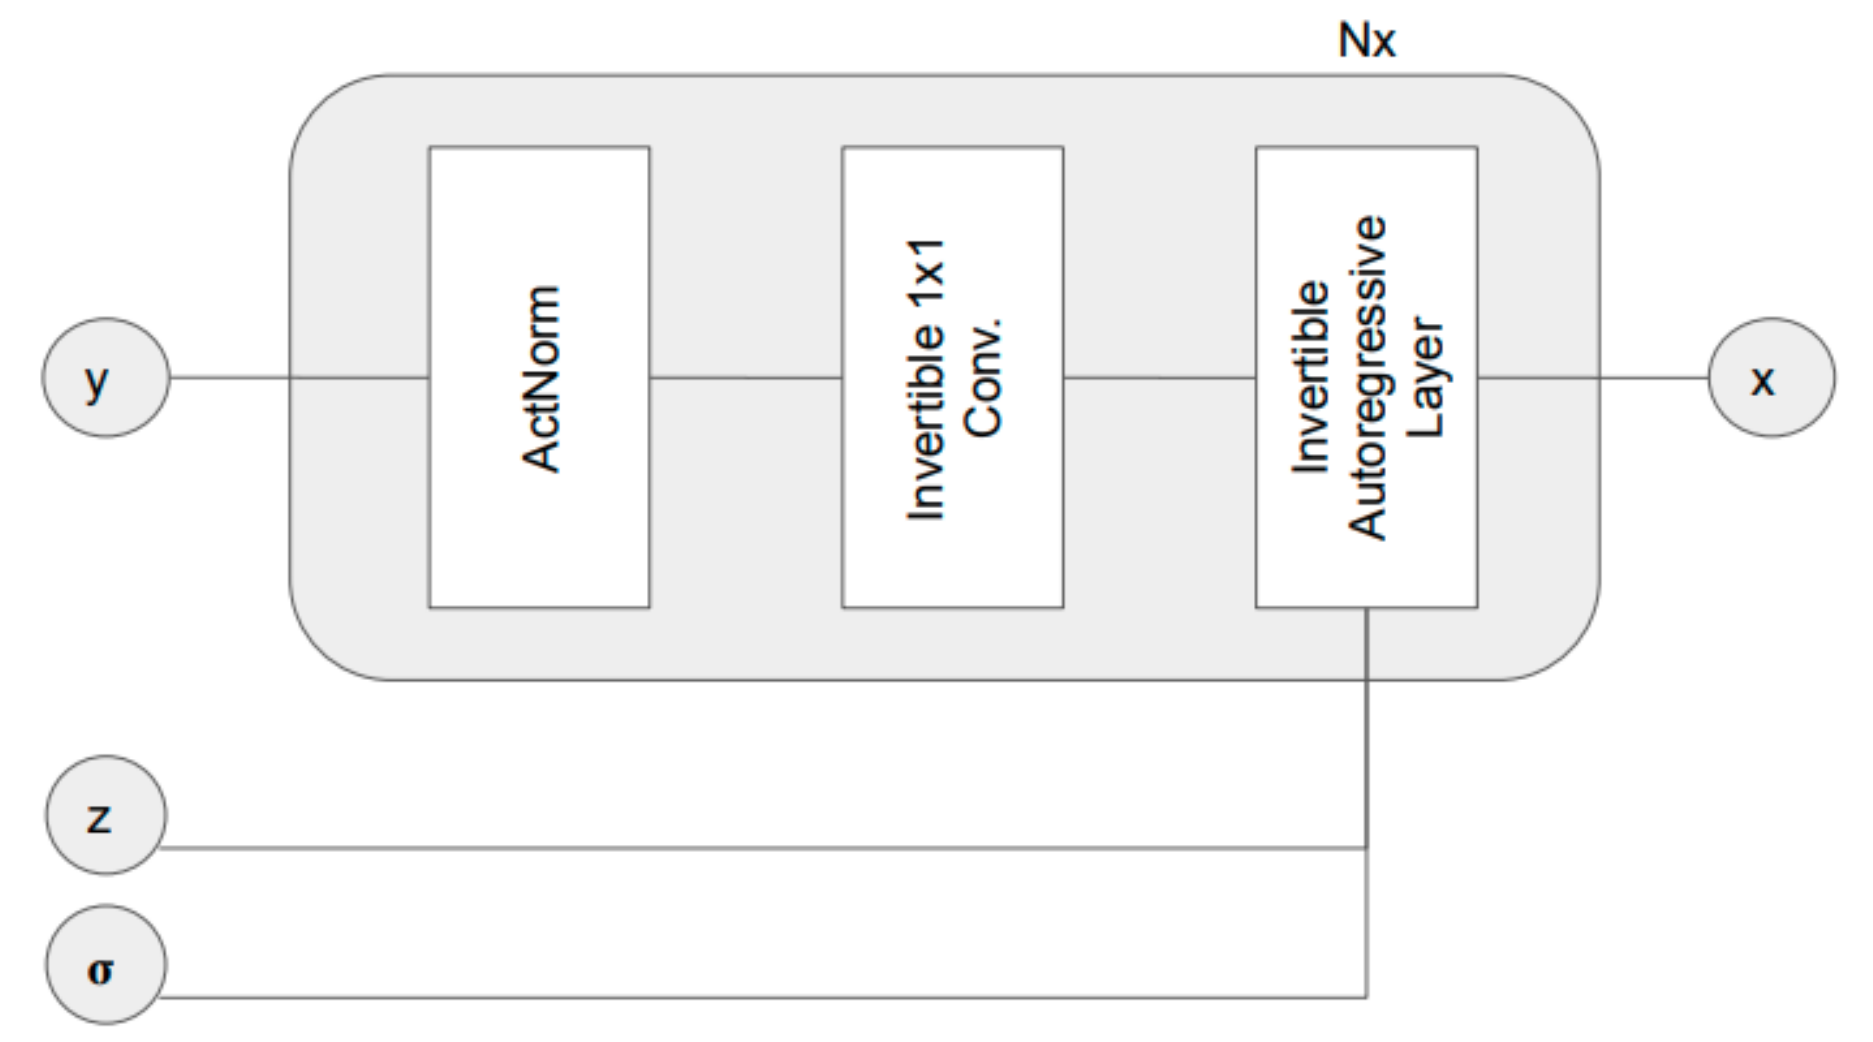}
  \caption{Basic module of architecture used in comparison with SoftFlow~\cite{kim2020softflow}.}.
  \label{fig:softflow_architecture}
\end{subfigure}%
\\
\begin{subfigure}{.9\textwidth}
  \centering
  \includegraphics[width=.9\linewidth]{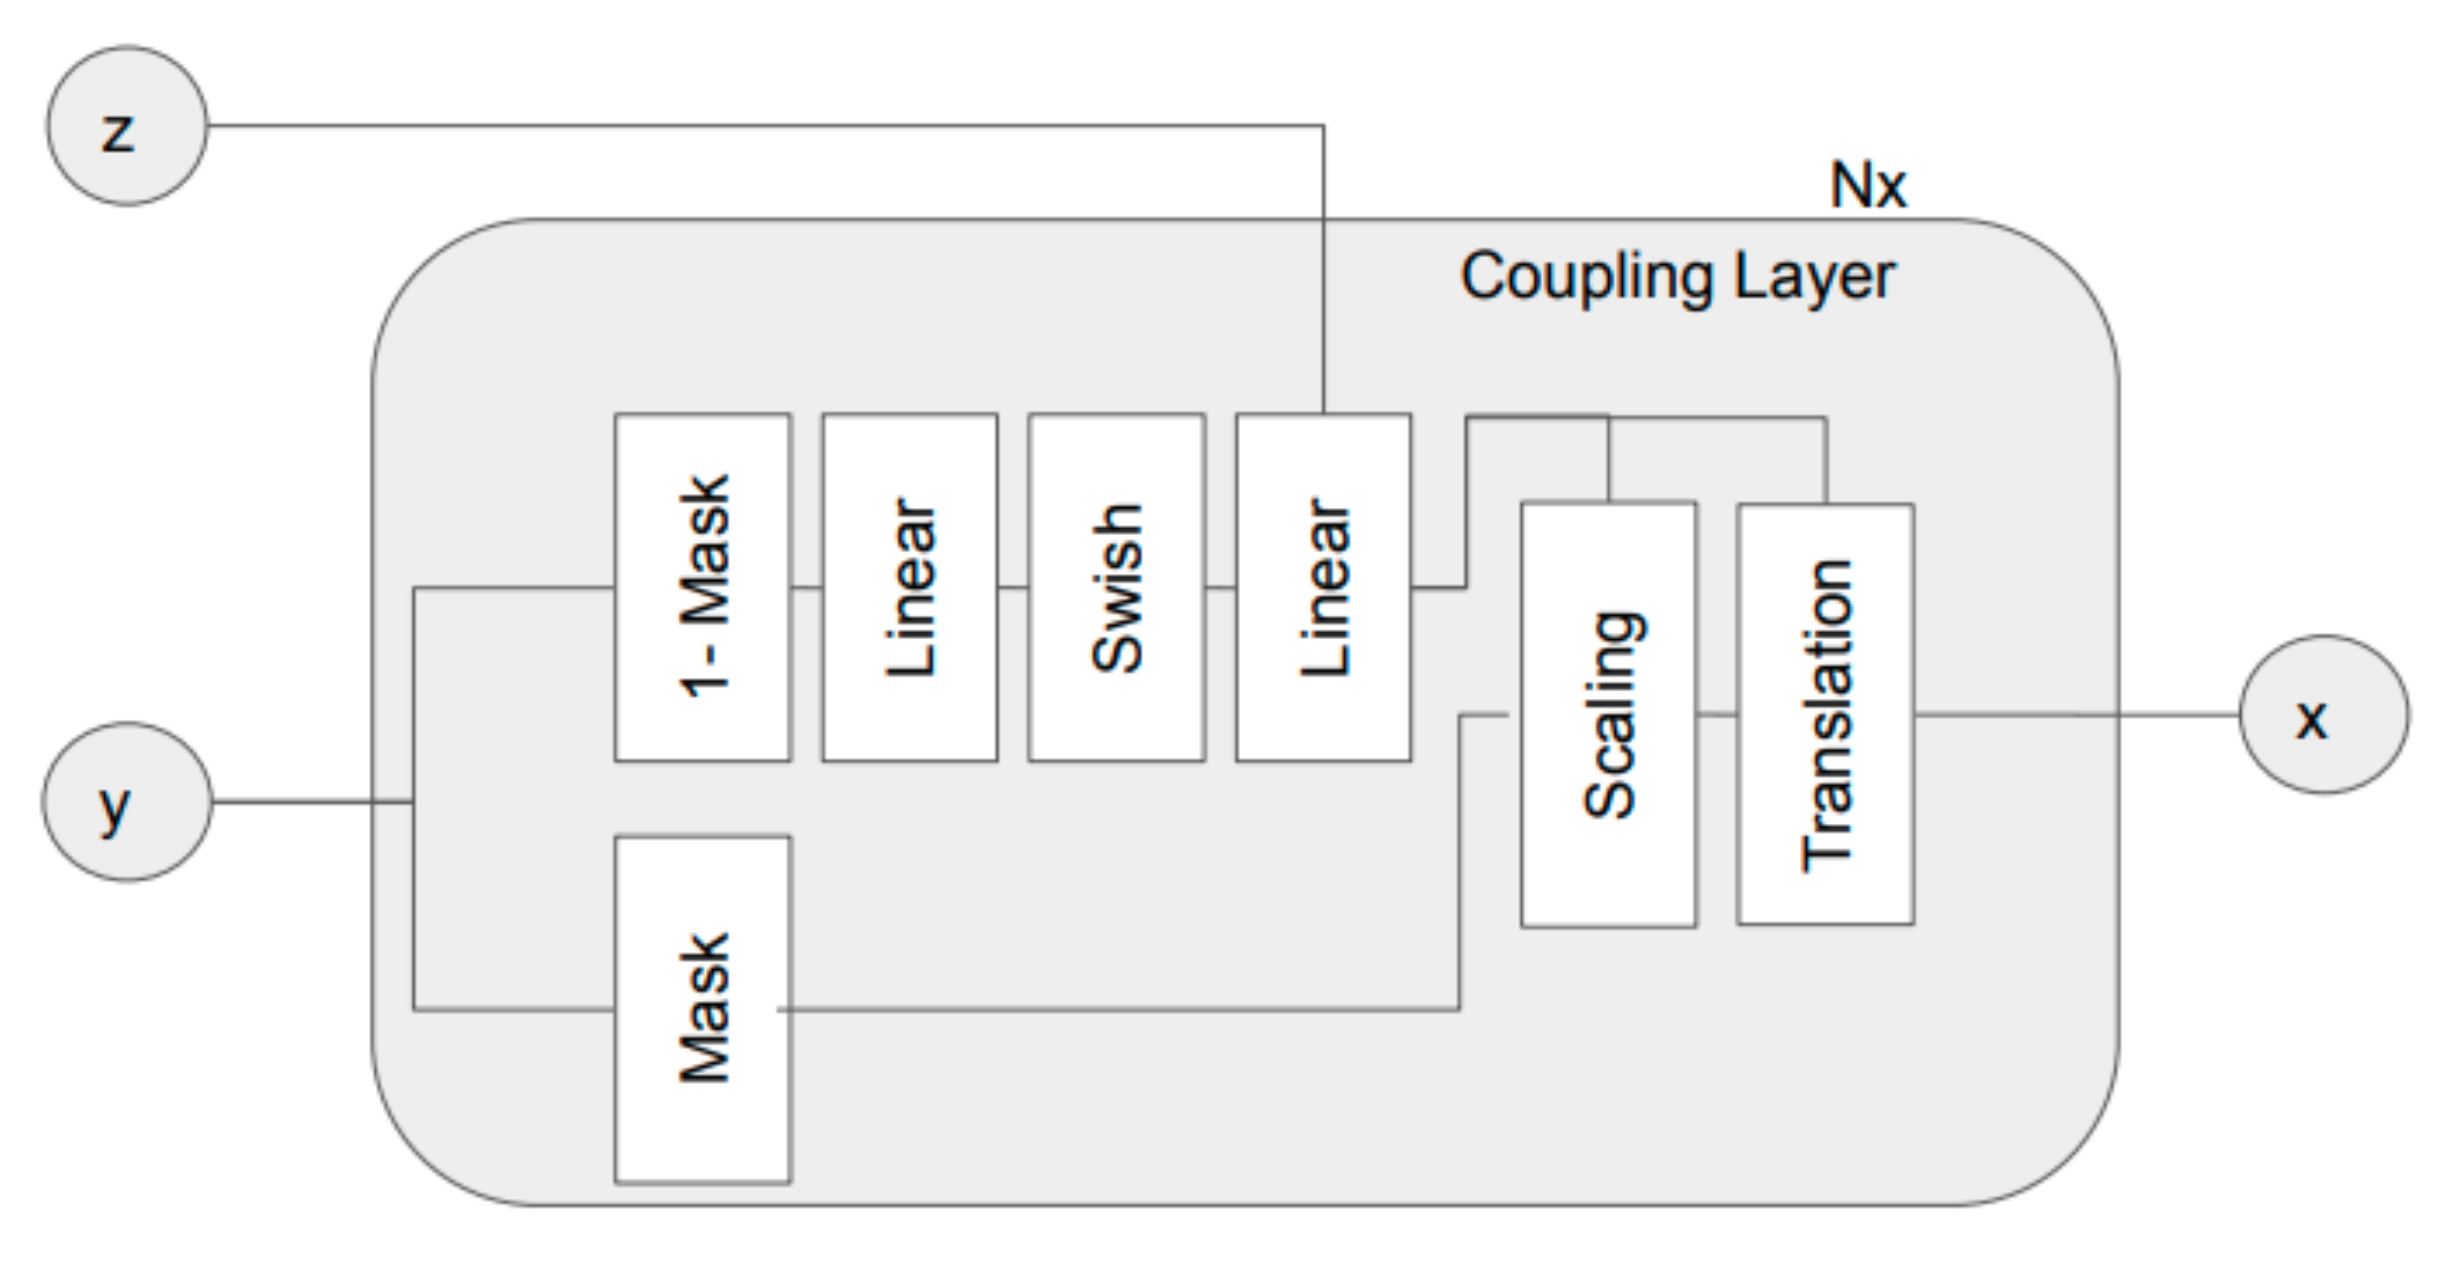}
  \caption{Basic module of RealNVP architecture used in general comparison on point cloud autoencoding.}
  \label{fig:dpf_architecture}
\end{subfigure}
\caption{Architectures used in comparison in \secref{subsubsection:softflow} (a) and \secref{subsection:pc_autoencoding}. We use N=8 (a) and  resp. N=63 (b) blocks.}
\label{fig:architectures}
\end{figure*}

\subsubsection{Training Details}

\paragraph{Artificial Data.} We train the RealNVP for 5000 iterations with a batch size of 128 on randomly drawn samples from the aforementioned distributions. We use the Adam~\cite{kingma2014adam} optimizer and an initial learning rate of $10^{-3}$ which we half after 2500 iterations. 

\paragraph{Comparison with SoftFlow}~\cite{kim2020softflow} in \secref{subsection:pc_autoencoding}. We train autoencoder for 15000 epochs using a batch size of 128 and the Adam optimizer with an initial learning rate of $10^{-3}$. We multiply the learning rate by a factor of $0.24$ after 5000 and 10000 epochs. When training a \ac{nf} absent of the SoftFlow framework we add noise of the magnitude 0.02 to the data. When training with the SoftFlow framework, we follow the original implementation~\cite{kim2020softflow} and use a maximum noise standard deviation of 0.075 and a minimum noise standard deviation of 0.0.

\paragraph{General experiments on autoencoding} in \secref{subsection:pc_autoencoding}. We train the RealNVP for 1500 epochs using a batch size of 128 and the Adam optimizer with an initial learning rate of $6.4\times 10^{-4}$ which we multiply with 0.25 after 1200 and 1400 epochs. Additionally, we vary the magnitude of noise added to the point clouds over the process of the training. Initially, we train with a Gaussian noise of standard deviation $\sigma=0.25$ for the first 100 epochs. Then, we exponentially decay the standard deviation of the noise to $\sigma=0.02$ between epoch 100 and epoch 1200. Afterwards we fix $\sigma=0.02$.
