# Supplementary material for: ManiFlow: Implicitly Representing Manifolds with Normalizing Flows
Source: arXiv:2208.08932 source file (2022-08-18)
Supplement: Supplementary file 3 [file car_supplement.tex]

\begin{figure*}[t]
\begin{center}

    \renewcommand{\figsize}{0.15}
    \newcommand{\carsize}{3.5}
    
    \begin{tabular}{ c c c c c }
    \setlength{\tabcolsep}{0pt} % Default value: 6pt
     % Default value: 1
    
        \centering 
    
      GT  & DPM~\cite{luo2021diffusion} & NF & NF\textsubscript{LLM} & NF\textsubscript{LL-Poisson} \\
      
      \includegraphics[width=\figsize\linewidth,trim={\carsize cm \carsize cm \carsize cm \carsize cm},clip]{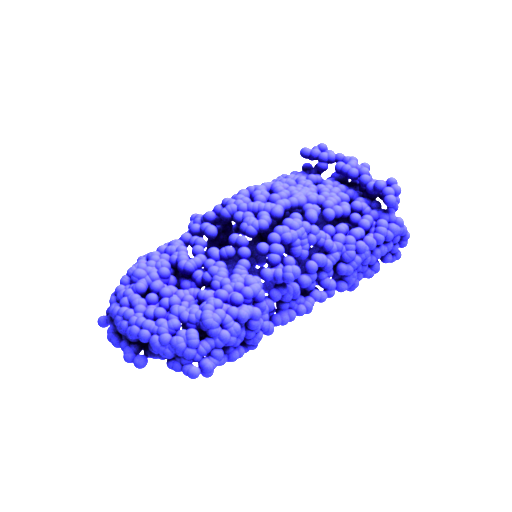} &
      \includegraphics[width=\figsize\linewidth,trim={\carsize cm \carsize cm \carsize cm \carsize cm},clip]{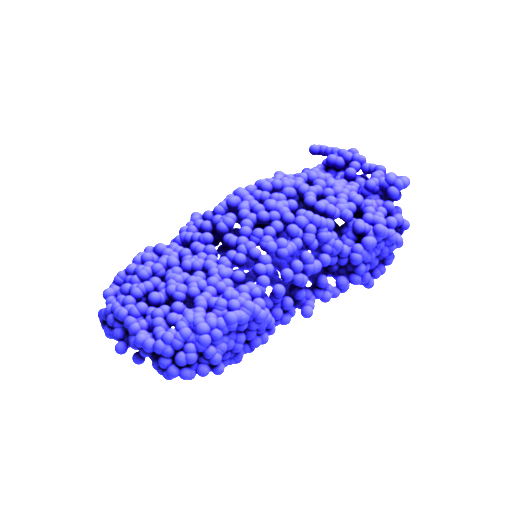} &
      \includegraphics[width=\figsize\linewidth,trim={\carsize cm \carsize cm \carsize cm \carsize cm},clip]{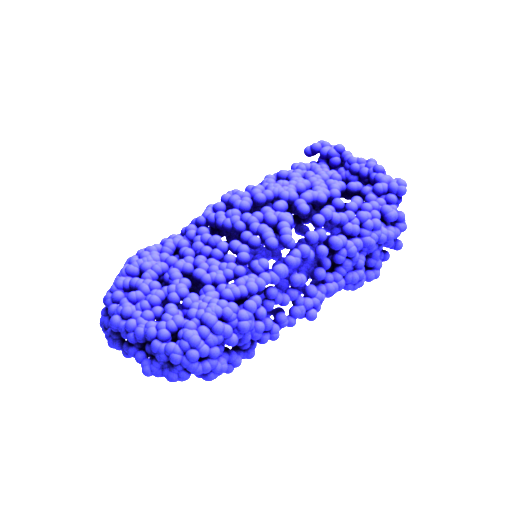} &
      \includegraphics[width=\figsize\linewidth,trim={\carsize cm \carsize cm \carsize cm \carsize cm},clip]{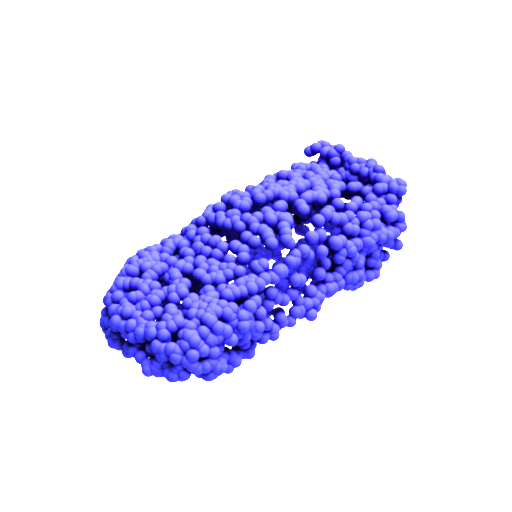} &
      \includegraphics[width=\figsize\linewidth,trim={\carsize cm \carsize cm \carsize cm \carsize cm},clip]{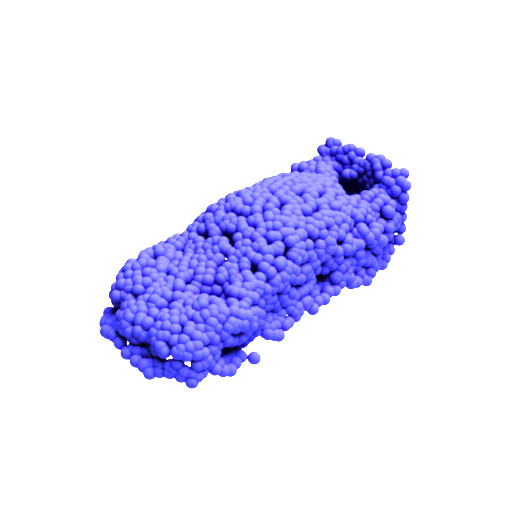} \\
      
      \includegraphics[width=\figsize\linewidth,trim={\carsize cm \carsize cm \carsize cm \carsize cm},clip]{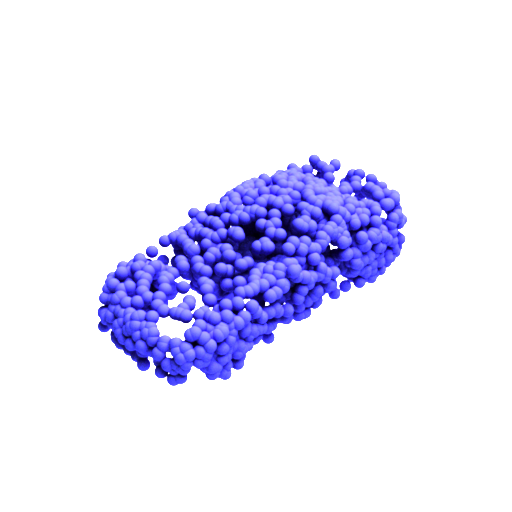} &
      \includegraphics[width=\figsize\linewidth,trim={\carsize cm \carsize cm \carsize cm \carsize cm},clip]{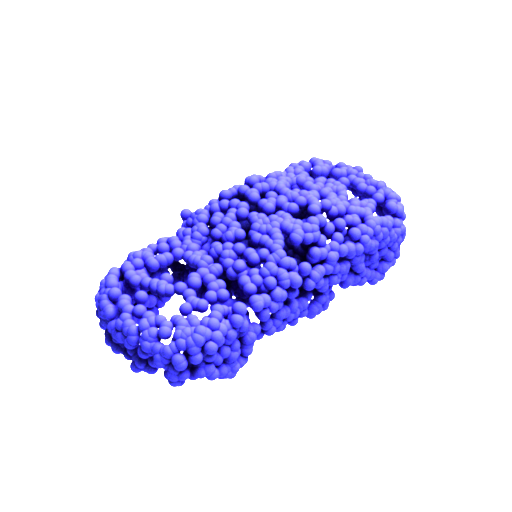} &
      \includegraphics[width=\figsize\linewidth,trim={\carsize cm \carsize cm \carsize cm \carsize cm},clip]{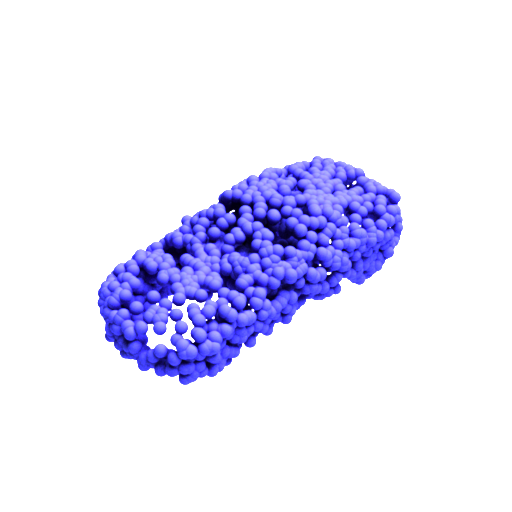} &
      \includegraphics[width=\figsize\linewidth,trim={\carsize cm \carsize cm \carsize cm \carsize cm},clip]{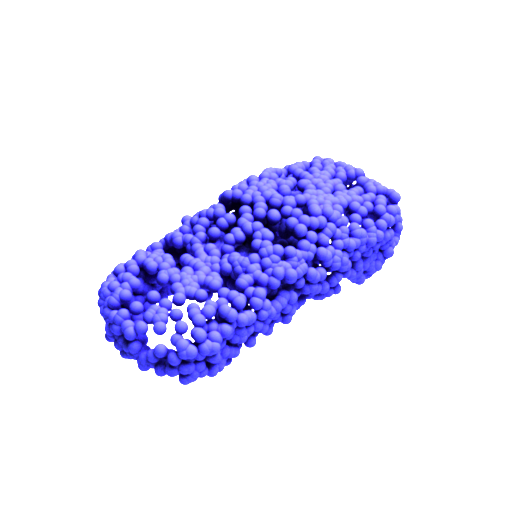} &
      \includegraphics[width=\figsize\linewidth,trim={\carsize cm \carsize cm \carsize cm \carsize cm},clip]{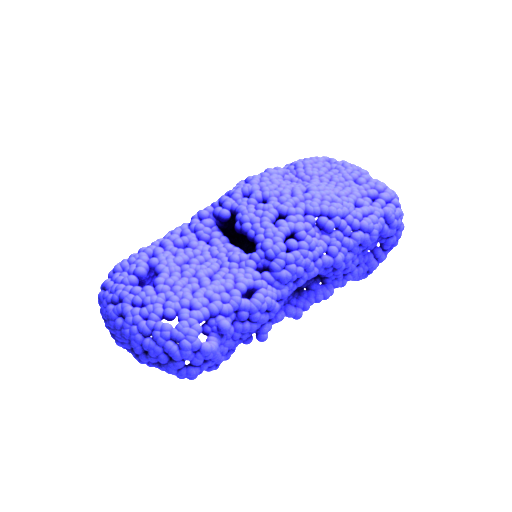} \\
      
      \includegraphics[width=\figsize\linewidth,trim={\carsize cm \carsize cm \carsize cm \carsize cm},clip]{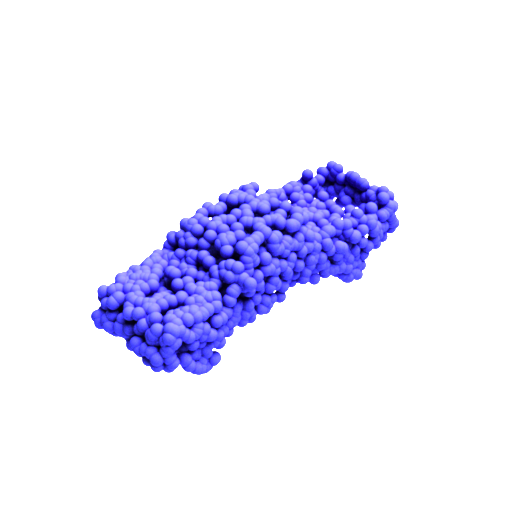} &
      \includegraphics[width=\figsize\linewidth,trim={\carsize cm \carsize cm \carsize cm \carsize cm},clip]{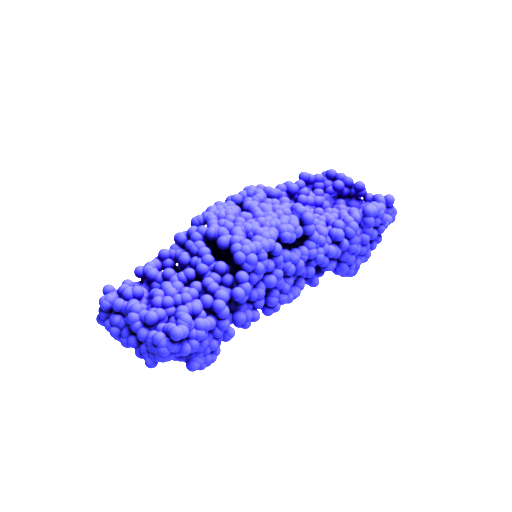} &
      \includegraphics[width=\figsize\linewidth,trim={\carsize cm \carsize cm \carsize cm \carsize cm},clip]{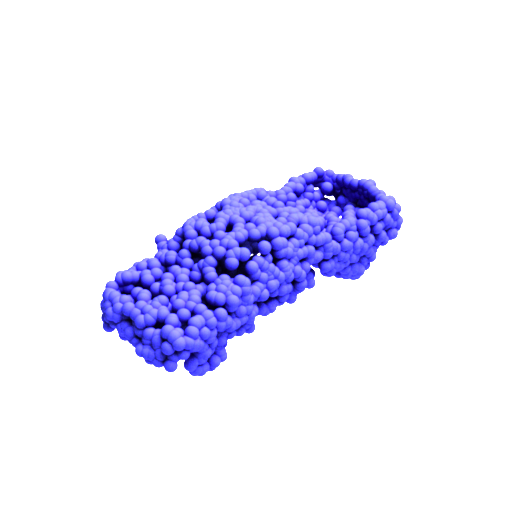} &
      \includegraphics[width=\figsize\linewidth,trim={\carsize cm \carsize cm \carsize cm \carsize cm},clip]{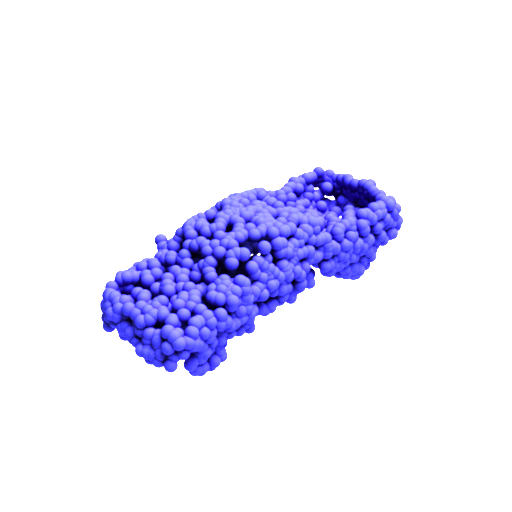} &
      \includegraphics[width=\figsize\linewidth,trim={\carsize cm \carsize cm \carsize cm \carsize cm},clip]{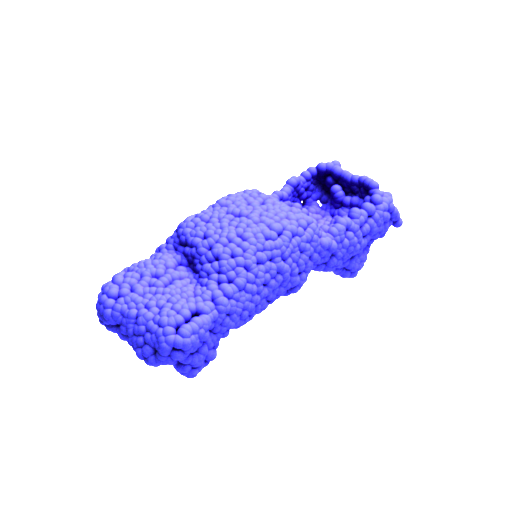} \\
      
    \end{tabular}
    
\end{center}
\caption{Further qualitative results on the car category of the ground truth (GT), DPM~\cite{luo2021diffusion}, a RealNVP (NF) and a RealNVP with LLM/LL-Poisson (NF\textsubscript{LLM}/NF\textsubscript{LL-Poisson}).}\label{fig:car_supplement}
\end{figure*}
