# Supplementary material for: ManiFlow: Implicitly Representing Manifolds with Normalizing Flows
Source: arXiv:2208.08932 source file (2022-08-18)
Supplement: Supplementary file 6 [file llm.tex]

\begin{figure}[t!]
\centering
\begin{subfigure}{.49\textwidth}
  \centering
  \includegraphics[width=1.0\linewidth]{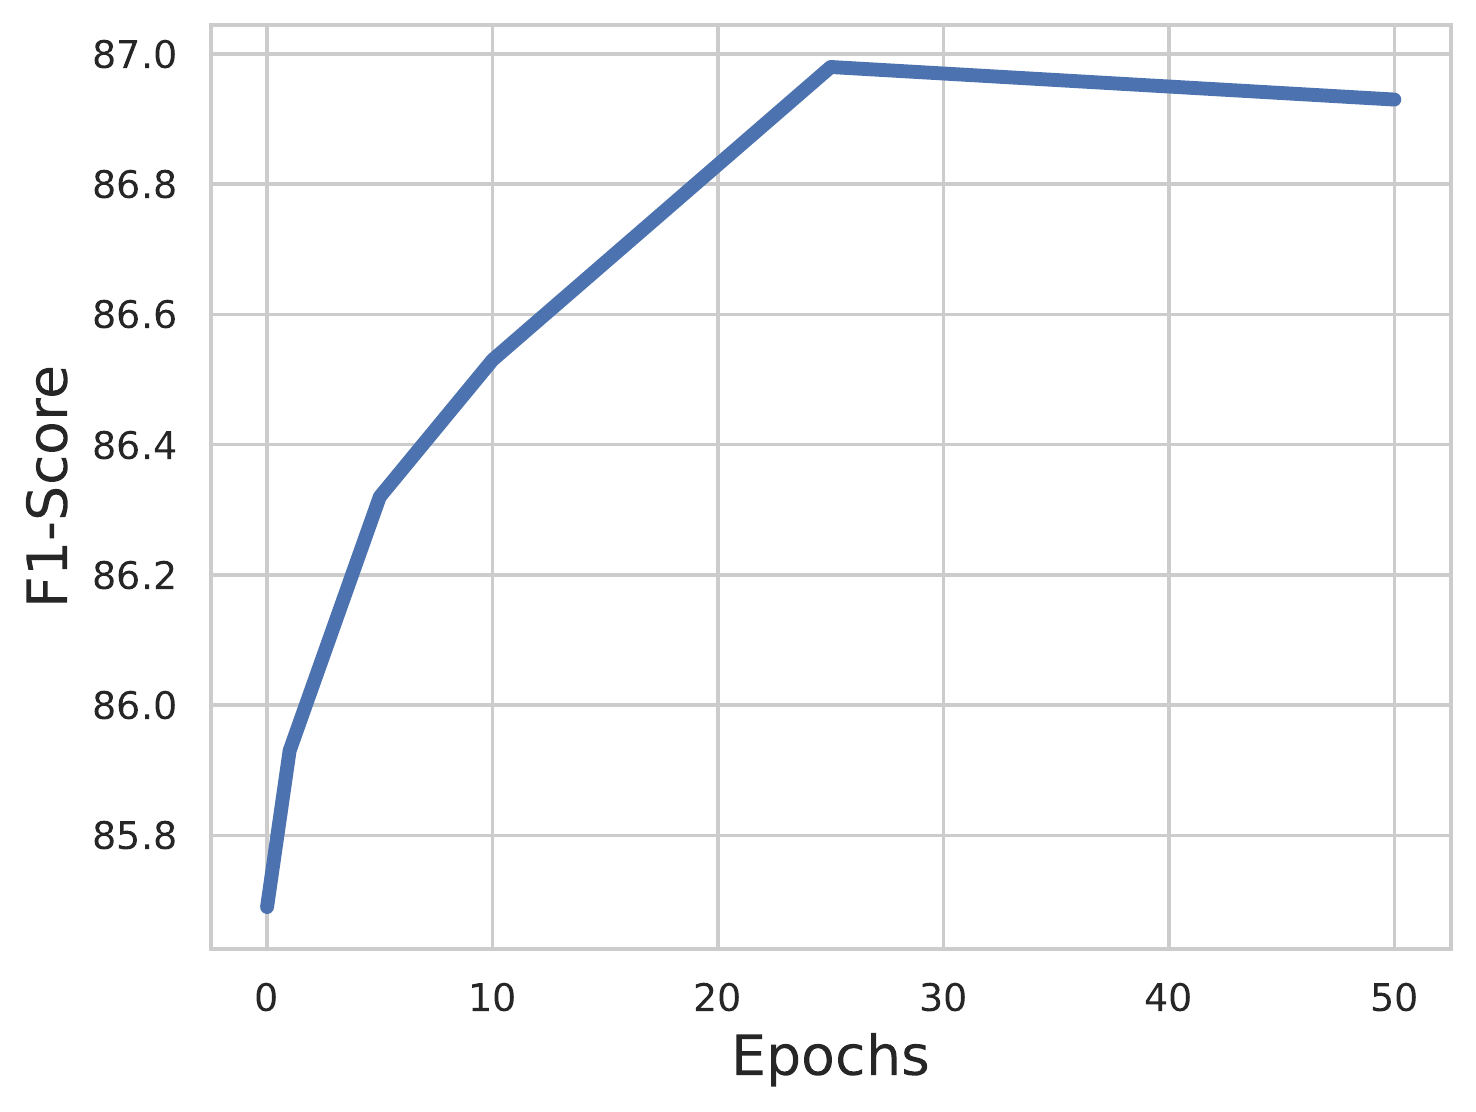}
  \caption{F1-Score depending on the number of epochs used for ManiFlow-LLM.}.
  \label{fig:f1_vs_epochs}
\end{subfigure}%
\\
\begin{subfigure}{.49\textwidth}
  \centering
  \includegraphics[width=1.0\linewidth]{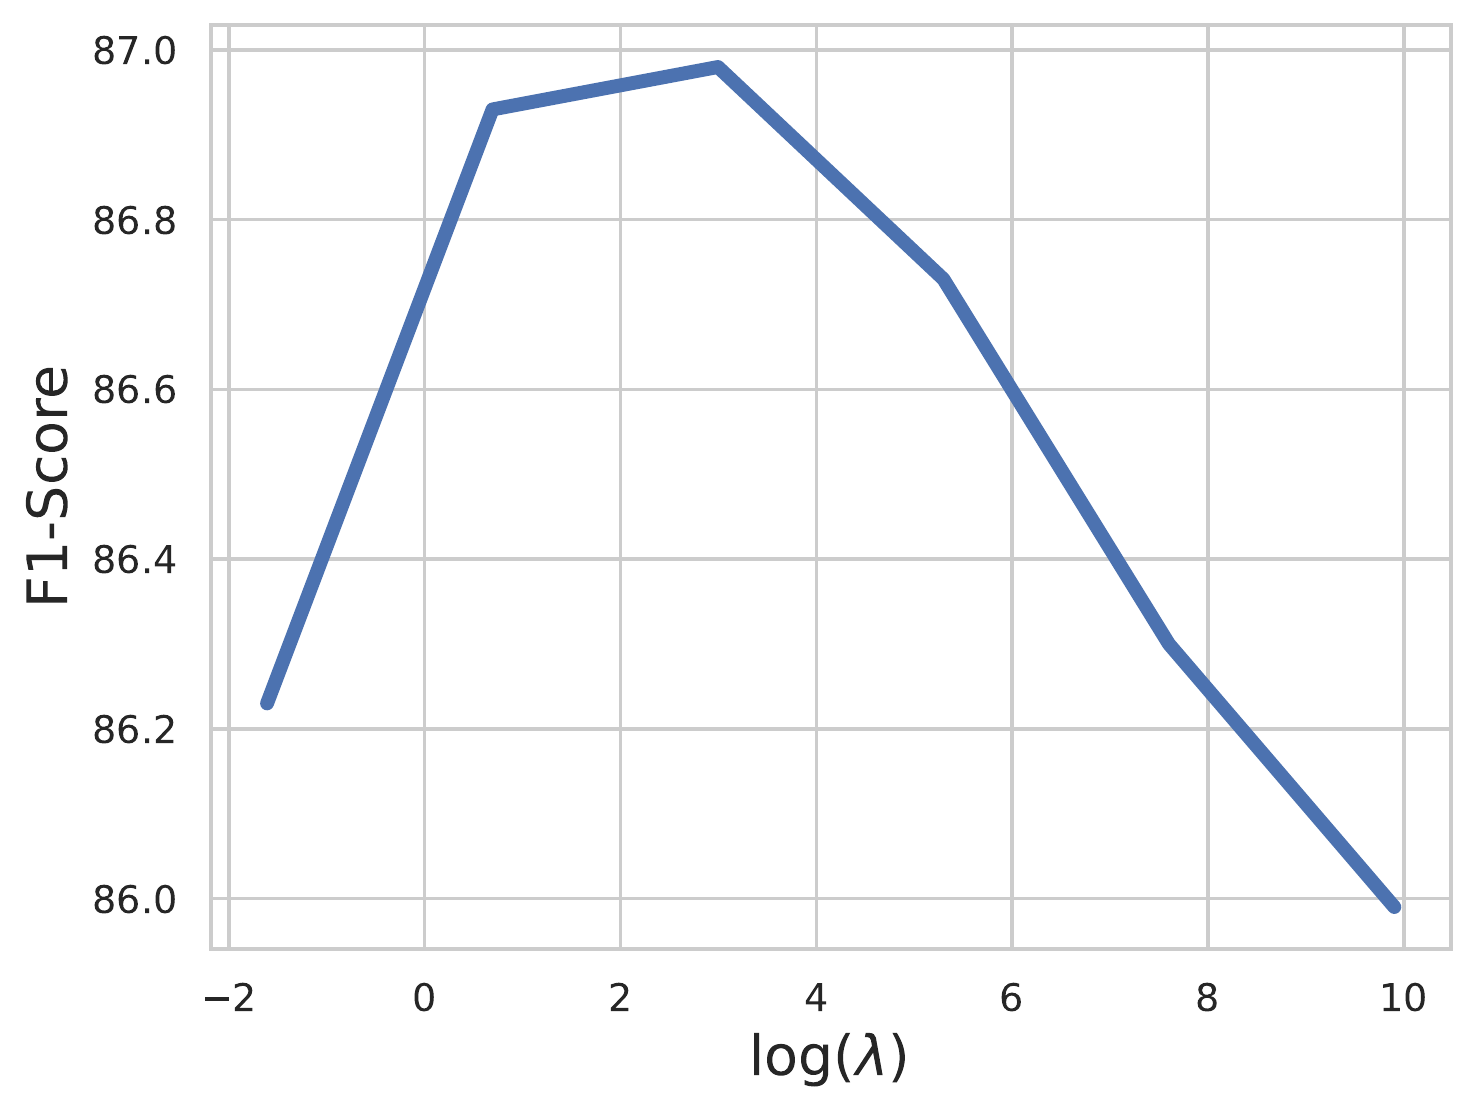}
  \caption{F1-Score depending on the on the logarithm of the weight $\lambda$ used for ManiFlow-LLM.}
  \label{fig:f1_vs_dweight}
\end{subfigure}
\caption{Analysis of the sensitivity of ManiFlow-LLM to the number of epochs (a) and the magnitude of $\lambda$ (b) on the airplane category.}
\label{fig:llm_ablation}
\end{figure}
