# Supplementary material for: ManiFlow: Implicitly Representing Manifolds with Normalizing Flows
Source: arXiv:2208.08932 source file (2022-08-18)
Supplement: Supplementary file 7 [file llpoisson.tex]

\begin{figure}
\centering
\begin{subfigure}{.49\textwidth}
  \centering
  \includegraphics[width=1.0\linewidth]{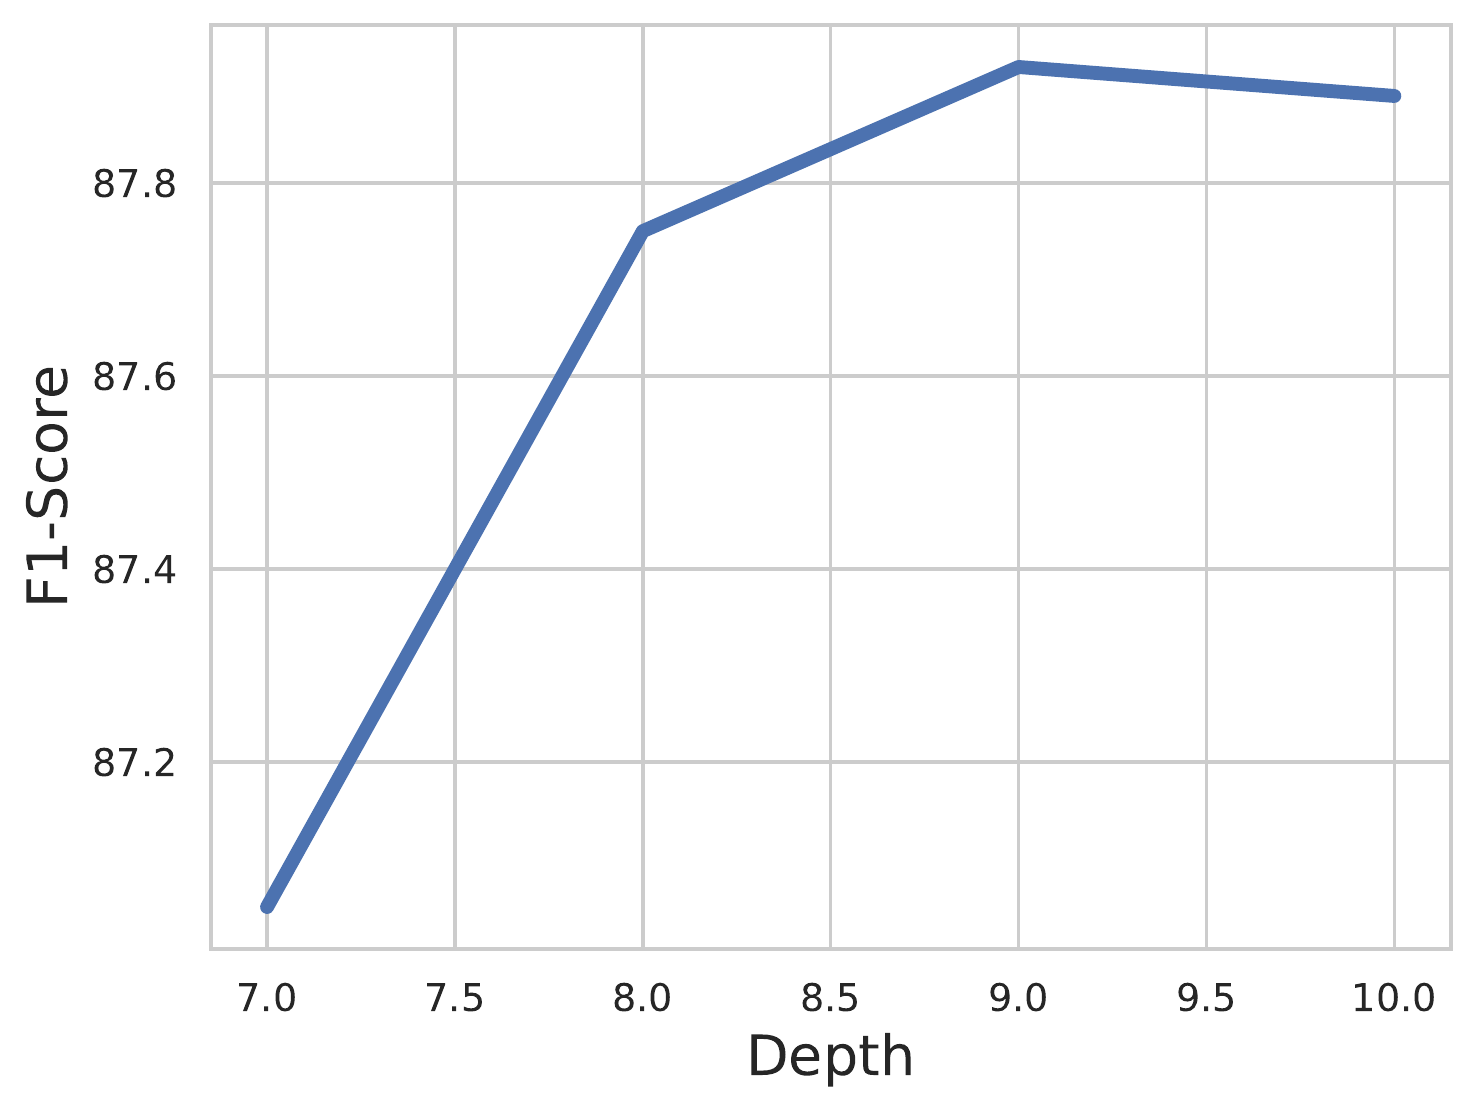}
  \caption{F1-Score depending on the depth used in Poisson surface reconstruction.}.
  \label{fig:f1_vs_dpoisson}
\end{subfigure}%
\\
\begin{subfigure}{.49\textwidth}
  \centering
  \includegraphics[width=1.0\linewidth]{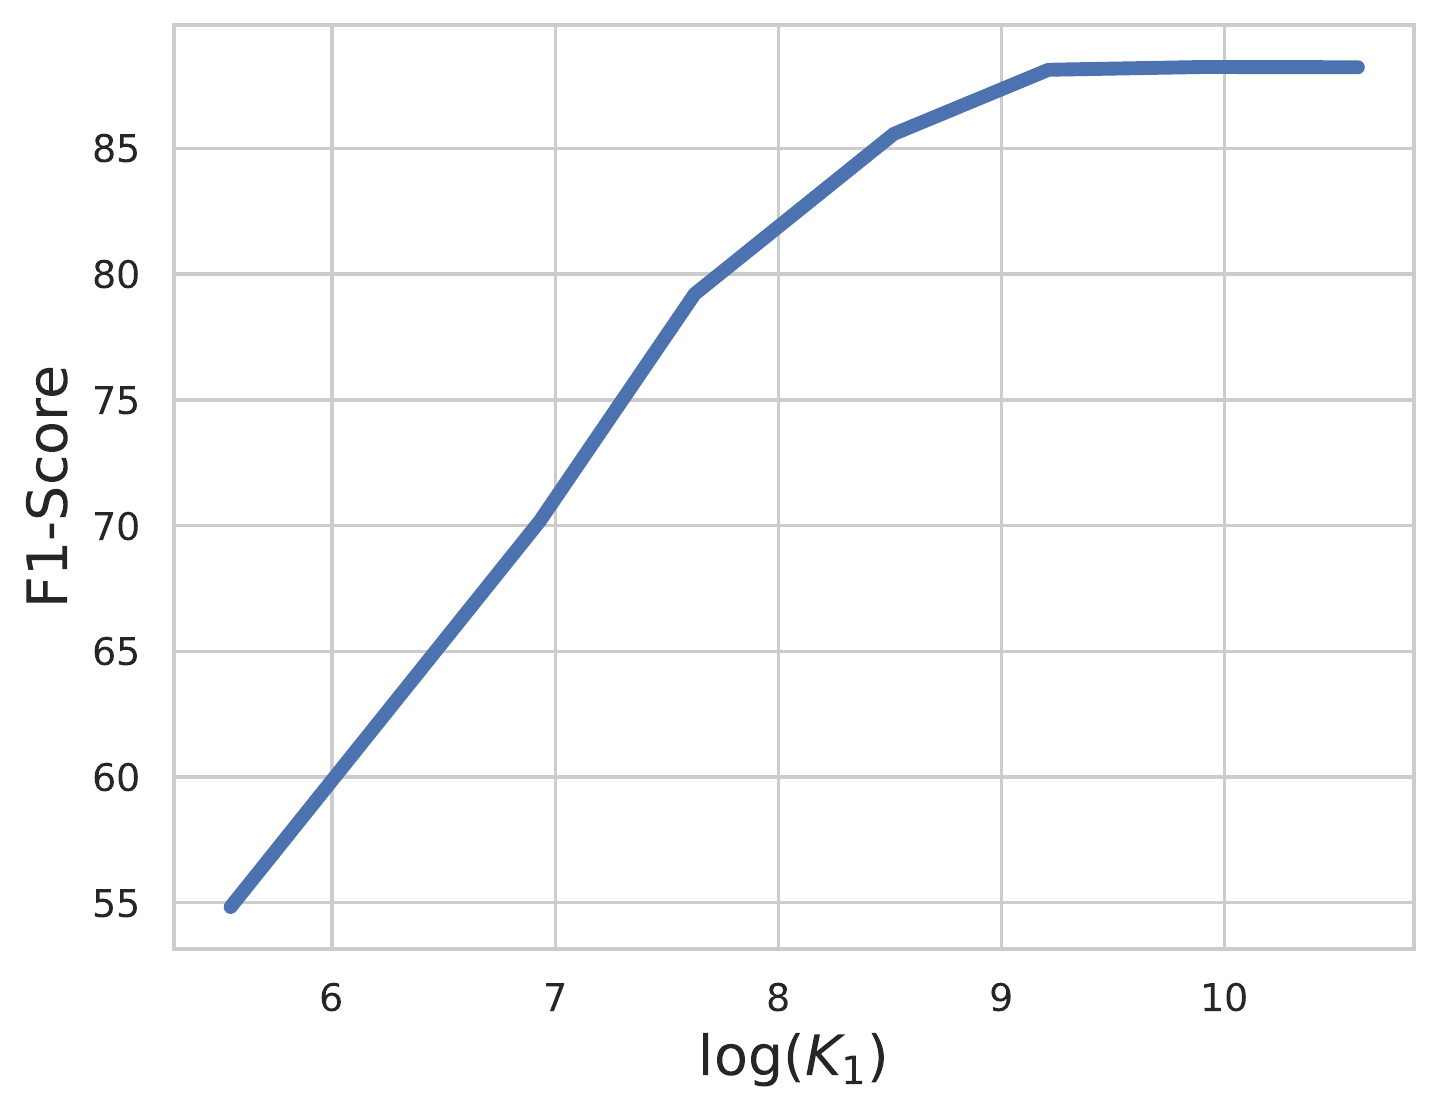}
  \caption{F1-Score depending on the on the logarithm of the number of points K\textsubscript{1}.}
  \label{fig:f1_vs_nr_points}
\end{subfigure}
\caption{Analysis of the sensitivity of ManiFlow-LL-Poisson to the depth used for Poisson surface reconstruction (a) and the number of points K\textsubscript{1} (b) on the airplane category.}
\label{fig:llpoisson_ablation}
\end{figure}
