# Supplementary material for: ManiFlow: Implicitly Representing Manifolds with Normalizing Flows
Source: arXiv:2208.08932 source file (2022-08-18)
Supplement: Supplementary file 8 [file ablation.tex]

We analyse the sensitivity of LLM/LL-Poisson to its hyperparameters. We perform this anaysis on the task of point cloud autoencoding and use the RealNVP trained on the airplane category in \secref{subsection:pc_autoencoding}. For LLM we plot the F1-score against the number of epochs used to optimize \eref{eq:optimization_criterion} and the logarithm of the magnitude of the weight $\lambda$. For LL-Poisson we plot the F1-score against the depth used for Poisson surface reconstruction and the logarithm of the number of points K\textsubscript{1} sampled prior to surface reconstruction. \figref{fig:llm_ablation} and \figref{fig:llpoisson_ablation} depict the results. While there exists an optimal $\lambda$, we find that the other hyperparameters typically lead to saturating performance given a sufficient magnitude.

\begin{figure}[t!]
\centering
\begin{subfigure}{.49\textwidth}
  \centering
  \includegraphics[width=1.0\linewidth]{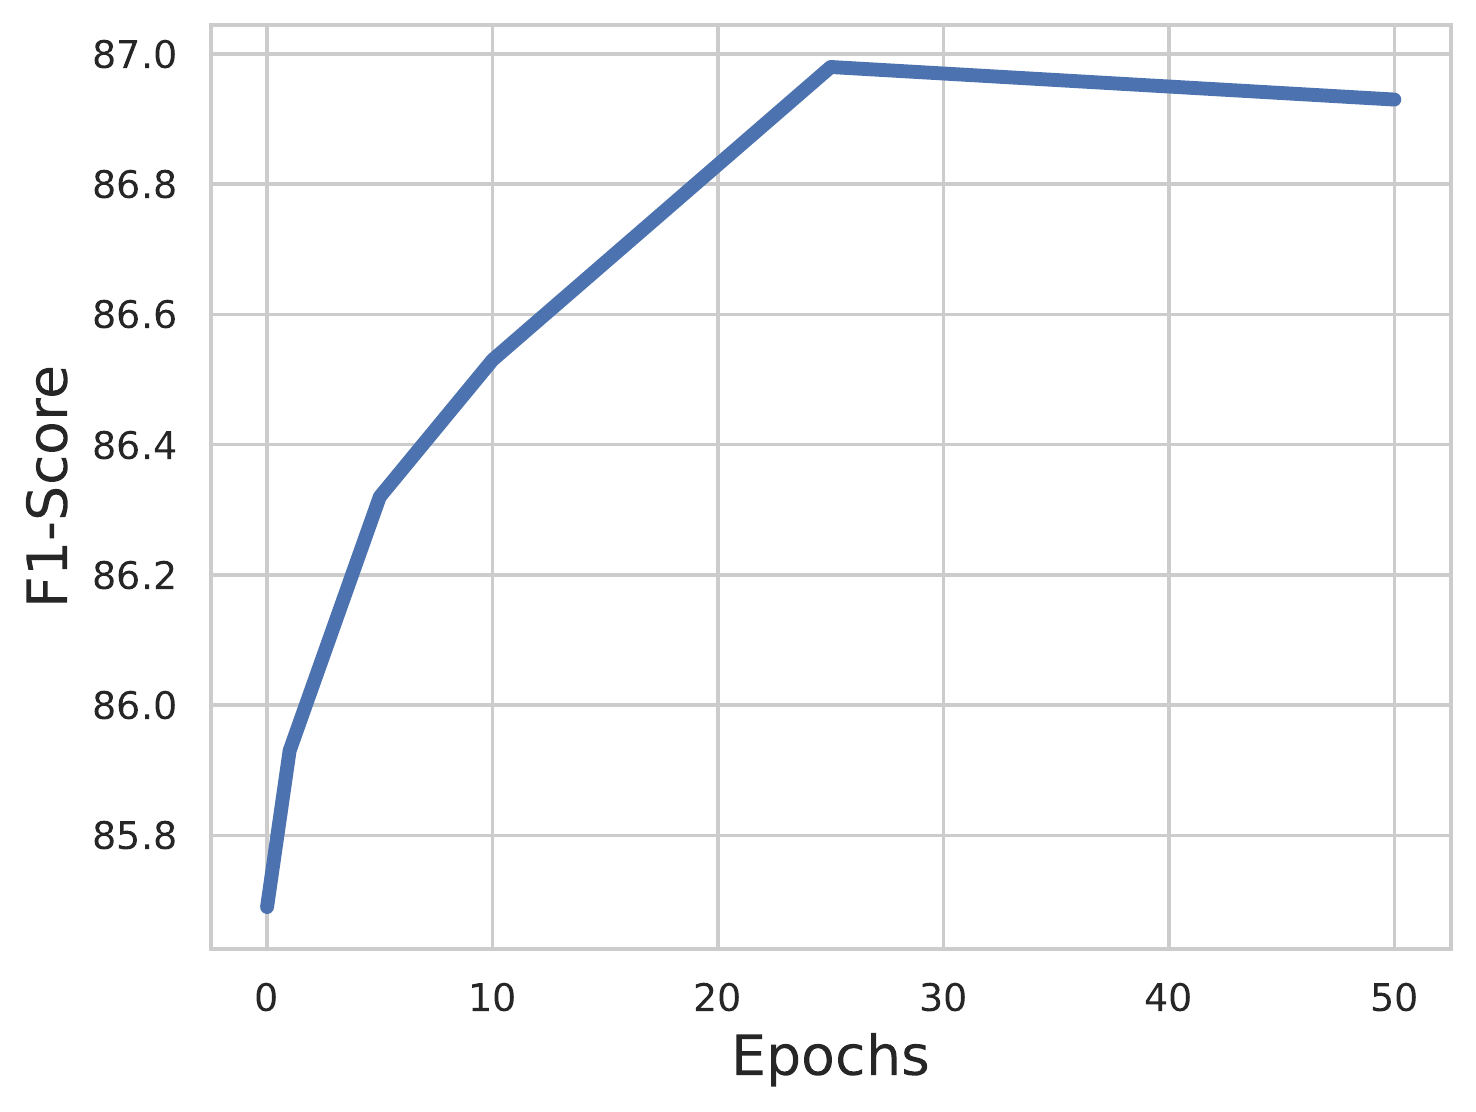}
  \caption{F1-Score depending on the number of epochs used for ManiFlow-LLM.}.
  \label{fig:f1_vs_epochs}
\end{subfigure}%
\\
\begin{subfigure}{.49\textwidth}
  \centering
  \includegraphics[width=1.0\linewidth]{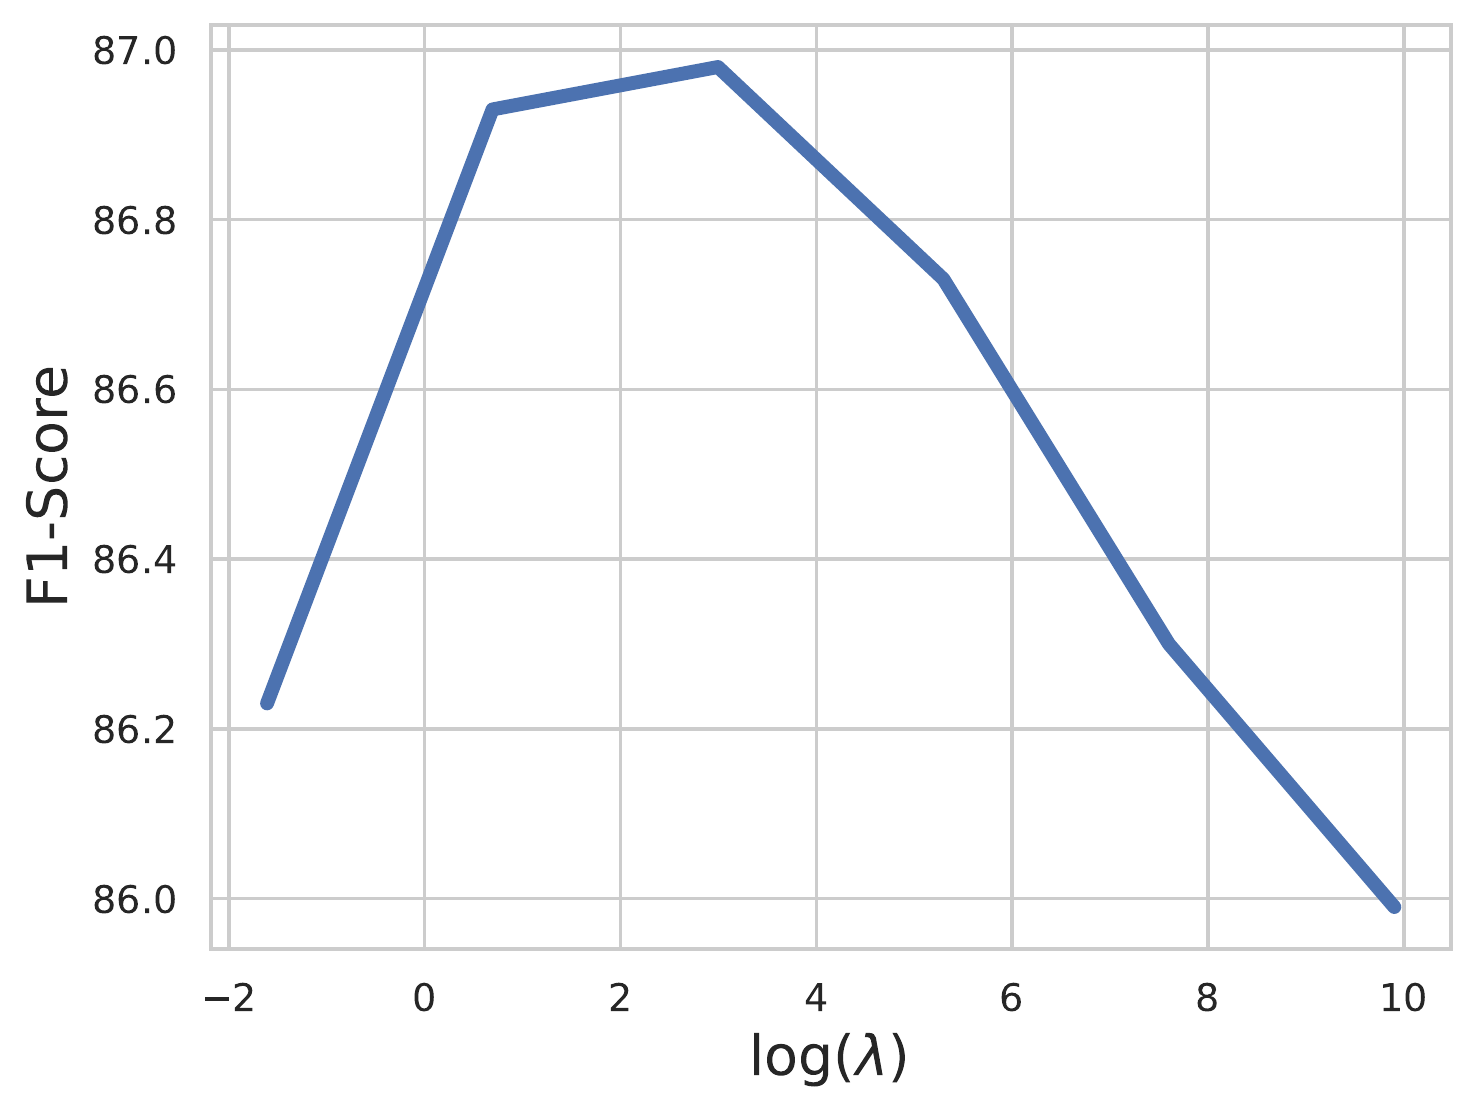}
  \caption{F1-Score depending on the on the logarithm of the weight $\lambda$ used for ManiFlow-LLM.}
  \label{fig:f1_vs_dweight}
\end{subfigure}
\caption{Analysis of the sensitivity of ManiFlow-LLM to the number of epochs (a) and the magnitude of $\lambda$ (b) on the airplane category.}
\label{fig:llm_ablation}
\end{figure}

\begin{figure}
\centering
\begin{subfigure}{.49\textwidth}
  \centering
  \includegraphics[width=1.0\linewidth]{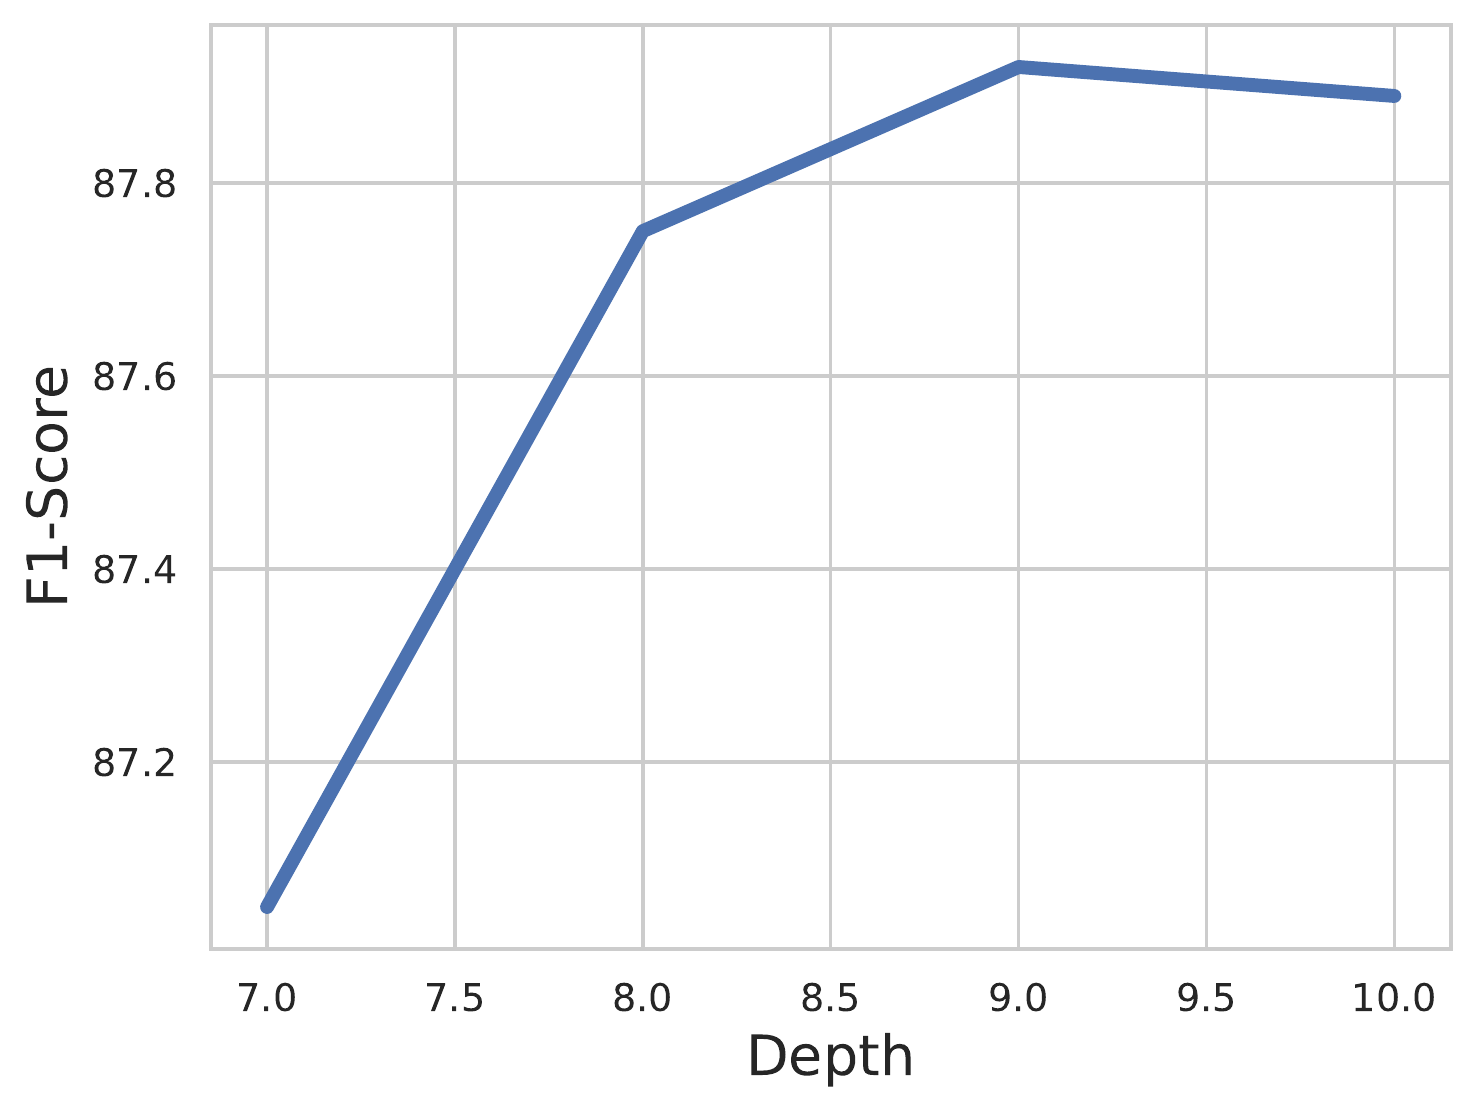}
  \caption{F1-Score depending on the depth used in Poisson surface reconstruction.}.
  \label{fig:f1_vs_dpoisson}
\end{subfigure}%
\\
\begin{subfigure}{.49\textwidth}
  \centering
  \includegraphics[width=1.0\linewidth]{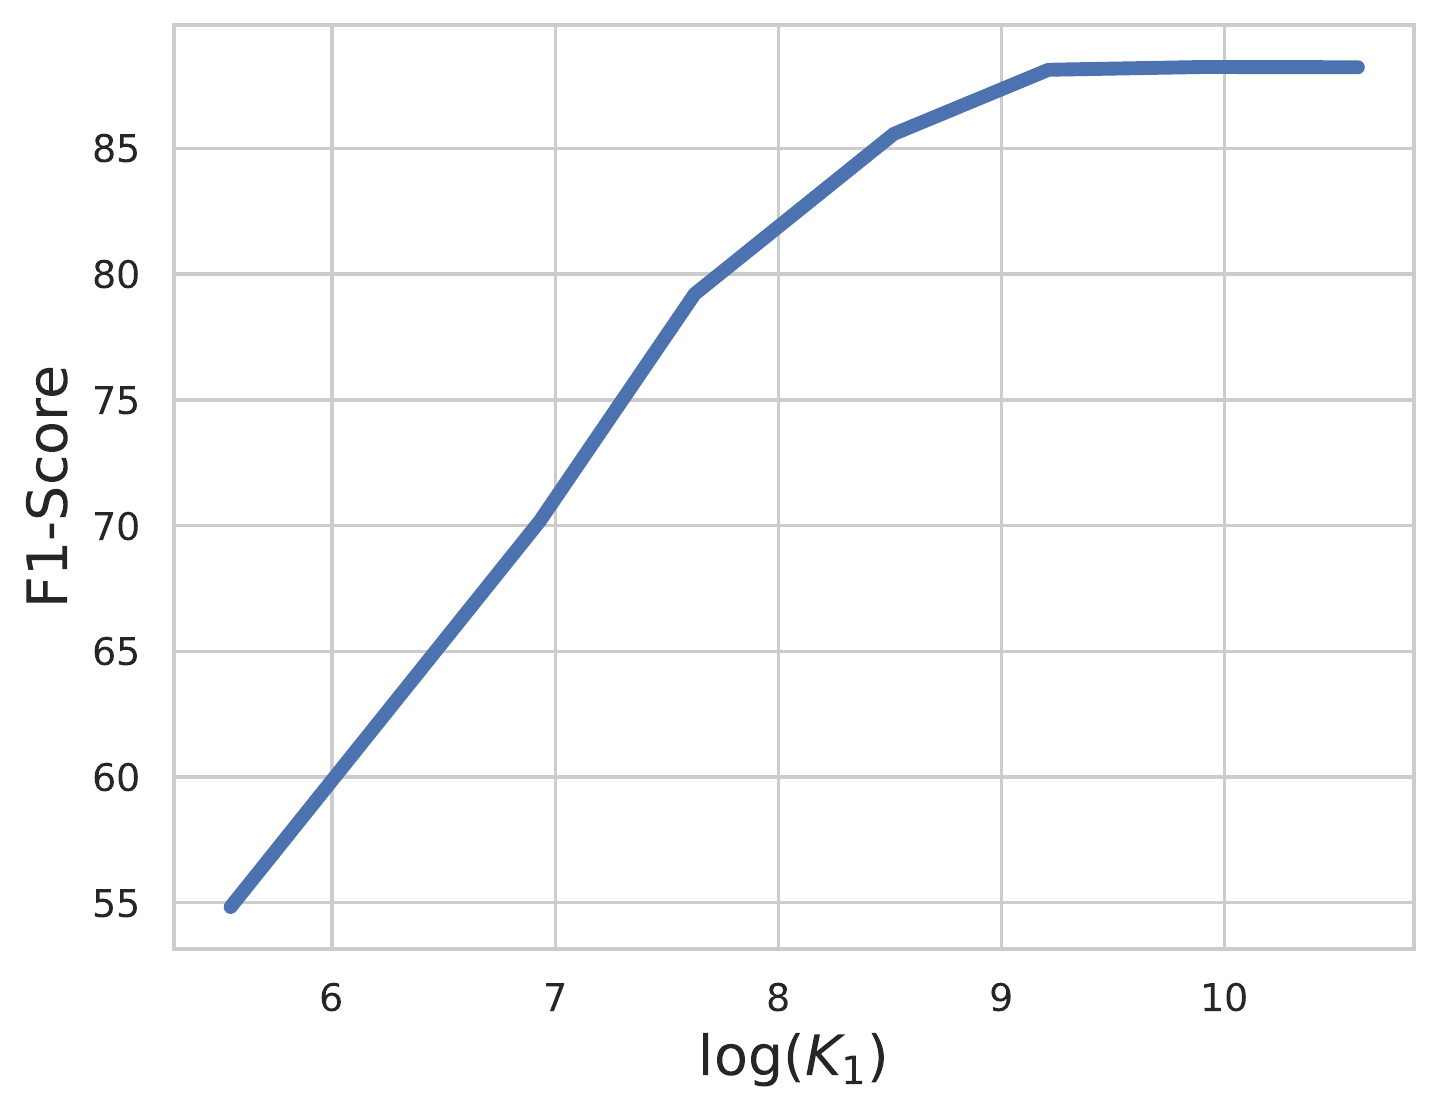}
  \caption{F1-Score depending on the on the logarithm of the number of points K\textsubscript{1}.}
  \label{fig:f1_vs_nr_points}
\end{subfigure}
\caption{Analysis of the sensitivity of ManiFlow-LL-Poisson to the depth used for Poisson surface reconstruction (a) and the number of points K\textsubscript{1} (b) on the airplane category.}
\label{fig:llpoisson_ablation}
\end{figure}
