# Supplementary material for: ManiFlow: Implicitly Representing Manifolds with Normalizing Flows
Source: arXiv:2208.08932 source file (2022-08-18)
Supplement: Supplementary file 9 [file experimental_details.tex]

\subsubsection{Architecture of Normalizing Flows}

\paragraph{Experiments on Artificial Data.} We train a RealNVP~\cite{dinh2016density} comprised of 5 coupling layers. Each coupling layer is comprised of two linear layers with a relu activation function and 128 hidden dimensions between them. We mask dimensions of the 2D data alternatingly.

\paragraph{Comparison with SoftFlow}~\cite{kim2020softflow} in \secref{subsection:pc_autoencoding}. We apply the architecture proposed in the original work~\cite{kim2020softflow}. The decoder \ac{nf} is comprised of a sequence of 8 identical modules. This module is depicted in \figref{fig:softflow_architecture}. Here, activation normalization (ActNorm) and invertible 1x1 convolutions are implemented according to GLOW~\cite{kingma2018glow}. 1x1 convolutions are enforced to be invertible by parameterizing the kernel using the LU-decomposition~\cite{kingma2018glow}. The invertible autoregressive layer is implemented according to~\cite{kingma2016improved}. In invertible autoregressive layers scaling and translation of each dimension are calculated autoregressively. Each autoregressive step is parameterized by a separate \ac{nn} consisting of of 4 linear layers with tanh activation functions and 256 hidden dimensions. 

\paragraph{General experiments on autoencoding} in \secref{subsection:pc_autoencoding}. Here the decoder model is implemented as a ReaLNVP~\cite{dinh2016density} consisting of 63 coupling layers. Such coupling layers are schematically depicted in \figref{fig:dpf_architecture}. A coupling layer splits the dimensions into two sets and applies the identity mapping to one set of dimensions. Further, the set of dimensions, which is mapped by the identity, is used to compute scaling and translation factors for the other set of dimensions. The computation of scaling and translation is parameterized by a \ac{nn} which consists of 2 linear layers with an intermediate Swish activation function and 64 hidden dimensions. The conditioning on the latent shape representation z is implemented by FiLM conditioning~\cite{perez2018film}.

\begin{figure*}
\centering
\begin{subfigure}{.9\textwidth}
  \centering
  \includegraphics[width=1.0\linewidth]{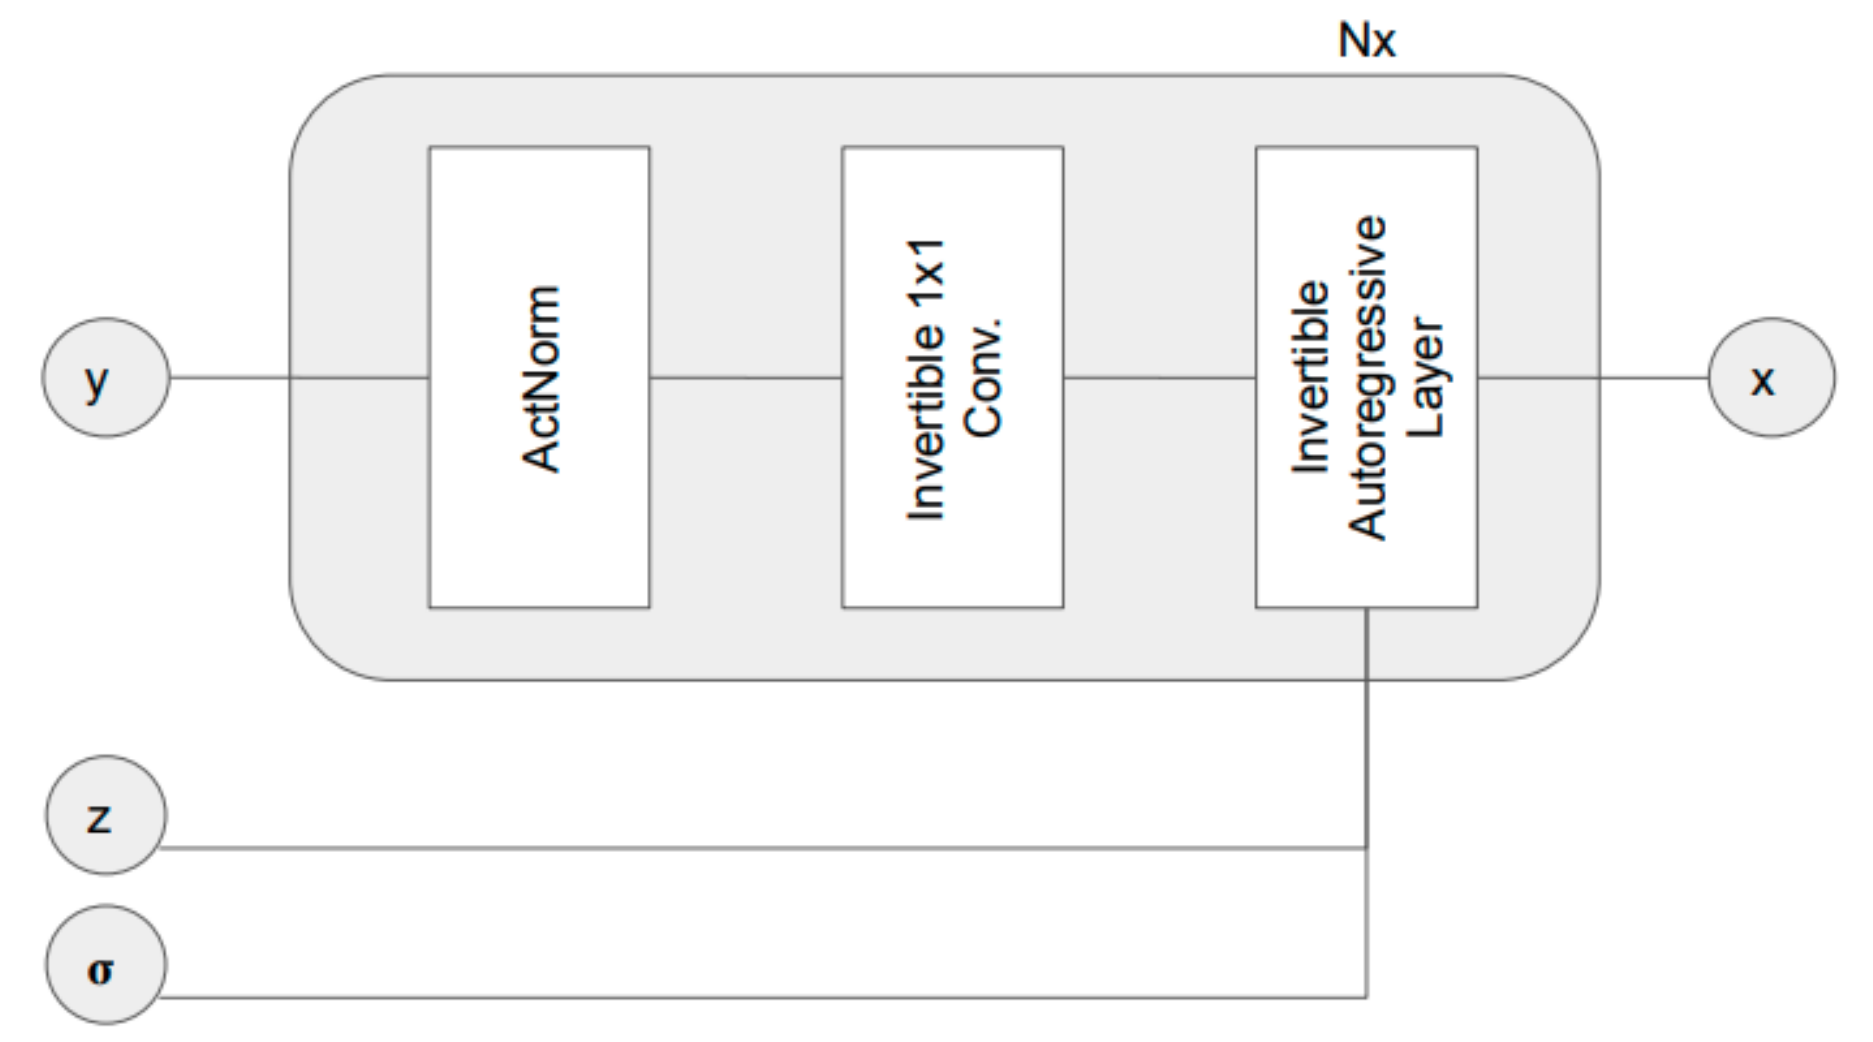}
  \caption{Basic module of architecture used in comparison with SoftFlow~\cite{kim2020softflow}.}.
  \label{fig:softflow_architecture}
\end{subfigure}%
\\
\begin{subfigure}{.9\textwidth}
  \centering
  \includegraphics[width=.9\linewidth]{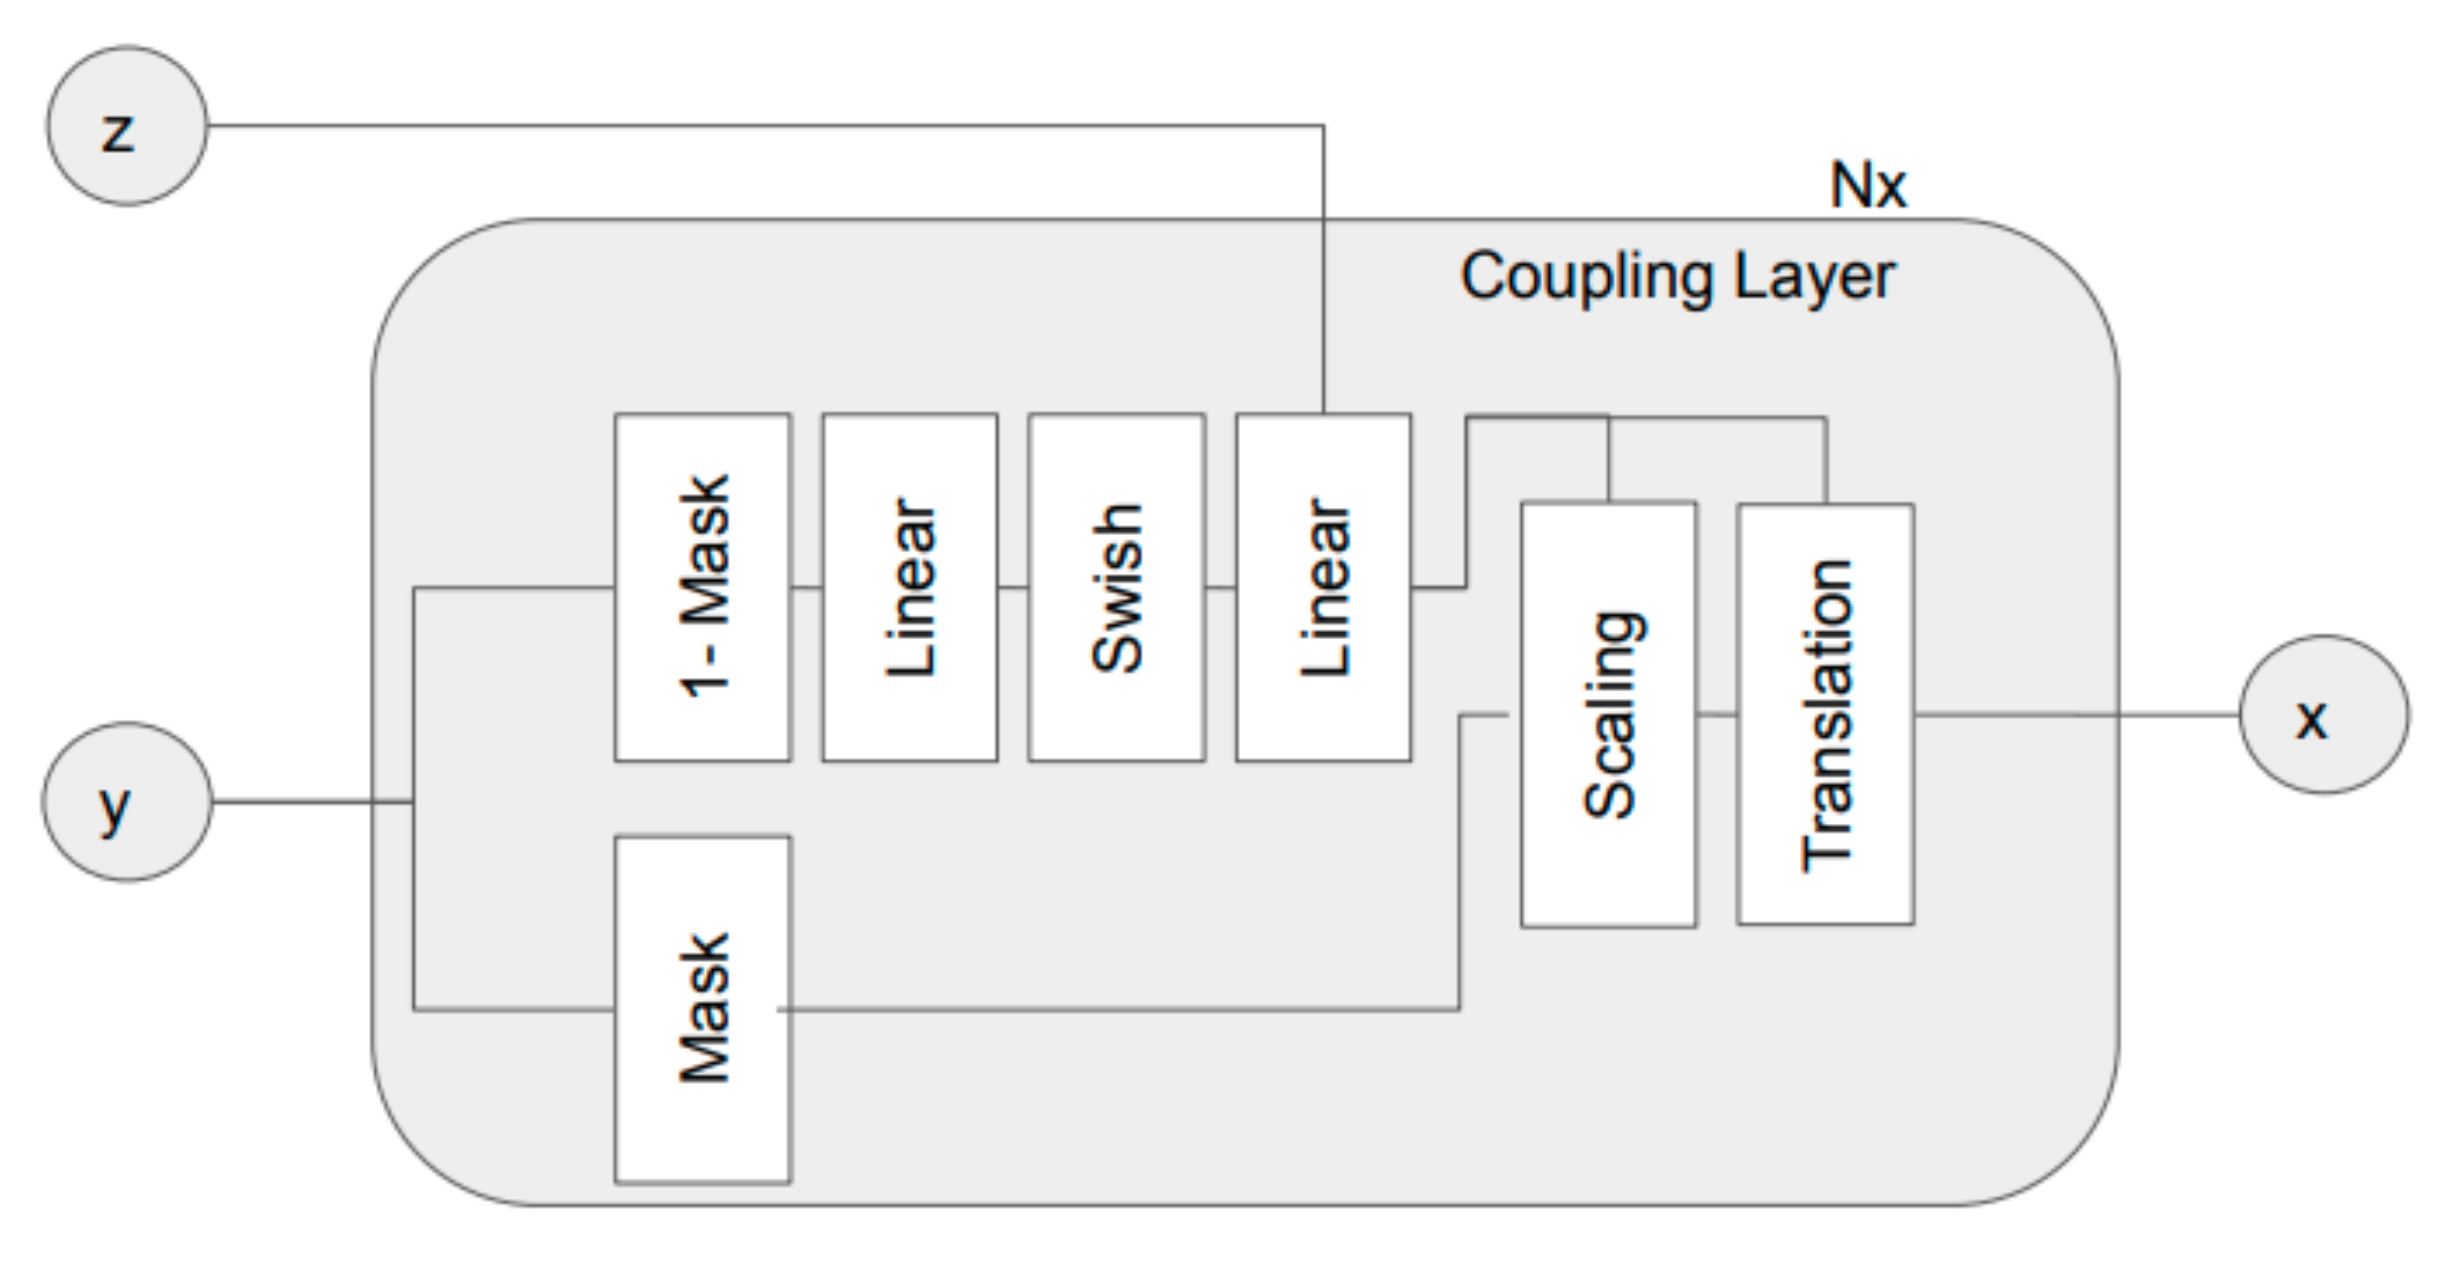}
  \caption{Basic module of RealNVP architecture used in general comparison on point cloud autoencoding.}
  \label{fig:dpf_architecture}
\end{subfigure}
\caption{Architectures used in comparison in \secref{subsubsection:softflow} (a) and \secref{subsection:pc_autoencoding}. We use N=8 (a) and  resp. N=63 (b) blocks.}
\label{fig:architectures}
\end{figure*}

\subsubsection{Training Details}

\paragraph{Artificial Data.} We train the RealNVP for 5000 iterations with a batch size of 128 on randomly drawn samples from the aforementioned distributions. We use the Adam~\cite{kingma2014adam} optimizer and an initial learning rate of $10^{-3}$ which we half after 2500 iterations. 

\paragraph{Comparison with SoftFlow}~\cite{kim2020softflow} in \secref{subsection:pc_autoencoding}. We train autoencoder for 15000 epochs using a batch size of 128 and the Adam optimizer with an initial learning rate of $10^{-3}$. We multiply the learning rate by a factor of $0.24$ after 5000 and 10000 epochs. When training a \ac{nf} absent of the SoftFlow framework we add noise of the magnitude 0.02 to the data. When training with the SoftFlow framework, we follow the original implementation~\cite{kim2020softflow} and use a maximum noise standard deviation of 0.075 and a minimum noise standard deviation of 0.0.

\paragraph{General experiments on autoencoding} in \secref{subsection:pc_autoencoding}. We train the RealNVP for 1500 epochs using a batch size of 128 and the Adam optimizer with an initial learning rate of $6.4\times 10^{-4}$ which we multiply with 0.25 after 1200 and 1400 epochs. Additionally, we vary the magnitude of noise added to the point clouds over the process of the training. Initially, we train with a Gaussian noise of standard deviation $\sigma=0.25$ for the first 100 epochs. Then, we exponentially decay the standard deviation of the noise to $\sigma=0.02$ between epoch 100 and epoch 1200. Afterwards we fix $\sigma=0.02$.
