# Supplementary material for: ManiFlow: Implicitly Representing Manifolds with Normalizing Flows
Source: arXiv:2208.08932 source file (2022-08-18)
Supplement: Supplementary file 10 [file proof.tex]

We now prove assumptions about the log-likelihood of \acp{nf} made in \secref{subsection:sampling_manifold}. 
Let $\Omega$ denote a m-dimensional compact manifold embedded in n-dimensional Euclidean space, $\Omega \in \mathbb{R}^n$ where $m<n$. Let further $X$/$S$ refer to a random variables with their corresponding probability density $P_X$/$P_S$ and $x\sim P_X(x)$, resp. $s\sim P_S(s)$, realizations of these random variables. Moreover, let $S$ exist on the m-dimensional manifold $\Omega$ such that $P_S(x) = 0$ $\forall x \notin \Omega$.
Assuming that $S$ is locally well approximated by a m-dimensional hypersphere with radius $r\gg \sigma$ and that $P_S$ is approximately uniform on this hypersphere, we show that i) the gradient of the log-likelihood $\log(P_X)$ is perpendicular to $S$ and ii) that $P_X$ has a maximum on $S$.  

To this end, we will consider one sample $x\sim P_X$ and approximate $P_S$ in its neighborhood using the aforementioned hypersphere L and multivariate Gaussian noise with a covariance matrix $\Sigma = \sigma^2 I$.
\begin{align}
    P_X(x) &= \int_{\mathbb{R}^n} P_N(x-s)P_S(s) ds \nonumber\\
    &= \int_{\mathbb{R}^n} P_N(x-s)p_0\delta(f_{imp}(s)) ds \\
    &\approx \frac{p_0}{(2\pi \sigma^2)^{\frac{n}{2}}}\int_{L} \exp\left(  \frac{\sum_{i+1}^{n} (x - l)^2}{\sigma^{2n}}\right) dl \nonumber
\end{align}
where we have used $P_S(s) = p_0\delta(f_{imp}(s))$. $p_0$ is the local probability density, $\delta(x)$ the delta function and $f_{imp}(s)$ an implicit representation of $\Omega$ that is zero on $\Omega$. Thus, we are integrating the noise distribution over the hypersphere. Without loss of generality let us assume that L is zero-centered and axis aligned - i.e. n-m basis vectors of the n-dimensional space are perpendicular to L. Now let $M = \{ i_1, \dots, i_k \}$ denote the set of basis vectors that are parallel to L, then we have 
\begin{align}
\begin{split}
    P_X(x) \approx & \frac{p_0}{(2\pi \sigma^2)^{\frac{n}{2}}} \exp\left(  \frac{\sum_{i\not\in M} x_i^2}{\sigma^{2n}}\right) \\ &\int_{L} \exp\left(  \frac{\sum_{i\in M} (x_i - l_i)^2}{\sigma^{2n}}\right) dx_{i_1}\dots dx_{i_k}
\end{split}
\end{align}
Thus, we only integrate over the axis that are aligned with the hypersphere. Given that $r\gg \sigma$ and knowledge about the solution of the Gaussian integral, the integral approximately evaluates to $\int_{L} \exp\left(  \frac{\sum_{i\in M} (x_i - l_i)^2}{\sigma^{2n}}\right) dx_{i_1}\dots dx_{i_k} \approx (2\pi \sigma^2)^{\frac{m}{2}}$ for x close to the origin. Consequently, we can locally approximate $P_X$ with (d-m)-dimensional Gaussian distribution that is invariant to changes along basis vectors in $M$:
\begin{equation}
    P_X(x) \approx \frac{p_0}{(2\pi \sigma^2)^{\frac{n-m}{2}}} \exp\left(  \frac{\sum_{i\not\in M} x_i^2}{\sigma^{2n}}\right)
\end{equation}
From this we can see that $P_X$ approximately fulfills i) and ii).
