# Supplementary material for: ManiFlow: Implicitly Representing Manifolds with Normalizing Flows
Source: arXiv:2208.08932 source file (2022-08-18)
Supplement: Supplementary file 11 [file qualitative_meshes.tex]

Poisson surface reconstruction in LL-Poisson extracts a mesh of the 3D shape from the \ac{nf}'s log-likelihood. We provide qualitative examples of these meshes in \figref{fig:ll_poisson_meshes}. Note that these meshes correspond to the point clouds visualized in \figref{fig:airplane_supplement}, \figref{fig:car_supplement} and \figref{fig:chair_supplement}.

\begin{figure*}[b]
\begin{center}

    \renewcommand{\figsize}{0.15}
    
    \begin{tabular}{ c c c }
    \setlength{\tabcolsep}{0pt} % Default value: 6pt
     % Default value: 1
    
        \centering 
      
      \includegraphics[width=\figsize\linewidth]{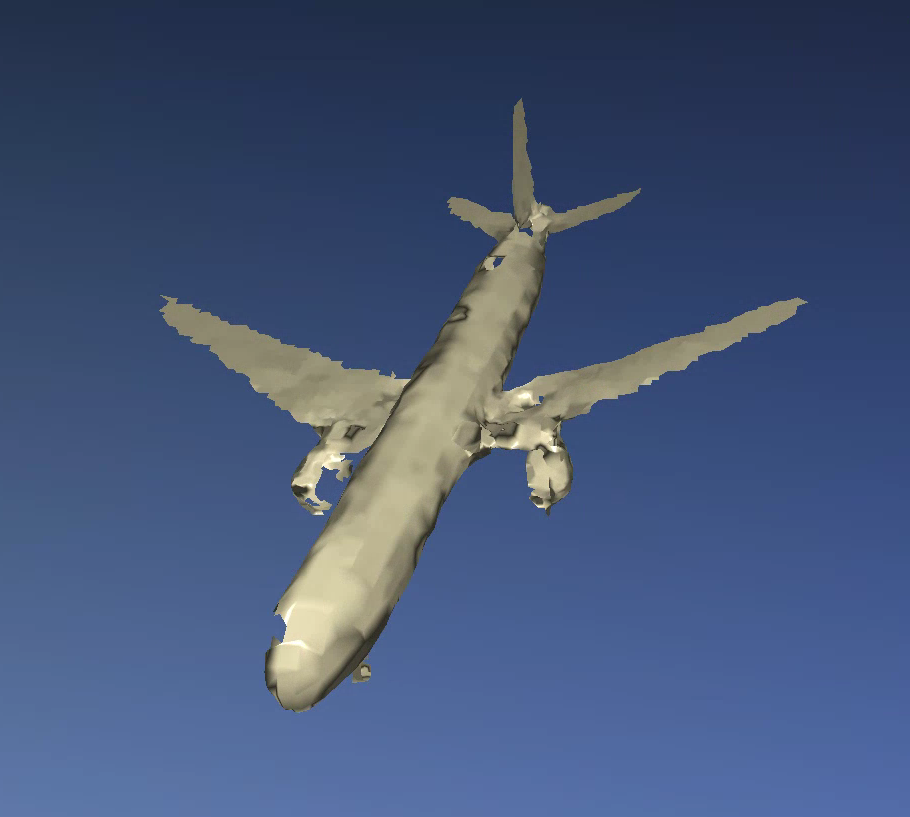} &
      \includegraphics[width=\figsize\linewidth]{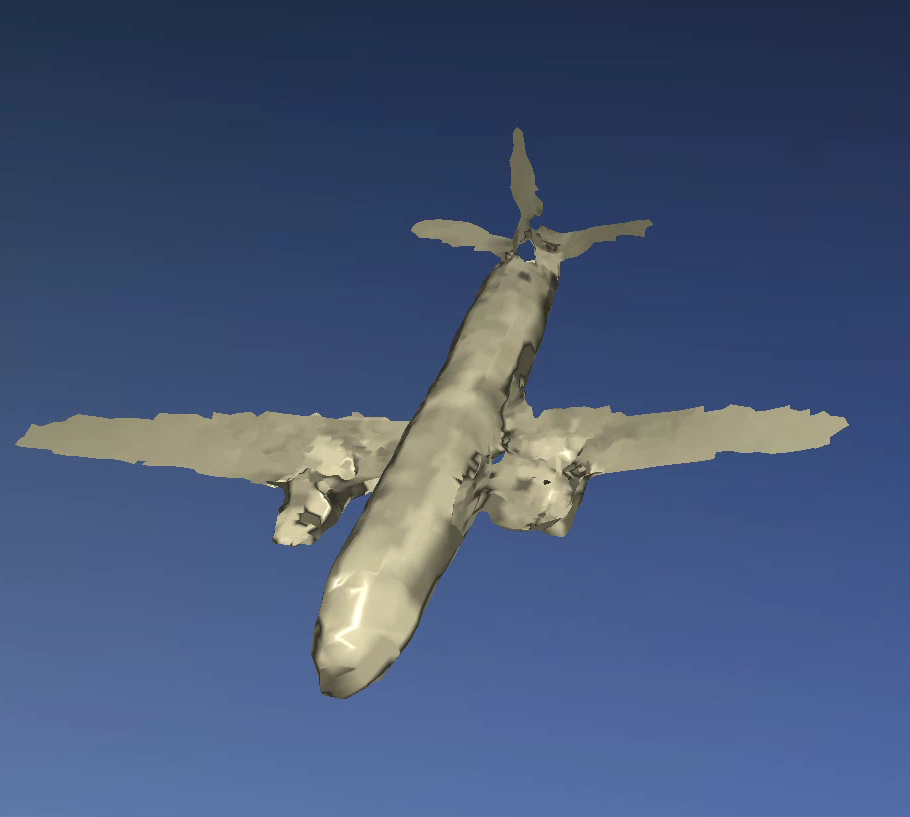} &
      \includegraphics[width=\figsize\linewidth]{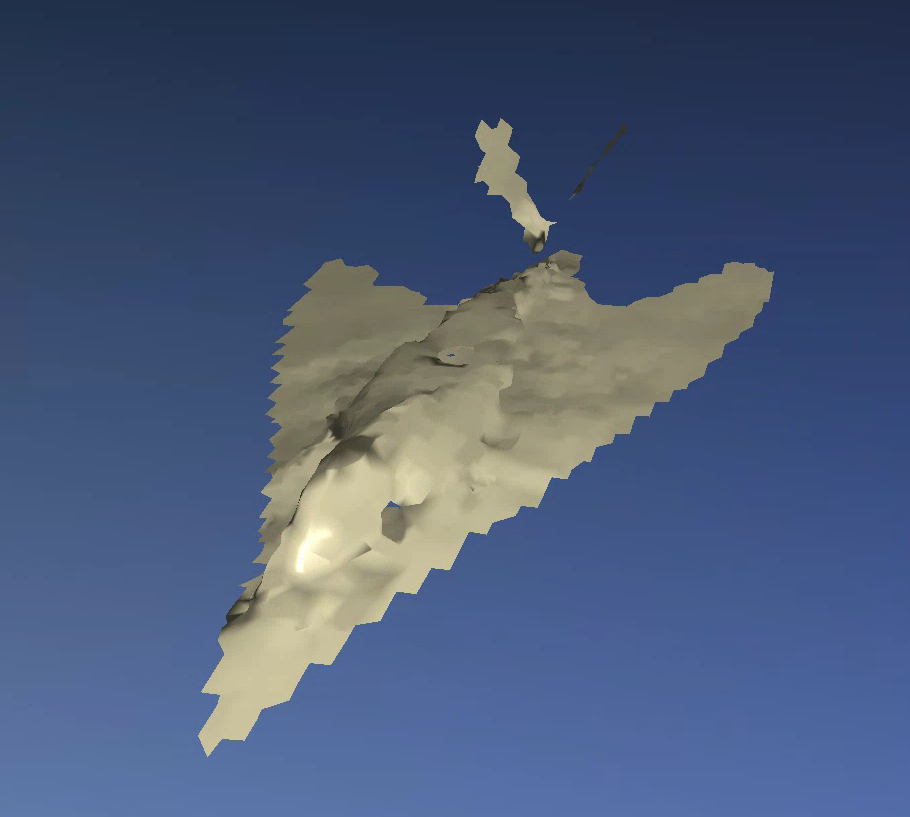} \\
      
      \includegraphics[width=\figsize\linewidth]{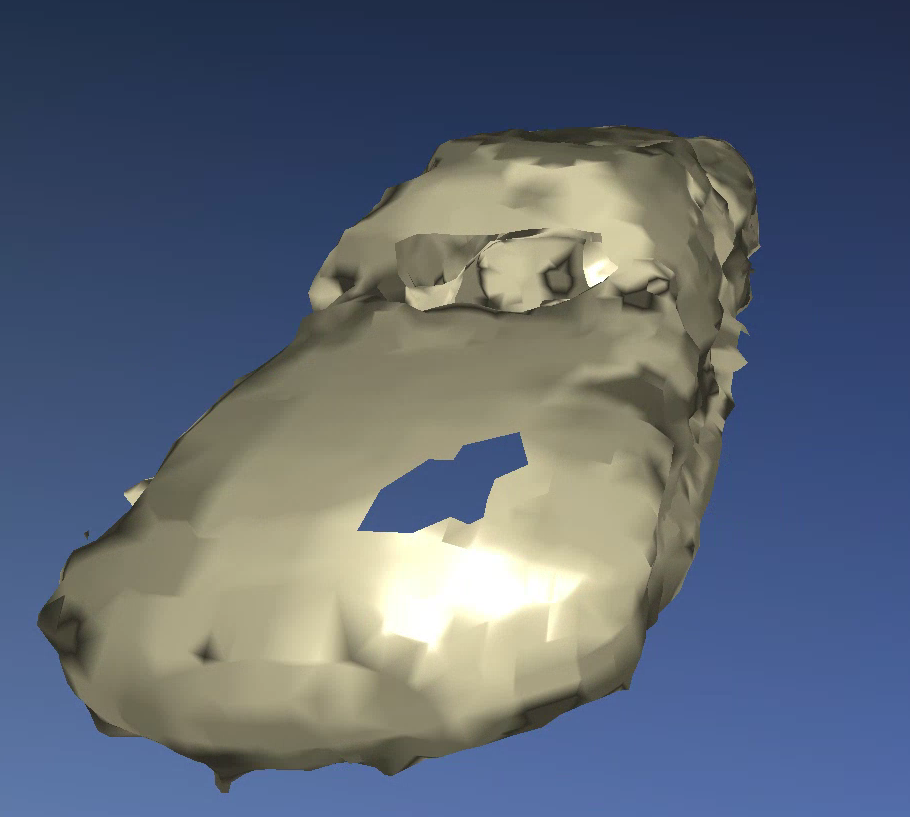} &
      \includegraphics[width=\figsize\linewidth]{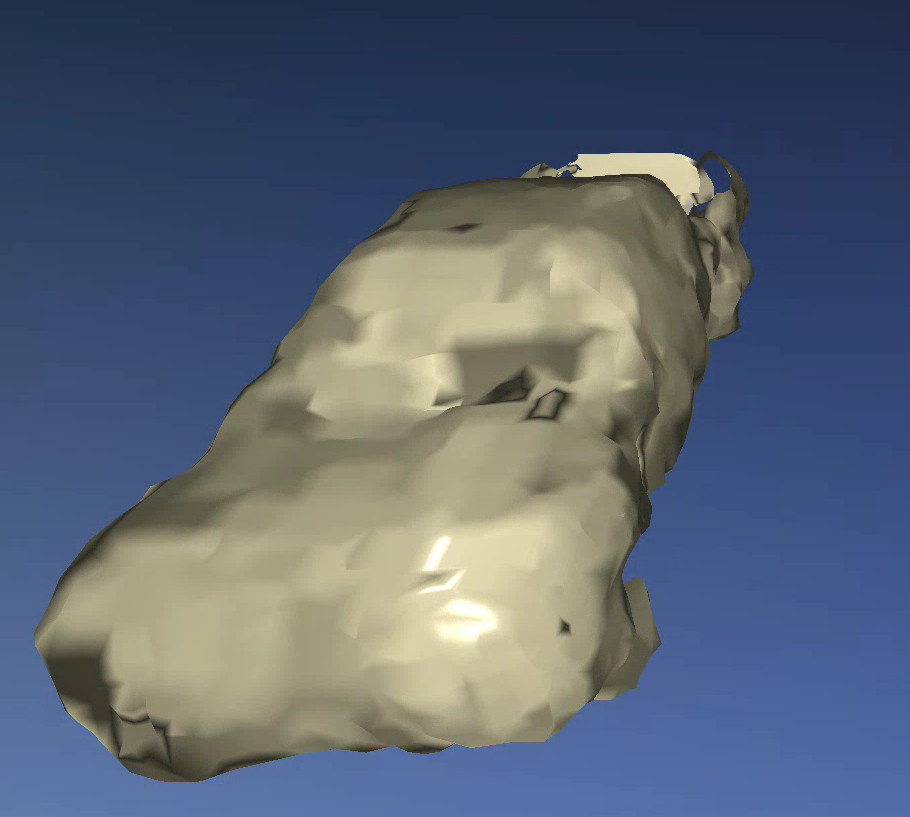} &
      \includegraphics[width=\figsize\linewidth]{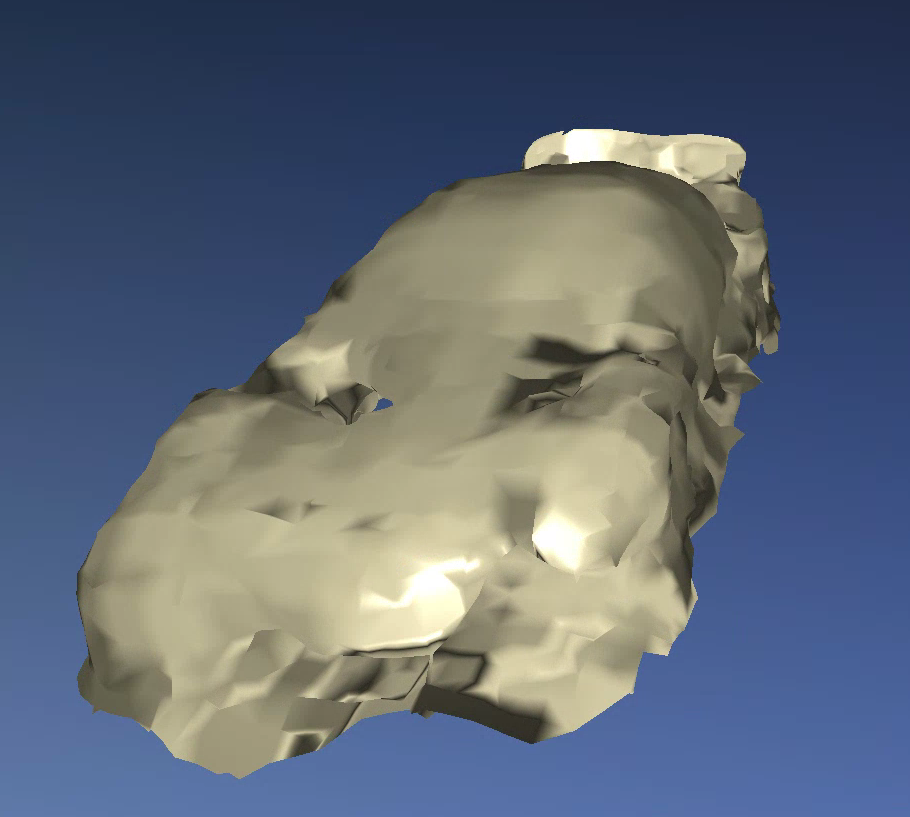} \\
      
      \includegraphics[width=\figsize\linewidth]{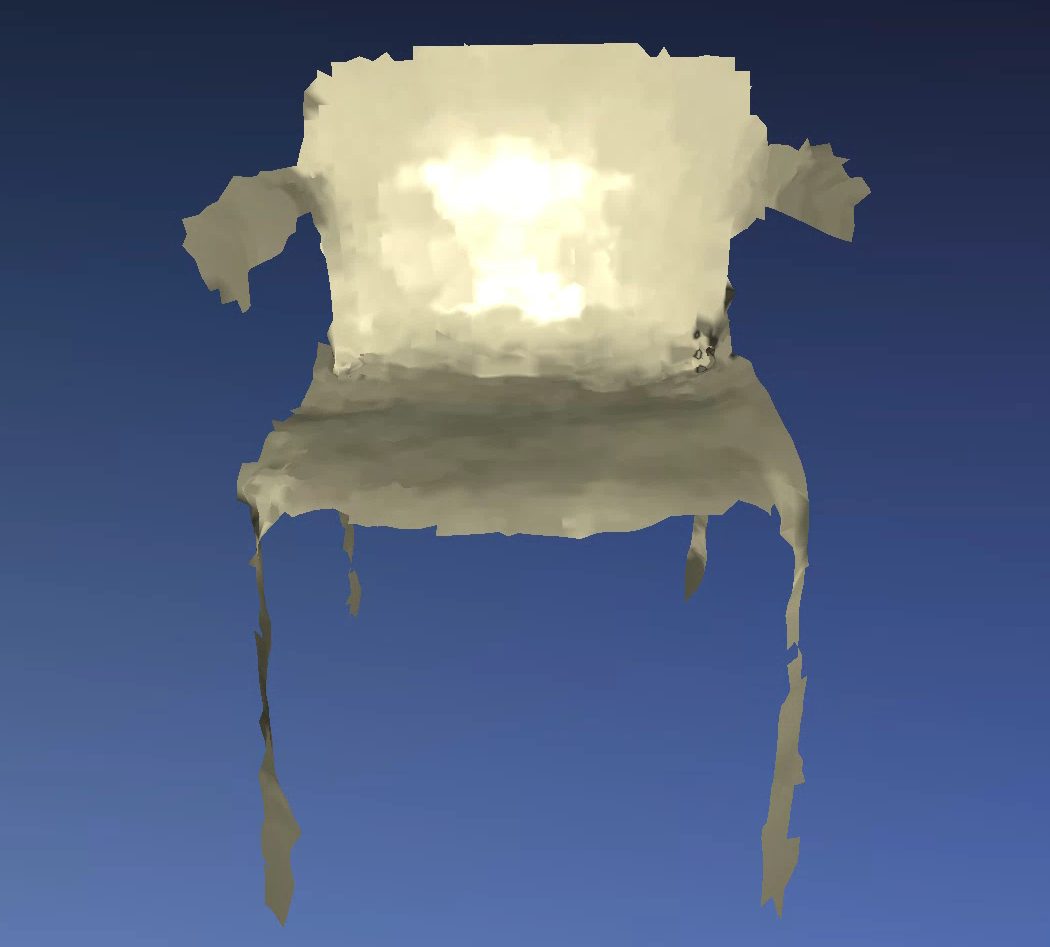} &
      \includegraphics[width=\figsize\linewidth]{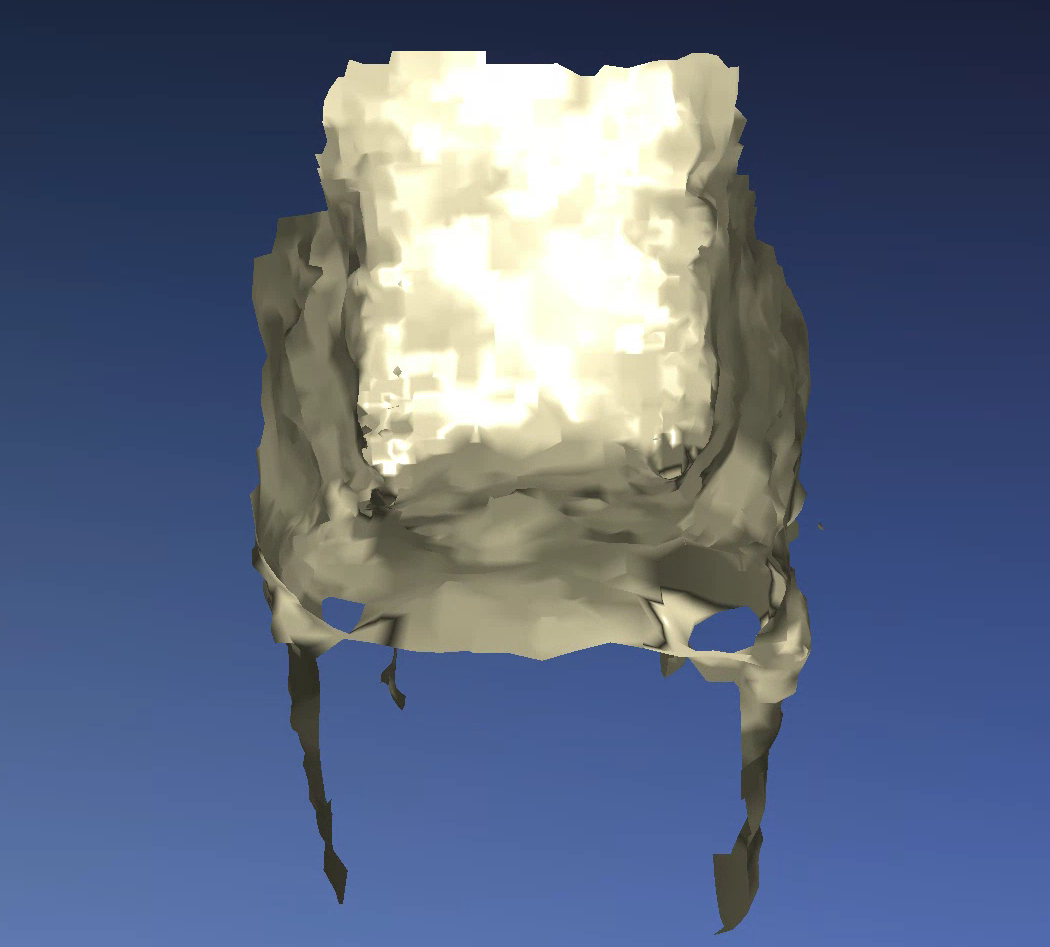} &
      \includegraphics[width=\figsize\linewidth]{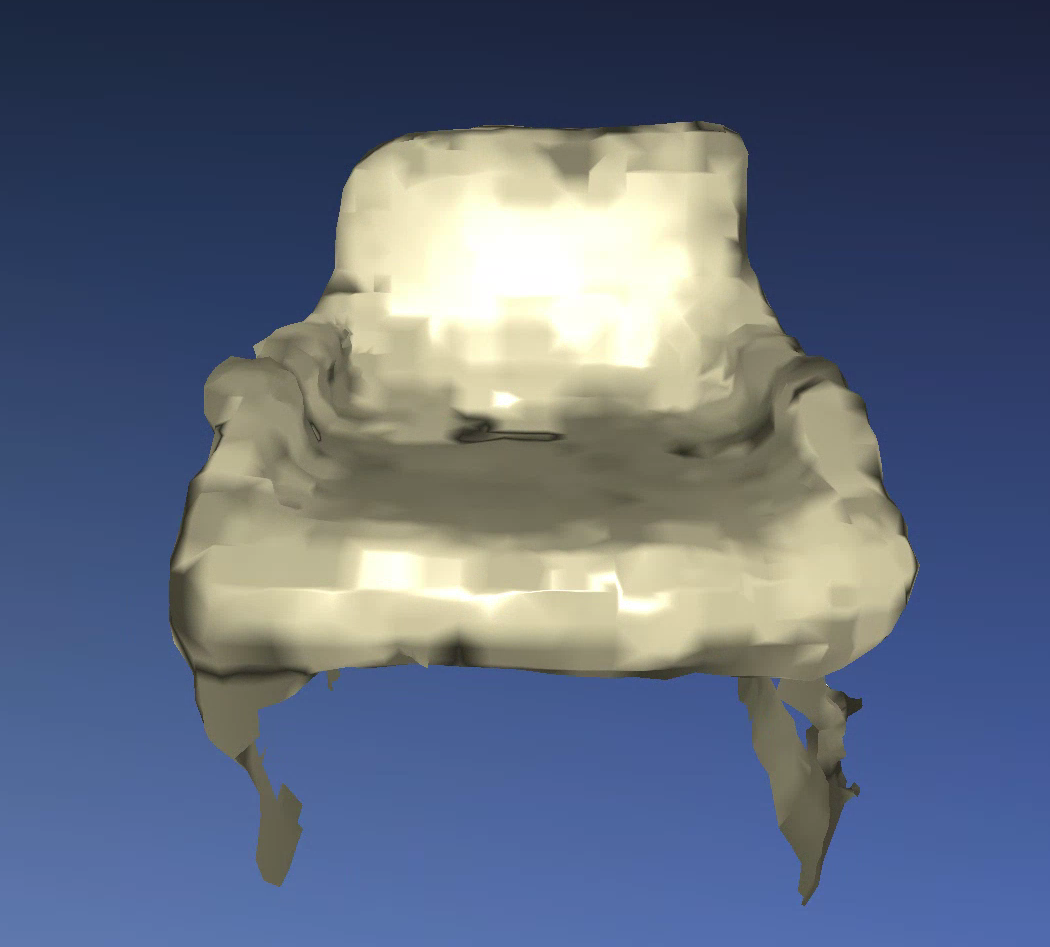} \\
      
    \end{tabular}
    
\end{center}
\caption{Qualitative examples of meshes created with LL-Poisson on the categories airplane, car and chair.}\label{fig:ll_poisson_meshes}
\end{figure*}
