# Supplementary material for: ManiFlow: Implicitly Representing Manifolds with Normalizing Flows
Source: arXiv:2208.08932 source file (2022-08-18)
Supplement: Supplementary file 13 [file toy_examples.tex]

We provide an additional experiment on artificial data showing the importance of setting $\lambda>0$ in \eref{eq:optimization_criterion}. To this end, we train a \ac{nf} on a non-uniform distribution on a 1D sine curve embedded in 2D space. After training, we recover the manifold using ManiFlow - LLM using $\lambda=0.0$ and $\lambda=0.2$. The results are in \figref{fig:toy_example_regularization}. We observe that $\lambda=0.0$ fails to recover the true distribution on the manifold since generated points collapse towards global peaks of the distribution parameterized by the \ac{nf}.
